# Supplementary material for: Quantum Many-Body Physics Calculations with Large Language Models
Source: arXiv:2403.03154 source file (2024-08-22)
Supplement: Supplementary file 1 [file SM.pdf]

# Supplemental material for "Many-Body Physics Calculations with Large Language Models"

Haining Pan,[1] Nayantara Mudur,[2,3] Will Taranto,[1] Maria Tikhanovskaya,[2,3] Subhashini Venugopalan,[2] Yasaman Bahri,[4] Michael P. Brenner,[2,3,5] and Eun-Ah Kim[1,2,6]

[1] *Department of Physics, Cornell University, Ithaca, NY, USA*
[2] *Google Research, Mountain View, CA 94043*
[3] *Department of Physics, Harvard University, Cambridge, MA, USA*
[4] *Google DeepMind, Mountain View, CA 94043*
[5] *School of Engineering and Applied Sciences, Harvard University, Cambridge, MA, USA*
[6] *Department of Physics, Ewha Womans University, Seoul, South Korea*

**Contents**

A. The general structure of HF calculation 2
  1. Analytical Derivation of the Hartree-Fock Hamiltonian $H_{HF}$ 2
  2. Numerical solution to the matrix self-consistency equations 3

B. Choice of papers 3

C. Design of templates 4
  1. Branches 4
  2. Paradigm of divide-and-conquer 5
  3. Contents of prompt templates 5
  4. The generic workflow for three branches 23

D. API Execution for Annotated-Excerpt based execution 24

E. Abstract-based Execution 25

F. Code 50

G. Example of spotting a typo 50

H. One-shot prompting for extraction 51

I. Automatic Evaluation 52
  1. Zero-Shot 52
  2. Few (2)-Shot with Rationale 53

References 60

### A. The general structure of HF calculation

#### 1. Analytical Derivation of the Hartree-Fock Hamiltonian $H_{HF}$

The HF calculation can ultimately be reduced to solving a single-particle problem numerically. While the HF calculation sometimes is analytically solvable, e.g., BCS theory and Stoner ferromagnetism, (e.g., for Stoner ferromagnetism, we have $H_{int}^{HF} = U\sum_i \left[n_{\uparrow,i}\langle n_{\downarrow,i}\rangle + n_{\downarrow,i}\langle n_{\uparrow,i}\rangle - \langle n_{\downarrow,i}\rangle\langle n_{\uparrow,i}\rangle\right]$) real materials often manifest great complexity due to the presence of multiple flavors (degrees of freedom). Therefore, the single-particle HF Hamiltonian could become a matrix with the dimension of the product of all local degrees of freedom for each flavor ($\prod_{i=1}^{n} d_i$), e.g., $d = 2$ for electron spin flavors. This necessitates numerical methods for diagonalizing the HF Hamiltonian. In addition to the presence of multiple flavors, the breaking of translational symmetry can introduce another degree of freedom corresponding to the reduced reciprocal lattice vector, paving the way for charge-density waves (CDW) and spin-density waves (SDW). This is likely to arise from the Fermi surface nesting in the non-interacting term or be inferred from experimental observation of extra peaks inside the Brillouin zone (BZ) in the x-ray diffraction pattern.

As the system contains more types of flavors, brute force numerical diagonalization becomes increasingly difficult. Thus, taking the system's symmetry into account can greatly alleviate the numerical challenge. Different systems, characterized by their unique dispersions and interactions, exhibit distinct symmetries affecting the matrix elements of the final single-particle HF Hamiltonian. If interactions are restricted to specific flavors, this constraint introduces an effective symmetry charge, leading to the block-diagonalization of the final HF Hamiltonian within sectors that respect this symmetry. Another example is that if the interaction lacks SU(n) symmetry in a flavor, where $n$ represents the number of possible states for a given flavor, then the resulting HF Hamiltonian will reflect this anisotropy. In 1106.6060, we show that the interaction is anisotropic within the orbital flavor.

In principle, one can construct the system entirely from numerics in the very beginning by considering all possible coupling combinations in flavors. However, as will be demonstrated, this approach lacks efficiency. Thus, one needs to work out a certain amount of analytical derivations before invoking numerical solvers. (Ideally, one should relegate only the absolute necessary calculations to the numerical solver). Therefore, by deriving analytical insights into the distribution of each matrix element of $H_{HF}$, we can gain several advantages:

(1) Time Complexity Advantages: In numerical methods, analytical pre-computing reduces the computational burden on numerical solvers, enabling its handling of larger-scale problems. Specifically, the direct diagonalization of the matrix considering all combinations of different flavors involves a time complexity of $\prod_{i=1}^{n} d_i^3$ (the time complexity of diagonalizing a $n \times n$ matrix is $\mathcal{O}(n^3)$, whilst, the block diagonalization within each symmetry sector, enabled by the analytical calculation, needs only the diagonalization of $d_1$ smaller matrices, each of dimension $\prod_{i=2}^{n} d_i$, offering a speed-up by a factor of $d_1^2$.

(2) Physical understanding. Physicists seek not only to identify the ground state of a system under certain parameters regime but also to understand the underlying reasons for the formation of specific phases. Analytical calculations elucidate the connection between the system's symmetry and the symmetry of $H_{HF}$, thereby predicting the potential eigenstates respecting this symmetry. Without preliminary analytical analysis, relying solely on numerical solvers obscures the physical insights, making it challenging to comprehend why a particular state emerges as the ground state. Analytical frameworks, therefore, are crucial for establishing a deeper physical understanding that goes beyond numerical outcomes.

### 2. Numerical solution to the matrix self-consistency equations

In the example in Fig. 1. [1], we consider the several candidate phases indicated by different choices of the order parameter, namely, the finite value of $\left\langle c^{\dagger}_{k_\alpha,l_\alpha,\tau_\alpha} c_{k_\alpha,l_\beta,\tau_\beta} \right\rangle$, where $k$, $l$, and $\tau$ represent the momentum, layer (top and bottom), and valley (K and K') valley. To obtain a valley polarized state at a filling factor of 1 (one hole per moiré unit cell), we set $\tau_\alpha = \tau_\beta$, implying $\left\langle c^{\dagger}_{k_\alpha,l_\alpha,K} c_{k_\alpha,l_\beta,K} \right\rangle > 0$ ($K'$ is another spontaneous symmetry breaking state which can be related by time-reversal symmetry) and all rest is zero. For an intervalley coherent state, we enforce $\tau_\alpha \neq \tau_\beta$, with both $\left\langle c^{\dagger}_{k_\alpha,l_\alpha,K} c_{k_\alpha,l_\beta,K'} \right\rangle > 0$ and $\left\langle c^{\dagger}_{k_\alpha,l_\alpha,K'} c_{k_\alpha,l_\beta,K} \right\rangle > 0$. Additionally, for states with translational symmetry breaking, e.g., spin density waves, involves decomposing momentum $k$ into $Q$ (within the reduced Brillouin zone of the extended moiré unit cell) and $q$ (the reciprocal lattice vector), where $k = Q + q$, introducing a fourth index $q$ that represents the reduced Brillouin zone's reciprocal lattice vectors, adding complexity to order parameters. For instance, a spin density wave with $\sqrt{3} \times \sqrt{3}$ periodicity on a triangular lattice implies $N = 3$ for the enlarged unit cell multiple. After solving self-consistent equations for each state and comparing their energies upon convergence, we identify the ground state and propose a phase diagram based on various parameters. The analysis of this part is left for future work, and our current focus is to reach the end of HF Hamiltonian.

## B. Choice of papers

To construct the paper database, we downloaded arXiv paper dataset from [2] provided by Cornell University, selecting papers published between January 2010 and August 2023, totaling 1841366 documents. Our focus narrowed to the 'cond-mat' category, excluding 'cond-mat.soft' and 'cond-mat.stat-mech', resulting in 187,460 papers. Given our interest in Hartree-Fock-related research, we further refined our selection to include papers mentioning 'Hartree', 'Fock', or 'Mean-field' in their abstracts, yielding 6456 papers. To concentrate on fermionic systems, we excluded papers with 'bosons' in the abstract, reducing the count to 4,901. Aiming for a minimal yet representative template, we focused on normal order parameters, excluding terms like 'superconducting' and 'quantum spin liquid', which led to 3722 papers. Additionally, we excluded papers employing dynamical mean-field theory (DMFT), density functional theory (DFT), Quantum Monte Carlo (QMC), and renormalization group (RG) methods, further narrowing the selection to 2234 papers. Ultimately, we chose papers published in Physical Review Letters (PRL), Physical Review B (PRB), and Physical Review X (PRX), finalizing our database at 807 papers.

After analyzing the last authorship of the selected papers, we identified the top 3 authors are: *Allan H. MacDonald* (10 papers), *Sankar Das Sarma* (9 papers), and *Yukitoshi Motome* (6 papers). We selected representative papers from these authors and supplemented our selection with recent contributions from other researchers. Our curated collection encompasses papers published after gpt-4-0613's training data cutoff in September 2021, including two papers posted on arXiv even after June 13th, 2023—the snapshot date for gpt-4-0613. The inclusion of papers posted after both dates helps us investigate whether the LLM is merely recalling information it might have already seen during training or generating novel insights.

## C. Design of templates

### 1. Branches

To manage the diversity of conventions used across different papers for identical physical quantities, we developed distinct versions of prompt templates tailored to each paper's specific notations while ensuring consistency in content. This approach avoids the complexity and inefficiency of incorporating 'if-else' branches within a single template, which would introduce irrelevant information for specific tasks. For example, the Fourier transform that brings a Hamiltonian in the real space to the momentum space has two versions– 'continuum' and 'lattice', which are used to handle the continuum system and lattice system, respectively. Another dichotomy is in the basis of the Hamiltonian, which can be either in 'the first quantized basis' or 'the second quantized basis'. In total, we have three types as shown in Fig. 1(d) and (f) — (lattice, second quantized), (continuum, second-quantized), and (continuum, first-quantized). ('lattice, first quantized' is rare and we encountered no papers employing this convention). For each branch, we design a workflow of prompt templates. Therefore, when processing a new paper, our methodology begins by identifying the branch, and then streamlining the prompt templates in that branch. The results are shown in Table I.

TABLE I: The branch of the paper

| arXiv number | Branch |
|---|---|
| 1010.1819 [3] | continuum, first-quantized |
| 1106.6060 [4] | lattice, second-quantized |
| 1208.0116 [5] | continuum, first-quantized |
| 1310.2674 [6] | lattice, second-quantized |
| 1508.00296 [7] | lattice, second-quantized |
| 1812.04213 [8] | lattice, second-quantize |
| 2004.04168 [9] | lattice, second-quantized |
| 2008.08998 [10] | lattice, second-quantized |
| 2012.04554 [11] | lattice, second-quantized |
| 2108.02159 [12] | continuum, second-quantized |
| 2110.11330 [13] | lattice, second-quantized |
| 2111.01152 [1] | continuum, first-quantized |
| 2112.07523 [14] | continuum, second-quantized |
| 2308.03843 [15] | lattice, second-quantized |
| 2308.07488 [16] | continuum, first-quantized |

Figures 1(d) and (f) assess the performance of both execution and extraction stages across three distinct branches, revealing no substantial differences among them. This uniformity confirms that the outcomes are not influenced by the specific conventions utilized within the papers.

Figure 1(a) provides a detailed evaluation of all tasks during the execution stage, expanding on the summary provided in Figure 4(d) of the main text, which categorizes tasks into five steps. Similarly, Figure 1(e) details task performance in the extraction stage.

Despite efforts to tailor the prompt template closely to each paper, certain tasks in some papers do not fit perfectly into the template. Figure 1(b) estimates the fitness of the prompt template for various tasks, showing that over 90% of tasks across all papers fit well with the templates. However, about 10% of tasks roughly fit the template but lack some details, e.g., the meaning of the variable is not unambiguously defined. For example, $\kappa_\pm$ in [2308] is misunderstood as the

momentum shift at $K/K^{'}$ valley, despite, it is the shift on each layer. and less than 5% of tasks, such as interaction involving Hund's coupling [6], do not match the template designed for density-density interaction terms. Consequently, Figure 1(c) correlates template suitability with execution performance, indicating that a good fit between the task and the template significantly enhances result accuracy.

### 2. Paradigm of divide-and-conquer

The prompt template's design during the execution stage adopts a divide-and-conquer strategy, where we segment the required tasks into various subproblems for the LLM to address. If the LLM fails to provide an accurate solution, the task is further divided into smaller, more manageable subproblems until the LLM can resolve each component. This approach, combined with an understanding of what constitutes an "atomic" task (the smallest unit of task that is meaningful in a physical context), allows us to organize the entire procedure into five steps, as depicted in Fig. 2 of the main text, with each step comprising 2-4 specific tasks. It is important to note that our template design is neither the unique nor the most efficient approach; it simply represents a feasible method. Theoretically, alternate templates could be developed to perform similar analyses, offering flexibility in template design and the potential to adapt this methodology for various other problems.

### 3. Contents of prompt templates

```
Identify kinetic term (continuum,first-quantized)
**Prompt:**
You will be instructed to describe the kinetic term of Hamiltonian in {
system} in the {real|momentum} space in the {single-particle|second-
quantized} form.
The degrees of freedom of the system are: {degrees_of_freedom}.
Express the Kinetic Hamiltonian {kinetic_symbol} using {variable} which
are only on the diagonal terms, and arrange the basis in the order of {
order}. [Note that the sublattice degrees of freedom is suppressed for
now and will be stated later]

Use the following conventions for the symbols:
{definition_of_variables}
```

```
Identify kinetic term (continuum,second-quantized)
**Prompt:**
You will be instructed to describe the kinetic term of Hamiltonian in {
system} in the {real|momentum} space in the {single-particle|second-
quantized} form.
The degrees of freedom of the system are: {degrees_of_freedom}.
Express the Kinetic Hamiltonian {kinetic_symbol} using {
dispersion_symbol}, {annihilation_op}, and {creation_op}, where the
summation of ${k|r}$ should be running over the {entire_space|
```

```
first_Brillouin_zone}.

Use the following conventions for the symbols:
{definition_of_variables}
```

```
Identify kinetic term (lattice)
**Prompt:**
You will be instructed to describe the kinetic term of Hamiltonian in {
system} in the {real|momentum} space in the {single-particle|second-
quantized} form.
The degrees of freedom of the system are: {degrees_of_freedom}
The kinetic term is a tight-binding model composed of the following
hopping process:
{site i and site j with the amplitude hopping}
[You should ensure the hermiticity of the Hamiltonian]
The summation should be taken over all {degrees_of_freedom} and all {
real|momentum} space positions.
Return the Kinetic Hamiltonian {kinetic_symbol}.

Use the following conventions for the symbols:
{definition_of_variables}
```

```
Define energy dispersion (continuum)
**Prompt:**
You will be instructed to construct each term, namely {Energy_dispersion
}.
For all energy dispersions, {Energy_dispersion}, it characterizes the {
parabolic|Dirac|cos} dispersion for {electrons|holes}.
[In addition, a shift of {momentum_shift} in the momentum ${k_symbol}$
for {shifted_Ek}, respectively.]
You should follow the EXAMPLE below to obtain the correct energy
dispersion, select the correct EXAMPLE by noticing the type of
dispersion.
Finally, in the real space, the momentum ${k_symbol}=-i \partial_{{{
r_symbol}}}$. You should keep the form of ${k_symbol}$ in the
Hamiltonian for short notations but should remember ${k_symbol}$ is an
operator.
You should recall that {expression_kinetic}.
Return the expression for {Energy_dispersion} in the Kinetic Hamiltonian
, and substitute it into the Kinetic Hamiltonian {kinetic_symbol}.

Use the following conventions for the symbols (You should also obey the
conventions in all my previous prompts if you encounter undefined
symbols. If you find it is never defined or has conflicts in the
conventions, you should stop and let me know):
{definition_of_variables}

===
EXAMPLE 1:
```

```
A parabolic dispersion for electron is $E_{{\alpha}}=\frac{{\hbar^2 k
^2}}{{2m_{{\alpha}}}}$, where $\alpha$ indicates the type of electron.
If there is a further shift of $q$ in the momentum $k$, the dispersion
will become $E_{{\alpha}}=\frac{{\hbar^2 (k-q)^2}}{{2m_{{\alpha}}}}$.

EXAMPLE 2:
A cos dispersion is $E_{{\alpha}}=-\cos(k a / 2)$, where $\alpha$
indicates the type of particle.  If there is a further shift of $q$ in
the momentum $k$, the dispersion will become $E_{{\alpha}}=-\cos((k-q) a
 / 2))$. However, there could be more prefactors before cos depending on
 the geometry of the lattice.

EXAMPLE 3:
A dirac dispersion for electron/hole is a 2 by 2 matrix, i.e., $h_{{\
theta}}(k)=-\hbar v_D |k| \begin{{pmatrix}}  0 & e^{{i(\theta_{{k}}-\
theta)}}\\ e^{{-i(\theta_{{\bar{{k}}}}-\theta)}} & 0 \end{{pmatrix}}$,
where $v_D$ is the Fermi velocity, $\theta$ is the twist angle, and $\
theta_k$ indicates the azumith angle of $k$. If there is a further shift
 of $K_{{\theta}}$ in the momentum $k$, the dispersion will become $h_
{{\theta}}(k)=-\hbar v_D |k-K_{{\theta}}| \begin{{pmatrix}}  0 & e^{{i(\
theta_{{k-K_{{\theta}}}}-\theta)}}\\ e^{{-i(\theta_{{k-K_{{\theta}}}}-\
theta)}} & 0 \end{{pmatrix}}$.
```

```
Identify potential term (continuum)
**Prompt:**
You will be instructed to describe the potential term of Hamiltonian {
potential_symbol} in the {real|momentum} space in the {single-particle|
second-quantized} form.
The potential Hamiltonian has the same degrees of freedom as the kinetic
 Hamiltonian.
The diagonal terms are {diagonal_potential}.
The off-diagonal terms are the coupling between {
potential_degrees_of_freedom}, {offdiagonal_potential}, which should be
kept hermitian.
All other terms are zero.
Express the potential Hamiltonian {potential_symbol} using {
diagonal_potential} and {offdiagonal_potential}.

Use the following conventions for the symbols (You should also obey the
conventions in all my previous prompts if you encounter undefined
symbols. If you find it is never defined or has conflicts in the
conventions, you should stop and let me know):
{definition_of_variables}
```

```
Define potential term (continuum)
**Prompt:**
You will be instructed to construct each term {potential_symbol}, namely
, {Potential_variables}.
The expression for diagonal terms are: {expression_diag}.
The expression for off-diagonal terms are: {expression_offdiag}.
```

```
You should recall that {expression_Potential}.
Return the expressions for {Potential_variables}, and substitute it into
 the potential Hamiltonian {potential_symbol}.

Use the following conventions for the symbols (You should also obey the
conventions in all my previous prompts if you encounter undefined
symbols. If you find it is never defined or has conflicts in the
conventions, you should stop and let me know):
{definition_of_variables}
```

```
Identify interacting term (real space)
**Prompt:**
You will be instructed to construct the interaction part of the
Hamiltonian, {second_int_symbol} in the real space in the second-
quantized form.
The interacting Hamiltonian has the same degrees of freedom as the
kinetic Hamiltonian {kinetic_symbol}.
The interaction is a density-density interaction composed of the
following process:
{site i and site j with the interaction strength}
The summation should be taken over all {degrees_of_freedom} and all real
 space positions.
Return the interaction term {second_int_symbol} in terms of {
density_symbol}.

Use the following conventions for the symbols (You should also obey the
conventions in all my previous prompts if you encounter undefined
symbols. If you find it is never defined or has conflicts in the
conventions, you should stop and let me know):
{definition_of_variables}
```

```
Identify interacting term (momentum space)
**Prompt:**
You will be instructed to construct the interaction part of the
Hamiltonian {second_int_symbol} in the momentum space.
The interaction Hamiltonian is a product of four parts.
The first part is the product of four operators with two creation and
two annihilation operators following the normal order, namely, creation
operators are before annihilation operators. You should follow the order
 of $1,2,2,1$ for the {index_of_operator}, and $1,2,3,4$ for the {
momentum}.
The second part is the constraint of total momentum conservation, namely
 the total momentum of all creation operators should be the same as that
 of all annihilation operators. [For each operator, the total momentum
is the sum of moire reciprocal lattice $b_i$ and momentum with in the
first BZ $k_i$]
The third part is the interaction form. You should use {interaction}
with $V(q)={int_form}$, where $q$ is the transferred total momentum
between a creation operator and an annihilation operator with the same {
index_of_operator}, namely $q=k_1-k_4$.
```

```
The fourth part is the normalization factor, you should use {
normalization_factor} here.
Finally, the summation should be running over all {index_of_operator},
and {momentum}
Return the interaction term {second_int_symbol} in terms of {op} and $V(
q)$ (with $q$ expressed in terms of {momentum}).

Use the following conventions for the symbols (You should also obey the
conventions in all my previous prompts if you encounter undefined
symbols. If you find it is never defined or has conflicts in the
conventions, you should stop and let me know):
{definition_of_variables}
```

```
Second-quantization (matrix)
**Prompt:**
You will be instructed to construct the second quantized form of the
total noninteracting Hamiltonian in the {real|momentum} space.
The noninteracting Hamiltonian in the {real|momentum} space {
nonint_symbol} is the sum of Kinetic Hamiltonian {kinetic_symbol} and
Potential Hamiltonian {potential_symbol}.
To construct the second quantized form of a Hamiltonian. You should
construct the creation and annihilation operators from the basis
explicitly. You should follow the EXAMPLE below to convert a Hamiltonian
 from the single-particle form to second-quantized form.
Finally by "total", it means you need to take a summation over the {real
|momentum} space position {$r$|$k$}.
Return the second quantized form of the total noninteracting Hamiltonian
 {second_nonint_symbol}

Use the following conventions for the symbols (You should also obey the
conventions in all my previous prompts if you encounter undefined
symbols. If you find it is never defined or has conflicts in the
conventions, you should stop and let me know):
{definition_of_variables}

===
EXAMPLE:
For a Hamiltonian $H$, where $H=\begin{{pmatrix}} H_{{a,a}} & H_{{a,b}}
\\ H_{{b,a}} & H_{{b,b}} \end{{pmatrix}}$ and the order of basis is (a),
 (b), we can construct the creation operators $\psi_a^\dagger$  and $\
psi_b^\dagger$, and the annihilation operator $\psi_a$  and $\psi_b$.
The corresponding second quantized form is $\hat{{H}}=\vec{{\psi}}^\
dagger H \vec{{\psi}}$, where $\vec{{\psi}}=\begin{{pmatrix}} \psi_a \\
\psi_b \end{{pmatrix}}$ and $\vec{{\psi}}^\dagger=\begin{{pmatrix}} \
psi_a^\dagger & \psi_b^\dagger \end{{pmatrix}}$.
```

```
Second-quantization (summation)
**Prompt:**
You will be instructed to expand the second-quantized form Hamiltonian {
second_nonint_symbol} using {matrix_element_symbol} and {basis_symbol}.
```

```
You should follow the EXAMPLE below to expand the Hamiltonian.
You should use any previous knowledge to simplify it. For example, if
any term of {matrix_element_symbol} is zero, you should remove it from
the summation.
You should recall that {second_nonint_symbol} is {
expression_second_nonint}.
Return the expanded form of {second_nonint_symbol} after simplification.

Use the following conventions for the symbols (You should also obey the
conventions in all my previous prompts if you encounter undefined
symbols. If you find it is never defined or has conflicts in the
conventions, you should stop and let me know):
{definition_of_variables}

===
EXAMPLE:
For a $\hat{{H}}=\vec{{\psi}}^\dagger H \vec{{\psi}}$, where $\vec{{\psi
}}=\begin{{pmatrix}} \psi_a \\ \psi_b \end{{pmatrix}}$ and $\vec{{\psi
}}^\dagger=\begin{{pmatrix}} \psi_a^\dagger & \psi_b^\dagger \end{{
pmatrix}}$, we can expand it as  $\hat{{H}}=\sum_{{i,j=\{{a,b\}}}} \
psi_i^\dagger H_{{i,j}} \psi_j$.
```

```
Fourier transform noninteracting term to momentum space (continuum)
**Prompt:**
You will be instructed to convert the total noninteracting Hamiltonian
in the second quantized form from the basis in real space to the basis
by momentum space.
To do that, you should apply the Fourier transform to {real_creation_op}
 in the real space to the {momentum_creation_op} in the momentum space,
which is defined as {definition_of_Fourier_Transformation}, where {
real_variable} is integrated over the {entire_real|first_Brillouin_Zone
}. You should follow the EXAMPLE below to apply the Fourier transform.
Express the total noninteracting Hamiltonian {second_nonint_symbol} in
terms of {momentum_creation_op}. Simplify any summation index if
possible.

Use the following conventions for the symbols (You should also obey the
conventions in all my previous prompts if you encounter undefined
symbols. If you find it is never defined or has conflicts in the
conventions, you should stop and let me know):
{definition_of_variables}

===
EXAMPLE:
Write a Hamiltonian $\hat{{H}}$ in the second quantized form, $\hat{{H
}}=\int dr \psi(r)^\dagger H(r) \psi(r)$, where $r$ is integrated over
the entire real space.
Define the Fourier transform $c^\dagger(k)=\frac{{1}}{{\sqrt{{V}}}} \int
 \psi^\dagger(r) e^{{i k \cdot r}} dr$, where $r$ is integrated over the
 entire real space, and $V$ is the area of the unit cell in the real
space.
This leads to the inverse Fourier transform $\psi^\dagger(r) = \frac
{{1}}{{\sqrt{{V}}}} \sum_k c^\dagger(k) e^{{-i k \cdot r}}$, where $k$
```

```
is summed over the extended Brillouin zone (i.e., the entire momentum
space), $\Omega$ is the area of Brillouin zone in the momentum space.
Thus, substitute $\psi^\dagger(r)$ and $\psi(r)$ into $\hat{{H}}$, we
get
$$\hat{{H}} = \int dr \frac{{1}}{{\sqrt{{V}}}} \sum_{{k_1}} c^\dagger(
k_1) e^{{-i k_1 \cdot r}} H(r) \frac{{1}}{{\sqrt{{V}}}} \sum_{{k_2}} c(
k_2) e^{{i k_2 \cdot r}} =\sum_{{k_1,k_2}} c^\dagger(k_1) \frac{{1}}{{V
}} \int dr e^{{-i (k_1-k_2)\cdot r}} H(r) c(k_2) = \sum_{{k_1,k_2}} c^\
dagger(k_1) H(k_1,k_2) c(k_2)$$
, where we define the Fourier transform of $H(r)$ as $H(k_1,k_2)=\frac
{{1}}{{V}} \int dr e^{{-i (k_1-k_2)\cdot r}} H(r)$.
```

```
Fourier transform noninteracting term to momentum space (lattice)
**Prompt:**
You will be instructed to convert the noninteracting Hamiltonian {
nonint_symbol} in the second quantized form from the basis in real space
 to the basis in momentum space.
To do that, you should apply the Fourier transform to {real_creation_op}
 in the real space to the {momentum_creation_op} in the momentum space,
which is defined as {definition_of_Fourier_Transformation}, where {
real_variable} is integrated over all sites in the entire real space.
You should follow the EXAMPLE below to apply the Fourier transform. [
Note that hopping have no position dependence now.]
You should recall that {nonint_symbol} is {expression_nonint}
Express the total noninteracting Hamiltonian {nonint_symbol} in terms of
 {momentum_creation_op}. Simplify any summation index if possible.

Use the following conventions for the symbols (You should also obey the
conventions in all my previous prompts if you encounter undefined
symbols. If you find it is never defined or has conflicts in the
conventions, you should stop and let me know):
{definition_of_variables}

===
EXAMPLE:
Write a Kinetic Hamiltonian $\hat{{H}}$ in the second quantized form in
the real space, $\hat{{H}}=\sum_{{i,j}} t(R_i-R_j) c^\dagger(R_i) c(R_j)
$, where $i,j$ are summed over the entire real space.
Define the Fourier transform $c^\dagger(k)=\frac{{1}}{{\sqrt{{N}}}} \
sum_{{i}}c^\dagger(R_i) e^{{i k \cdot R_i}}$, where $i$ is integrated
over the entire real space containing $N$ unit cells, $N$ is the number
of unit cells.
This leads to the inverse Fourier transform $c^\dagger(R_i) = \frac
{{1}}{{\sqrt{{N}}}} \sum_k c^\dagger(k) e^{{-i k \cdot R_i}}$, where $k$
 is first Brillouin zone.
Thus, substitute $c^\dagger(R_i)$ and $c(R_j)$ into $\hat{{H}}$, we get
$$\hat{{H}} = \sum_{{i,j}} t(R_i-R_j) \frac{{1}}{{\sqrt{{N}}}} \sum_{{
k_1}} c^\dagger(k_1) e^{{-i k_1 \cdot R_i}} \frac{{1}}{{\sqrt{{N}}}} \
sum_{{k_2}} c(k_2) e^{{i k_2 \cdot R_j}} =\frac{{1}}{{N}} \sum_{{i,j}}\
sum_{{k_1,k_2}} c^\dagger(k_1)  c(k_2)  e^{{-i k_1\cdot R_i}} e^{{i k_2
\cdot R_j}} t(R_i-R_j) $$
Now make a replacement by defining $n= R_i-R_j$
The Hamiltonian become
```

```
$$\hat{{H}}=\frac{{1}}{{N}} \sum_{{i,n}} \sum_{{k_1,k_2}} c^\dagger(k_1)
  c(k_2) t(n) e^{{-i (k_1-k_2)\cdot R_i}} e^{{-i k_2 \cdot n}}$$
Because $\frac{{1}}{{N}}\sum_{{i}} e^{{-i (k_1-k_2)\cdot R_i}} = \delta(
k_1,k_2)$, where $\delta(k_1,k_2)$ is the Kronecker delta function.
therefore
$$\hat{{H}}=\sum_{{k_1,k_2}} \sum_{{n}} t(n) e^{{-i k_2 \cdot n}} c^\
dagger(k_1)  c(k_2) \delta(k_1,k_2)$$
Using the property of Kronecker delta function and sum over $k_2$, we
obtain
$$\hat{{H}}=\sum_{{k_1}} \sum_{{n}} t(n) e^{{-i k_1 \cdot n}} c^\dagger(
k_1)  c(k_1) $$
For simplicity, we replace $k_1$ with $k$, we obtain
$$\hat{{H}}=\sum_{{k}} \sum_{{n}} t(n) e^{{-i k \cdot n}} c^\dagger(k)
c(k)$$
If we define energy dispersion $E(k)=\sum_{{n}} t(n) e^{{-i k \cdot n}}$
, where $n$ is the summation of all hopping pairs, the Hamiltonian in
the momentum space is
$$\hat{{H}}=\sum_{{k}} E(k) c^\dagger(k)  c(k)$$
```

```
Fourier transform interacting term to momentum space (lattice)
**Prompt:**
You will be instructed to convert the interacting Hamiltonian, {
second_int_symbol}, in the {single-particle|second-quantized} form the
basis in real space to the basis in momentum space.
To do that, you should apply the Fourier transform to {real_creation_op}
 in the real space to the {momentum_creation_op} in the momentum space,
which is defined as {definition_of_Fourier_Transformation}, where {
real_variable} is integrated over all sites in the entire real space,
and {momentum_var} is defined within the first Brillouin zone. You
should follow the EXAMPLE below to apply the Fourier transform. [Note
that interaction have no position dependence now]
You should recall that {second_int_symbol} is {expression_int}.
Express {second_int_symbol} in terms of {momentum_creation_op}. Simplify
 any summation index if possible.

===
EXAMPLE:
Write an interacting Hamiltonian $\hat{{H}}^{{int}}$ in the second
quantized form in the real space, $\hat{{H}}^{{int}}=\sum_{{s,s'}}\sum_
{{i,j}} U(R_i-R_j) c_s^\dagger(R_i) c_{{s'}}^\dagger(R_j) c_{{s'}}(R_j)
c_s(R_i)$, where $i,j$ are summed over the entire real space.
Define the Fourier transform $c_s^\dagger(k)=\frac{{1}}{{\sqrt{{N}}}} \
sum_{{i}}c_s^\dagger(R_i) e^{{i k \cdot R_i}}$, where $i$ is integrated
over the entire real space containing $N$ unit cells, $N$ is the number
of unit cells.
This leads to the inverse Fourier transform $c_s^\dagger(R_i) = \frac
{{1}}{{\sqrt{{N}}}} \sum_k c_s^\dagger(k) e^{{-i k \cdot R_i}}$, where
$k$ is summed over the first Brillouin zone.
Thus, substitute $c^\dagger(R_i)$ and $c(R_j)$ into $\hat{{H}}^{{int}}$,
 we get
$$\hat{{H}}^{{int}} = \sum_{{s,s'}}\sum_{{i,j}} U(R_i-R_j) \frac{{1}}{{\
sqrt{{N}}}} \sum_{{k_1}} c_s^\dagger(k_1) e^{{-i k_1 \cdot R_i}} \frac
{{1}}{{\sqrt{{N}}}} \sum_{{k_2}} c_{{s'}}^\dagger(k_2) e^{{-i k_2 \cdot
```

```
R_j}} \frac{{1}}{{\sqrt{{N}}}} \sum_{{k_3}} c_{{s'}}(k_3) e^{{i k_3 \
cdot R_j}} \frac{{1}}{{\sqrt{{N}}}} \sum_{{k_4}} c_s(k_4) e^{{i k_4 \
cdot R_i}}=\sum_{{s,s'}}\sum_{{i,j}}\frac{{1}}{{N^2}}\sum_{{k_1,k_2,k_3,
k_4}}U(R_i-R_j)c_s^\dagger(k_1)c_{{s'}}^\dagger(k_2)c_{{s'}}(k_3)c_s(k_4
)e^{{-i(k_1-k_4)\cdot R_i}} e^{{-i(k_2-k_3)\cdot R_j}}$$
Now make a replacement by defining $n= R_i-R_j$
The Hamiltonian become
$$\hat{{H}}^{{int}}=\frac{{1}}{{N^2}} \sum_{{j,n}} \sum_{{s,s'}} \sum_{{
k_1,k_2,k_3,k_4}} U(n) c_s^\dagger(k_1)c_{{s'}}^\dagger(k_2)c_{{s'}}(k_3
)c_s(k_4)e^{{-i(k_1-k_4)\cdot n}} e^{{-i(k_1-k_4+k_2-k_3)\cdot r_j }}$$
Because $\frac{{1}}{{N}}\sum_{{i}} e^{{-i (k_1-k_4+k_2-k_3)\cdot R_i}} =
 \sum\delta(k_1-k_4+k_2-k_3,G)$, where $\delta(..,..)$ is the Kronecker
delta function, and $G$ is the all reciprocal lattices in the momentum
space.
Therefore,
$$\hat{{H}}^{{int}}=\frac{{1}}{{N}}\sum_{{s,s'}}\sum_{{k_1,k_2,k_3,k_4}}
 \sum_{{n}} U(n) e^{{-i (k_1-k_4) \cdot n}} c_s^\dagger(k_1)c_{{s'}}^\
dagger(k_2)c_{{s'}}(k_3)c_s(k_4) \sum_{{G}} \delta(k_1-k_4+k_2-k_3,G)$$
If we define interaction in the momentum space $U(k)=\sum_{{n}} U(n) e
^{{-i k \cdot n}}$, where $n$ is the summation of all hopping pairs, the
 interacting Hamiltonian in the momentum space is
$$\hat{{H}}^{{int}}=\frac{{1}}{{N}}\sum_{{s,s'}}\sum_{{k_1,k_2,k_3,k_4}}
  U(k_1-k_4) c_s^\dagger(k_1)c_{{s'}}^\dagger(k_2)c_{{s'}}(k_3)c_s(k_4)
\sum_{{G}} \delta(k_1-k_4+k_2-k_3,G)$$
```

```
Particle-hole transformation
**Prompt:**
You will be instructed to perform a particle-hole transformation.
Define a hole operator, {hole_op}, which equals {particle_op}.
You should replace {particle_creation_op} with {hole_creation_op}, and {
particle_annihilation_op} with {hole_annihilation_op}. You should follow
 the EXAMPLE below to apply the particle-hole transformation.
You should recall that {expression_particle_Ham}.
Return the {second_nonint_symbol} in the hole operators.

Use the following conventions for the symbols (You should also obey the
conventions in all my previous prompts if you encounter undefined
symbols. If you find it is never defined or has conflicts in the
conventions, you should stop and let me know):
{definition_of_variables}

===
EXAMPLE:
Give a Hamiltonian  $\hat{{H}}=\sum_{{k_1,k_2}} c^\dagger(k_1) h(k_1,k_2
) c(k_2)$ , and the particle-hole transformation as $b(k)=c^\dagger(k)$.
 The transformed Hamiltonian is $\hat{{H}}=\sum_{{k_1,k_2}} b(k_1) h(k_1
,k_2) b^\dagger(k_2)$
```

```
Simplify the Hamiltonian in the particle-hole basis
**Prompt:**
```

```
You will be instructed to simplify the {second_nonint_symbol} in the
hole basis.
You should use canonical commutator relation for fermions to reorder the
 hole operator to the normal order. Normal order means that creation
operators always appear before the annihilation operators.  You should
follow the EXAMPLE below to simplify it to the normal order.
Express the {second_nonint_symbol} in the normal order of {hole_op} and
also make {index_1} always appear before {index_2} in the index of {op}
and {Ham_op}.
You should recall that {expression_hole_Ham}
Use the following conventions for the symbols (You should also obey the
conventions in all my previous prompts if you encounter undefined
symbols. If you find it is never defined or has conflicts in the
conventions, you should stop and let me know):
{definition_of_variables}

===
EXAMPLE:
For $\hat{{H}}^{{0}}= \sum_{{i,j}} b_i H_{{i,j}} b_j^\dagger$, where
$b_i$ satisfies fermion statistics (anticommuting to its self-adjoint
operator).
This gives $`[b_i, b_j^\dagger]_{{+}} = \delta_{{i,j}}`$, which means
$b_i b_j^\dagger=\delta_{{i,j}}-b_j^\dagger b_i$.
Substitute it into $\hat{{H}}^{{0}}$, we have $\hat{{H}}^{{0}}=\sum_{{i,
j}} (\delta_{{i,j}}-b_j^\dagger b_i) H_{{i,j}}=\sum_{{i,j}} \delta_{{i,j
}} H_{{i,j}} - \sum_{{i,j}}b_j^\dagger b_i H_{{i,j}}=\sum_i H_{{i,i}} -
\sum_{{i,j}}b_j^\dagger b_i H_{{i,j}}$.
The first term is simply $\sum_i H_{{i,i}}$ by summing over the index
$j$ due to $\delta_{{i,j}}$.
The second term is $-\sum_{{i,j}}b_j^\dagger b_i H_{{i,j}}$.
Relabeling the index of $i$ and $j$ by swapping them to make it
consistent with the original order of index (namely, $i$ appears before
$j$ in the index of $b$ and $H$), it becomes $-\sum_{{i,j}}b_i^\dagger
H_{{j,i}} b_j$.
Finally, to fix the order of the index in $H$ such that $i$ appears
before $j$, we notice that $`H_{{j,i}}=(H_{{i,j}})^*`$, where $`^*`$
means complex conjugate, because the Hamiltonian is Hermitian.
Thus, we end up in $\hat{{H}}^{{0}}=\sum_{{i,j}} b_i H_{{i,j}} b_j^\
dagger=\sum_i H_{{i,i}}-\sum_{{i,j}}b_i^\dagger (H_{{i,j}})^* b_j$
```

```
Wick's theorem expansion
**Prompt:**
You will be instructed to perform a Hartree-Fock approximation to expand
 the interaction term, {second_int_symbol}.
You should use Wick's theorem to expand the four-fermion term in {
second_int_symbol} into quadratic terms. You should strictly follow the
EXAMPLE below to expand using Wick's theorem, select the correct EXAMPLE
 by noticing the order of four-term product with and without ${}^\
dagger$, and be extremely cautious about the order of the index and sign
 before each term.
You should only preserve the normal terms. Here, the normal terms mean
the product of a creation operator and an annihilation operator.
You should recall that {second_int_symbol} is {expression_int}.
```

```
Return the expanded interaction term after Hartree-Fock approximation as
 {Hartree_Fock_symbol}.

Use the following conventions for the symbols (You should also obey the
conventions in all my previous prompts if you encounter undefined
symbols. If you find it is never defined or has conflicts in the
conventions, you should stop and let me know):
{definition_of_variables}

===
EXAMPLE 1:
For a four-fermion term $a_1^\dagger a_2^\dagger a_3 a_4$, using Wick's
theorem and preserving only the normal terms. this is expanded as $a_1^\
dagger a_2^\dagger a_3 a_4 = \langle a_1^\dagger a_4 \rangle a_2^\dagger
 a_3 + \langle a_2^\dagger a_3 \rangle a_1^\dagger a_4 - \langle a_1^\
dagger a_4 \rangle \langle a_2^\dagger a_3\rangle - \langle a_1^\dagger
a_3 \rangle a_2^\dagger a_4 - \langle a_2^\dagger a_4 \rangle a_1^\
dagger a_3 + \langle a_1^\dagger a_3\rangle \langle a_2^\dagger a_4 \
rangle$
Be cautious about the order of the index and sign before each term here.

EXAMPLE 2:
For a four-fermion term $a_1^\dagger a_2 a_3^\dagger a_4$, using Wick's
theorem and preserving only the normal terms. this is expanded as $a_1^\
dagger a_2 a_3^\dagger a_4 = \langle a_1^\dagger a_2 \rangle a_3^\dagger
 a_4 + \langle a_3^\dagger a_4 \rangle a_1^\dagger a_2 - \langle a_1^\
dagger a_2 \rangle \langle a_3^\dagger a_4\rangle - \langle a_1^\dagger
a_4 \rangle a_3^\dagger a_2 - \langle a_3^\dagger a_2 \rangle a_1^\
dagger a_4 + \langle a_1^\dagger a_4\rangle \langle a_3^\dagger a_2 \
rangle$
Be cautious about the order of the index and sign before each term here.
```

```
Drop constant terms
**Prompt:**
You will be instructed to extract the quadratic terms in the {
Hartree_Fock_term_symbol}.
The quadratic terms mean terms that are proportional to {bilinear_op},
which excludes terms that are solely expectations or products of
expectations.
You should only preserve the quadratic terms in {
Hartree_Fock_term_symbol}, denoted as {
Hartree_Fock_second_quantized_symbol}.
You should recall that {Hartree_Fock_term_symbol} is {expression_HF}.
Return {Hartree_Fock_second_quantized_symbol}.

Use the following conventions for the symbols (You should also obey the
conventions in all my previous prompts if you encounter undefined
symbols. If you find it is never defined or has conflicts in the
conventions, you should stop and let me know):
{definition_of_variables}
```

```
Keep Hartree term
**Prompt:**
You will be instructed to keep only the Hartree term in {
Hartree_Fock_second_quantized_symbol}.
Here, Hartree term only means that only the expected value in the form {
expected_value_Hartree} (Note that the two indices are the same) should
be the preserved. All other expected value terms should be dropped.
You should recall that {Hartree_Fock_second_quantized_symbol} is {
expression_HF}
Return the simplified Hamiltonian with {Hartree_second_quantized_symbol
}.
```

```
Keep Fock term
**Prompt:**
You will be instructed to keep only the Fock term in {
Hartree_Fock_second_term_symbol}.
Here, Fock term only means that only the expected value in the form {
expected_value_Fock} (Note that the two indices are the different)
should be the preserved. All other expected value terms should be
dropped.
You should recall that {Hartree_Fock_second_term_symbol} is {
expression_HF}
Return the simplified Hamiltonian with {Fock_second_quantized_symbol}.
```

```
Identify momentum transfer in interaction
**Prompt:**
You will be instructed to expand interaction term $V(q)$ in the MF
quadratic term {Hartree_Fock_second_quantized_symbol}.
If you find the $V(q)$ in {Hartree_Fock_second_quantized_symbol} does
not contain any momentum that is not in the summation sign. The
interaction term is already expanded. No action to perform on
interaction term.
Otherwise, you will expand $V(q)$ by replacing $q$ with the momentum {
momentum}.
You should recall that {Hartree_Fock_second_quantized_symbol} is {
expression_HF_2}.
Return {Hartree_Fock_second_quantized_symbol} with expanded interaction.
```

```
Relabel the index
**Prompt:**
You will be instructed to simplify the quadratic term {
Hartree_Fock_second_quantized_symbol} through relabeling the index.
The logic is that the expected value ({expected_value}) in the first
Hartree term ({expression_Hartree_1}) has the same form as the quadratic
 operators in the second Hartree term ({expression_Hartree_2}), and vice
 versa. The same applies to the Fock term.
```

```
Namely, a replacement of {relabel} is applied to ONLY the second Hartree
 or Fock term. You should not swap any index that is not in the
summation, which includes {Unsummed_Indices}.
This means, if you relabel the index by swapping the index in the "
expected value" and "quadratic operators" in the second Hartree or Fock
term, you can make the second Hartree or Fock term look identical to the
 first Hartree or Fock term, as long as $V(q)=V(-q)$, which is naturally
 satisfied in Coulomb interaction. You should follow the EXAMPLE below
to simplify it through relabeling the index.
You should recall that {Hartree_Fock_second_quantized_symbol} is {
expression_HF_2}
Return the simplified {Hartree_Fock_second_quantized_symbol}.

===
EXAMPLE:
Given a Hamiltonian $\hat{{H}}=\sum_{{k_1,k_2, k_3, k_4,\sigma_1,\
sigma_2,\sigma_3,\sigma_4}} V(k_1-k_4) (\langle c_{{d,\sigma_1}}^\dagger
(k_1) c_{{d,\sigma_4}}(k_4) \rangle c_{{p,\sigma_2}}^\dagger(k_2) c_{{p
,\sigma_3}}(k_3) + \langle c_{{p,\sigma_2}}^\dagger(k_2) c_{{d,\sigma_3
}}(k_3) \rangle c_{{d,\sigma_1}}^\dagger(k_1) c_{{\sigma_4}}(k_4) ) \
delta_{{k_1+k_2,k_3+k_4}}$, where $V(q)=V(-q)$.
In the second term, we relabel the index to swap the index in expected
value and the index in quadratic operators, namely, $\sigma_1 \
leftrightarrow \sigma_2$, $\sigma_3 \leftrightarrow \sigma_4$, $k_1 \
leftrightarrow k_2$, $k_3 \leftrightarrow k_4$. Important: $d$ and $p$
cannot be swapped because they are not indices in the summation.
After the replacement, the second term becomes $\sum_{{k_1,k_2, k_3, k_4
,\sigma_1,\sigma_2,\sigma_3,\sigma_4}} V(k_2-k_3) \langle c_{{p,\sigma_1
}}^\dagger(k_1) c_{{p,\sigma_4}}(k_4) \rangle c_{{d,\sigma_2}}^\dagger(
k_2) c_{{d,\sigma_3}}(k_3) \delta_{{k_4+k_3,k_2+k_1}}$.
Note that the Kronecker dirac function $\delta_{{k_4+k_3,k_2+k_1}}$
implies $k_1+k_2=k_3+k_4$, i.e., $k_2-k_3=k_4-k_1$. Thus, the second
term simplifies to $\sum_{{k_1,k_2, k_3, k_4,\sigma_1,\sigma_2,\sigma_3
,\sigma_4}} V(k_4-k_1) \langle c_{{p,\sigma_1}}^\dagger(k_1) c_{{p,\
sigma_4}}(k_4) \rangle c_{{d,\sigma_2}}^\dagger(k_2) c_{{d,\sigma_3}}(
k_3) \delta_{{k_4+k_3,k_2+k_1}}$.
Because $V(q)=V(-q)$, meaning $V(k_4-k_1)=V(k_1-k_4)$, the second term
further simplifies to $\sum_{{k_1,k_2, k_3, k_4,\sigma_1,\sigma_2,\
sigma_3,\sigma_4}} V(k_1-k_4) \langle c_{{p,\sigma_1}}^\dagger(k_1) c_{{
p,\sigma_4}}(k_4) \rangle c_{{d,\sigma_2}}^\dagger(k_2) c_{{d,\sigma_3
}}(k_3) \delta_{{k_4+k_3,k_2+k_1}}$.
Finally, we have the simplified Hamiltonian as  $\hat{{H}}=\sum_{{k_1,
k_2, k_3, k_4,\sigma_1,\sigma_2,\sigma_3,\sigma_4}} V(k_1-k_4) (\langle
c_{{d,\sigma_1}}^\dagger(k_1) c_{{d,\sigma_4}}(k_4) \rangle c_{{p,\
sigma_2}}^\dagger(k_2) c_{{p,\sigma_3}}(k_3) + \langle c_{{p,\sigma_1
}}^\dagger(k_1) c_{{p,\sigma_4}}(k_4) \rangle c_{{d,\sigma_2}}^\dagger(
k_2) c_{{d,\sigma_3}}(k_3)) \delta_{{k_4+k_3,k_2+k_1}}$.
```

```
Combine Hartree/Fock terms
**Prompt:**
You will be instructed to simplify the quadratic term {
Hartree_Fock_second_quantized_symbol} through relabeling the index to
combine the two Hartree/Fock term into one Hartree/Fock term.
```

```
The logic is that the expected value ({expected_value}) in the first
Hartree term ({expression_Hartree_1}) has the same form as the quadratic
 operators in the second Hartree term ({expression_Hartree_2}), and vice
 versa. The same applies to the Fock term.
This means, if you relabel the index by swapping the index in the "
expected value" and "quadratic operators" in the second Hartree term,
you can make the second Hartree term look identical to the first Hartree
 term, as long as $V(q)=V(-q)$, which is naturally satisfied in Coulomb
interaction. You should follow the EXAMPLE below to simplify it through
relabeling the index.
You should perform this trick of "relabeling the index" for both two
Hartree terms and two Fock terms to reduce them to one Hartree term, and
 one Fock term.
You should recall that {Hartree_Fock_second_quantized_symbol} is {
expression_HF_2}.
Return the simplified {Hartree_Fock_second_quantized_symbol} which
reduces from four terms (two Hartree and two Fock terms) to only two
terms (one Hartree and one Fock term)

===
EXAMPLE:
Given a Hamiltonian $\hat{{H}}=\sum_{{k_1,k_2, k_3, k_4,\sigma_1,\
sigma_2,\sigma_3,\sigma_4}} V(k_1-k_4) (\langle c_{{\sigma_1}}^\dagger(
k_1) c_{{\sigma_4}}(k_4) \rangle c_{{\sigma_2}}^\dagger(k_2) c_{{\
sigma_3}}(k_3) + \langle c_{{\sigma_2}}^\dagger(k_2) c_{{\sigma_3}}(k_3)
 \rangle c_{{\sigma_1}}^\dagger(k_1) c_{{\sigma_4}}(k_4) ) \delta_{{k_1+
k_2,k_3+k_4}}$, where $V(q)=V(-q)$.
In the second term, we relabel the index to swap the index in expected
value and the index in quadratic operators, namely, $\sigma_1 \
leftrightarrow \sigma_2$, $\sigma_3 \leftrightarrow \sigma_4$, $k_1 \
leftrightarrow k_2$, $k_3 \leftrightarrow k_4$. After the replacement,
the second term becomes $\sum_{{k_1,k_2, k_3, k_4,\sigma_1,\sigma_2,\
sigma_3,\sigma_4}} V(k_2-k_3) \langle c_{{\sigma_1}}^\dagger(k_1) c_{{\
sigma_4}}(k_4) \rangle c_{{\sigma_2}}^\dagger(k_2) c_{{\sigma_3}}(k_3) \
delta_{{k_4+k_3,k_2+k_1}}$.
Note that the Kronecker dirac function $\delta_{{k_4+k_3,k_2+k_1}}$
implies $k_1+k_2=k_3+k_4$, i.e., $k_2-k_3=k_4-k_1$. Thus, the second
term simplifies to $\sum_{{k_1,k_2, k_3, k_4,\sigma_1,\sigma_2,\sigma_3
,\sigma_4}} V(k_4-k_1) \langle c_{{\sigma_1}}^\dagger(k_1) c_{{\sigma_4
}}(k_4) \rangle c_{{\sigma_2}}^\dagger(k_2) c_{{\sigma_3}}(k_3) \delta_
{{k_4+k_3,k_2+k_1}}$.
Because $V(q)=V(-q)$, meaning $V(k_4-k_1)=V(k_1-k_4)$, the second term
further simplifies to $\sum_{{k_1,k_2, k_3, k_4,\sigma_1,\sigma_2,\
sigma_3,\sigma_4}} V(k_1-k_4) \langle c_{{\sigma_1}}^\dagger(k_1) c_{{\
sigma_4}}(k_4) \rangle c_{{\sigma_2}}^\dagger(k_2) c_{{\sigma_3}}(k_3) \
delta_{{k_4+k_3,k_2+k_1}}$. Note that this form of second term after
relabeling is identical to the first term.
Finally, we have the simplified Hamiltonian as  $\hat{{H}}=2\sum_{{k_1,
k_2, k_3, k_4,\sigma_1,\sigma_2,\sigma_3,\sigma_4}} V(k_1-k_4) \langle
c_{{\sigma_1}}^\dagger(k_1) c_{{\sigma_4}}(k_4) \rangle c_{{\sigma_2}}^\
dagger(k_2) c_{{\sigma_3}}(k_3) \delta_{{k_4+k_3,k_2+k_1}}$.
```

```
Identify order parameters in Hartree term (extended BZ)
**Prompt:**
You will be instructed to simplify the Hartree term in {
Hartree_second_quantized_symbol} by reducing the momentum inside the
expected value {expected_value}.
The expected value {expected_value} is only nonzero when the two momenta
 $k_i,k_j$ are the same, namely, {expected_value_nonzero}.
You should use the property of Kronecker delta function $\delta_{{k_i,
k_j}}$ to reduce one momentum $k_i$ but not $b_i$.
Once you reduce one momentum inside the expected value $\langle\dots\
rangle$. You will also notice the total momentum conservation will
reduce another momentum in the quadratic term. Therefore, you should end
 up with only two momenta left in the summation.
You should follow the EXAMPLE below to reduce one momentum in the
Hartree term, and another momentum in the quadratic term.
You should recall that {Hartree_second_quantized_symbol} is {
expression_Hartree}.
Return the final simplified Hartree term {
Hartree_second_quantized_symbol}.

===
EXAMPLE:
Given a Hamiltonian where the Hartree term $\hat{{H}}^{{Hartree}}=\sum_
{{k_1,k_2, k_3, k_4,b_1,b_2,b_3,b_4}} V(k_1-k_4+b_1-b_4) \langle c_{{b_1
}}^\dagger(k_1) c_{{b_4}}(k_4) \rangle c_{{b_2}}^\dagger(k_2) c_{{b_3}}(
k_3) \delta_{{k_1+k_2+b_1+b_2,k_3+k_4+b_3+b_4}}$, where $k_i$ is the
momentum inside first Brilloun zone and $b_i$ is the reciprocal lattice.
Inside the expected value, we realize $\langle c_{{b_1}}^\dagger(k_1) c_
{{b_4}}(k_4) \rangle$ is nonzero only when $k_1=k_4$, i.e., $\langle c_
{{b_1}}^\dagger(k_1) c_{{b_4}}(k_4) \rangle=\langle c_{{b_1}}^\dagger(
k_1) c_{{b_4}}(k_4) \rangle\delta_{{k_1,k_4}}$.
Thus, the Hartree term becomes $\sum_{{k_1,k_2, k_3, k_4,b_1,b_2,b_3,b_4
}} V(k_1-k_4+b_1-b_4) \langle c_{{b_1}}^\dagger(k_1) c_{{b_4}}(k_4) \
rangle \delta_{{k_1,k_4}} c_{{b_2}}^\dagger(k_2) c_{{b_3}}(k_3) \delta_
{{k_1+k_2+b_1+b_2,k_3+k_4+b_3+b_4}}$.
Use the property of Kronecker delta function $\delta_{{k_1,k_4}}$ to sum
 over $k_4$, we have $\sum_{{k_1, k_2, k_3,b_1,b_2,b_3,b_4}} V(k_1-k_1+
b_1-b_4) \langle c_{{b_1}}^\dagger(k_1) c_{{b_4}}(k_1) \rangle c_{{b_2
}}^\dagger(k_2) c_{{b_3}}(k_3) \delta_{{k_1+k_2+b_1+b_2,k_3+k_1+b_3+b_4
}}=\sum_{{k_1, k_2, k_3,b_1,b_2,b_3,b_4}} V(b_1-b_4) \langle c_{{b_1}}^\
dagger(k_1) c_{{b_4}}(k_1) \rangle c_{{b_2}}^\dagger(k_2) c_{{b_3}}(k_3)
 \delta_{{k_2+b_1+b_2,k_3+b_3+b_4}}$.
Because $k_i$ is momentum inside first Brilloun zone while $b_i$ is the
reciprocal lattice. It is only when $k_2=k_3$ that $\delta_{{k_2+b_1+b_2
,k_3+b_3+b_4}}$ is nonzero, i.e., $\delta_{{k_2+b_1+b_2,k_3+b_3+b_4}}=\
delta_{{b_1+b_2,b_3+b_4}}\delta_{{k_2,k_3}}$. Therefore, the Hartree
term simplifies to $\sum_{{k_1, k_2, k_3,b_1,b_2,b_3,b_4}} V(b_1-b_4) \
langle c_{{b_1}}^\dagger(k_1) c_{{b_4}}(k_1) \rangle c_{{b_2}}^\dagger(
k_2) c_{{b_3}}(k_3) \delta_{{b_1+b_2,b_3+b_4}}\delta_{{k_2,k_3}}=\sum_{{
k_1, k_2,b_1,b_2,b_3,b_4}} V(b_1-b_4) \langle c_{{b_1}}^\dagger(k_1) c_
{{b_4}}(k_1) \rangle c_{{b_2}}^\dagger(k_2) c_{{b_3}}(k_2) \delta_{{b_1+
b_2,b_3+b_4}}$.
Therefore, the final simplified Hartree term after reducing two momenta
is $\hat{{H}}^{{Hartree}}=\sum_{{k_1, k_2,b_1,b_2,b_3,b_4}}  V(b_1-b_4)
\langle c_{{b_1}}^\dagger(k_1) c_{{b_4}}(k_1) \rangle c_{{b_2}}^\dagger(
k_2) c_{{b_3}}(k_2) \delta_{{b_1+b_2,b_3+b_4}}$
```

```
Identify order parameters in Hartree term
**Prompt:**
You will be instructed to simplify the Hartree term, {
Hartree_second_quantized_symbol}, by reducing the momentum inside the
expected value {expected_value}.
The expected value {expected_value} is only nonzero when the two momenta
 $k_i,k_j$ are the same, namely, {expected_value_nonzero}.
You should use the property of Kronecker delta function $\delta_{{k_i,
k_j}}$ to reduce one momentum $k_i$.
Once you reduce one momentum inside the expected value $\langle\dots\
rangle$. You will also notice the total momentum conservation will
reduce another momentum in the quadratic term. Therefore, you should end
 up with only two momenta left in the summation.
You should follow the EXAMPLE below to reduce one momentum in the
Hartree term, and another momentum in the quadratic term.
You should recall that {Hartree_second_quantized_symbol} is {
expression_Hartree}.
Return the final simplified Hartree term {
Hartree_second_quantized_symbol}.

===
EXAMPLE:
Given a Hamiltonian where the Hartree term $\hat{{H}}^{{Hartree}}=\sum_
{{k_1,k_2, k_3, k_4,s_1,s_2}} V(k_1-k_4) \langle c_{{s_1}}^\dagger(k_1)
c_{{s_1}}(k_4) \rangle c_{{s_2}}^\dagger(k_2) c_{{s_2}}(k_3) \sum_{{G}}\
delta_{{k_1+k_2-k_3-k_4,G}}$, where $k_i$ is the momentum inside first
Brilloun zone, $G$ is the reciprocal lattice vectors, and $s_i$ is a
certain index for the degree of freedom other than momentum.
Inside the expected value, we realize $\langle c_{{s_1}}^\dagger(k_1) c_
{{s_1}}(k_4) \rangle$ is nonzero only when $k_1=k_4$, i.e., $\langle c_
{{s_1}}^\dagger(k_1) c_{{s_1}}(k_4) \rangle=\langle c_{{s_1}}^\dagger(
k_1) c_{{s_1}}(k_4) \rangle\delta_{{k_1,k_4}}$.
Thus, the Hartree term becomes $\sum_{{k_1,k_2, k_3, k_4,s_1,s_2}} V(k_1
-k_4) \langle c_{{s_1}}^\dagger(k_1) c_{{s_1}}(k_4) \rangle \delta_{{k_1
,k_4}} c_{{s_2}}^\dagger(k_2) c_{{s_2}}(k_3) \sum_{{G}}\delta_{{k_1+k_2-
k_3-k_4,G}}$.
Use the property of Kronecker delta function $\delta_{{k_1,k_4}}$ to sum
 over $k_4$, we have $\sum_{{k_1, k_2, k_3,s_1,s_2}} V(k_1-k_1) \langle
c_{{s_1}}^\dagger(k_1) c_{{s_1}}(k_1) \rangle c_{{s_2}}^\dagger(k_2) c_
{{s_2}}(k_3) \sum_{{G}}\delta_{{k_1+k_2-k_3-k_1,G}}=\sum_{{k_1, k_2, k_3
,s_1,s_2}} V(0) \langle c_{{s_1}}^\dagger(k_1) c_{{s_1}}(k_1) \rangle c_
{{s_2}}^\dagger(k_2) c_{{s_2}}(k_3) \sum_{{G}}\delta_{{k_2-k_3,G}}$.
We can further simplify $\sum_{{G}}\delta_{{k_2-k_3,G}}$. Because $k_i$
is momentum inside first Brilloun zone, and the difference between $k_2$
 and $k_3$ cannot exceed the first shell of reciprocal lattice vector,
which means $G$ can only take the value of the origin point in the
reciprocal lattice, therefore, $\sum_{{G}}\delta_{{k_2-k_3,G}}=\delta_{{
k_2-k_3,0}}$.
Thus, the Hartree term simplifies to $\sum_{{k_1, k_2, k_3,s_1,s_2}} V
(0) \langle c_{{s_1}}^\dagger(k_1) c_{{s_1}}(k_1) \rangle c_{{s_2}}^\
dagger(k_2) c_{{s_2}}(k_3) \delta_{{k_2-k_3,0}}=\sum_{{k_1, k_2,s_1,s_2
}} V(0) \langle c_{{s_1}}^\dagger(k_1) c_{{s_1}}(k_1) \rangle c_{{s_2
}}^\dagger(k_2) c_{{s_2}}(k_2)$.
Therefore, the final simplified Hartree term after reducing one momentum
 is $\hat{{H}}^{{Hartree}}=\sum_{{k_1, k_2,s_1,s_2}} V(0) \langle c_{{
s_1}}^\dagger(k_1) c_{{s_1}}(k_1) \rangle c_{{s_2}}^\dagger(k_2) c_{{s_2
```

```
}}(k_2)$
```

```
Identify order parameters in Fock term (extended BZ)
**Prompt:**
You will be instructed to simplify the Fock term in {
Fock_second_quantized_symbol} by reducing the momentum inside the
expected value {expected_value}.
The expected value {expected_value} is only nonzero when the two momenta
 $k_i,k_j$ are the same, namely, {expected_value_nonzero}.
You should use the property of Kronecker delta function $\delta_{{k_i,
k_j}}$ to reduce one momentum $k_i$ but not $b_i$.
Once you reduce one momentum inside the expected value $\langle\dots\
rangle$. You will also notice the total momentum conservation will
reduce another momentum in the quadratic term. Therefore, you should end
 up with only two momenta left in the summation.
You should follow the EXAMPLE below to reduce one momentum in the Fock
term, and another momentum in the quadratic term.
You should recall that {Fock_second_quantized_symbol} is {
expression_Fock}.
Return the final simplified Fock term {Fock_second_quantized_symbol}.

===
EXAMPLE:
Given a Hamiltonian where the Fock term $\hat{{H}}^{{Fock}}=-\sum_{{k_1,
k_2, k_3, k_4,b_1,b_2,b_3,b_4}} V(k_1-k_4+b_1-b_4) \langle c_{{b_1}}^\
dagger(k_1) c_{{b_3}}(k_3) \rangle c_{{b_2}}^\dagger(k_2) c_{{b_4}}(k_4)
  \delta_{{k_1+k_2+b_1+b_2,k_3+k_4+b_3+b_4}}$, where $k_i$ is the
momentum inside first Brilloun zone and $b_i$ is the reciprocal lattice.
Inside the expected value, we realize $\langle c_{{b_1}}^\dagger(k_1) c_
{{b_3}}(k_3) \rangle$ is nonzero only when $k_1=k_3$, i.e., $\langle c_
{{b_1}}^\dagger(k_1) c_{{b_3}}(k_3) \rangle=\langle c_{{b_1}}^\dagger(
k_1) c_{{b_3}}(k_3) \rangle\delta_{{k_1,k_3}}$.
Thus, the Fock term becomes $-\sum_{{k_1,k_2, k_3, k_4,b_1,b_2,b_3,b_4}}
 V(k_1-k_4+b_1-b_4) \langle c_{{b_1}}^\dagger(k_1) c_{{b_3}}(k_3) \
rangle \delta_{{k_1,k_3}} c_{{b_2}}^\dagger(k_2) c_{{b_4}}(k_4) \delta_
{{k_1+k_2+b_1+b_2,k_3+k_4+b_3+b_4}}$.
Use the property of Kronecker delta function $\delta_{{k_1,k_3}}$ to sum
 over $k_3$, we have $-\sum_{{k_1,k_2, k_4,b_1,b_2,b_3,b_4}} V(k_1-k_4+
b_1-b_4) \langle c_{{b_1}}^\dagger(k_1) c_{{b_3}}(k_1) \rangle c_{{b_2
}}^\dagger(k_2) c_{{b_4}}(k_4) \delta_{{k_1+k_2+b_1+b_2,k_1+k_4+b_3+b_4
}}=-\sum_{{k_1,k_2, k_4,b_1,b_2,b_3,b_4}} V(k_1-k_4+b_1-b_4) \langle c_
{{b_1}}^\dagger(k_1) c_{{b_3}}(k_1) \rangle c_{{b_2}}^\dagger(k_2) c_{{
b_4}}(k_4) \delta_{{k_2+b_1+b_2,k_4+b_3+b_4}}$.
Because $k_i$ is momentum inside first Brilloun zone while $b_i$ is the
reciprocal lattice. It is only when $k_2=k_4$ that $\delta_{{k_2+b_1+b_2
,k_4+b_3+b_4}}$ is nonzero, i.e., $\delta_{{k_2+b_1+b_2,k_4+b_3+b_4}}=\
delta_{{b_1+b_2,b_3+b_4}}\delta_{{k_2,k_4}}$.
Therefore, the Fock term simplifies to $-\sum_{{k_1,k_2, k_4,b_1,b_2,b_3
,b_4}}  V(k_1-k_4+b_1-b_4) \langle c_{{b_1}}^\dagger(k_1) c_{{b_3}}(k_1)
 \rangle c_{{b_2}}^\dagger(k_2) c_{{b_4}}(k_4) \delta_{{b_1+b_2,b_3+b_4
}}\delta_{{k_2,k_4}}=-\sum_{{k_1,k_2, b_1,b_2,b_3,b_4}} V(k_1-k_2+b_1-
b_4) \langle c_{{b_1}}^\dagger(k_1) c_{{b_3}}(k_1) \rangle c_{{b_2}}^\
dagger(k_2) c_{{b_4}}(k_2) \delta_{{b_1+b_2,b_3+b_4}}$.
```

```
Therefore, the final simplified Fock term after reducing two momenta is
$\hat{{H}}^{{Fock}}=-\sum_{{k_1, k_2,b_1,b_2,b_3,b_4}}  V(k_1-k_2+b_1-
b_4) \langle c_{{b_1}}^\dagger(k_1) c_{{b_3}}(k_1) \rangle c_{{b_2}}^\
dagger(k_2) c_{{b_4}}(k_2) \delta_{{b_1+b_2,b_3+b_4}}$
```

```
Identify order parameters in Fock term
**Prompt:**
You will be instructed to simplify the Fock term in {
Fock_second_quantized_symbol} by reducing the momentum inside the
expected value {expected_value}.
The expected value {expected_value} is only nonzero when the two momenta
 $k_i,k_j$ are the same, namely, {expected_value_nonzero}.
You should use the property of Kronecker delta function $\delta_{{k_i,
k_j}}$ to reduce one momentum $k_i$.
Once you reduce one momentum inside the expected value $\langle\dots\
rangle$. You will also notice the total momentum conservation will
reduce another momentum in the quadratic term. Therefore, you should end
 up with only two momenta left in the summation.
You should follow the EXAMPLE below to reduce one momentum in the Fock
term, and another momentum in the quadratic term.
You should recall that {Fock_second_quantized_symbol} is {
expression_Fock}.
Return the final simplified Fock term {Fock_second_quantized_symbol}.

===
EXAMPLE:
Given a Hamiltonian where the Fock term $\hat{{H}}^{{Fock}}=-\sum_{{k_1,
k_2, k_3, k_4,s_1,s_2}} V(k_1-k_4) \langle c_{{s_1}}^\dagger(k_1) c_{{
s_2}}(k_3) \rangle c_{{s_2}}^\dagger(k_2) c_{{s_1}}(k_4)  \sum_{{G}}\
delta_{{k_1+k_2-k_3-k_4,G}}$, where $k_i$ is the momentum inside first
Brilloun zone, $G$ is the reciprocal lattice vectors, and $s_i$ is a
certain index for the degree of freedom other than momentum.
Inside the expected value, we realize $\langle c_{{s_1}}^\dagger(k_1) c_
{{s_2}}(k_3) \rangle$ is nonzero only when $k_1=k_3$, i.e., $\langle c_
{{s_1}}^\dagger(k_1) c_{{s_2}}(k_3) \rangle=\langle c_{{s_1}}^\dagger(
k_1) c_{{s_2}}(k_3) \rangle\delta_{{k_1,k_3}}$.
Thus, the Fock term becomes $-\sum_{{k_1,k_2, k_3, k_4,s_1,s_2}} V(k_1-
k_4) \langle c_{{s_1}}^\dagger(k_1) c_{{s_2}}(k_3) \rangle \delta_{{k_1,
k_3}} c_{{s_2}}^\dagger(k_2) c_{{s_1}}(k_4) \sum_{{G}}\delta_{{k_1+k_2-
k_3-k_4,G}}$.
Use the property of Kronecker delta function $\delta_{{k_1,k_3}}$ to sum
 over $k_3$, we have $-\sum_{{k_1,k_2, k_4,s_1,s_2}} V(k_1-k_4) \langle
c_{{s_1}}^\dagger(k_1) c_{{s_2}}(k_1) \rangle c_{{s_2}}^\dagger(k_2) c_
{{s_1}}(k_4) \sum_{{G}}\delta_{{k_2-k_4,G}}$.
We can further simplify $\sum_{{G}}\delta_{{k_2-k_4,G}}$. Because $k_i$
is momentum inside first Brilloun zone, and the difference between $k_2$
 and $k_4$ cannot exceed the first shell of reciprocal lattice vector,
which means $G$ can only take the value of the origin point in the
reciprocal lattice, therefore, $\sum_{{G}}\delta_{{k_2-k_4,G}}=\delta_{{
k_2-k_4,0}}$.
Thus, the Fock term simplifies to $-\sum_{{k_1,k_2, k_4,s_1,s_2}} V(k_1-
k_4) \langle c_{{s_1}}^\dagger(k_1) c_{{s_2}}(k_1) \rangle c_{{s_2}}^\
dagger(k_2) c_{{s_1}}(k_4) \delta_{{k_2-k_4,0}}=-\sum_{{k_1, k_2,s_1,s_2
```

```
}} V(k_1-k_2) \langle c_{{s_1}}^\dagger(k_1) c_{{s_2}}(k_1) \rangle c_{{
s_2}}^\dagger(k_2) c_{{s_1}}(k_2)$.
Therefore, the final simplified Fock term after reducing one momentum is
 $\hat{{H}}^{{Fock}}=-\sum_{{k_1, k_2,s_1,s_2}} V(k_1-k_2) \langle c_{{
s_1}}^\dagger(k_1) c_{{s_2}}(k_1) \rangle c_{{s_2}}^\dagger(k_2) c_{{s_1
}}(k_2)$
```

```
Final form of iteration in quadratic terms
**Prompt:**
You will now be instructed to combine the Hartree term {Hartree_symbol}
and the Fock term {Fock_symbol}.
You should recall that the Hartree term {Hartree},
and the Fock term {Fock}.
You should perform the same trick of relabeling the index in the Fock
term to make the quadratic operators in the Fock term the same as those
in the Hartree term. The relabeling should be done with a swap : {
swap_rule}.
You should add them, relabel the index in Fock term, and simply their
sum.
Return the final sum of Hartree and Fock term.
```

### 4. The generic workflow for three branches

We present the generic workflow for the three branches: (continuum, first-quantized), (lattice, second-quantized), and (continuum, second-quantized) in Table II. The background colors are consistent with the five conceptual steps as shown in Fig. 1 in the main text.

Note that for some specific papers, one or two steps may be dropped because they are unnecessary. For example, in Ref. [4], since only the Hartree term was considered, therefore, there is no need to "Identify order parameters in Fock term", and then obtain "Final form of iteration in quadratic terms" by combining the Hartree and Fock terms.

Figure 1 in the main text shows the branch for "lattice, second-quantized" because it is conceptually easy and also representative.

TABLE II: The generic workflow for the three branches

| Continuum, first-quantized | Lattice, second-quantized | Continuum, second-quanitzed |
|---|---|---|
| Identify kinetic term (continuum,first-quantized) | Identify kinetic term (lattice) | Identify kinetic term (continuum,second-quantized) |
| Define energy dispersion (continuum) | | Define energy dispersion (continuum) |
| Identify potential term (continuum) | | Identify potential term (continuum) |
| Define potential term (continuum) | | Define potential term (continuum) |
| Identify interacting term (momentum space) | Identify interacting term (real space) | Identify interacting term (momentum space) |
| Second-quantization (matrix) | | |
| Second-quantization (summation) | | |
| Fourier transform noninteracting term to momentum space (continuum) | Fourier transform noninteracting term to momentum space (lattice) | Fourier transform noninteracting term to momentum space (continuum) |
| | Fourier transform interacting term to momentum space (lattice) | |
| Wick's theorem expansion | Wick's theorem expansion | Wick's theorem expansion |
| Drop constant terms | Drop constant terms | Drop constant terms |
| Identify momentum transfer in interaction | Identify momentum transfer in interaction | Identify momentum transfer in interaction |
| Combine Hartree/Fock terms | Combine Hartree/Fock terms | Combine Hartree/Fock terms |
| Identify order parameters in Hartree term | Identify order parameters in Hartree term | Identify order parameters in Hartree term |
| Identify order parameters in Fock term | Identify order parameters in Fock term | Identify order parameters in Fock term |
| Final form of iteration in quadratic terms | Final form of iteration in quadratic terms | Final form of iteration in quadratic terms |

### D. API Execution for Annotated-Excerpt based execution

The GPT-4 model we query via the API has a context window of 8192 tokens, which is not large enough to accommodate the entire sequence of tasks in the execution stage. Therefore, instead of simply prompting using all existing history, i.e.,

1. [Prompt 1] $\xRightarrow{\text{GPT4}}$ [Prompt1, Completion 1]

2. [Prompt 1, Completion 1, Prompt 2] $\xRightarrow{\text{GPT4}}$ [Prompt 1, Completion 1, Prompt 2, Answers 2]

   ...

$N$. [Prompt 1, Completion 1, Prompt 2, ... Prompt $N$] $\xRightarrow{\text{GPT4}}$ [Prompt 1, Completion 1, Prompt 2, ... Prompt $N$, Completion $N$-1],

We employ GPT-4 API to also summarize all previous contents to prevent the history from growing too long and work within the 8k token limit. Namely, the API call will be in the order of

1. [Prompt 1] $\xrightarrow{\text{GPT4: Solver}}$ [Prompt1, Completion 1]

2. [Prompt 1, Completion 1] $\xrightarrow{\text{GPT4: Summarizer}}$ [Summary 1]

3. [Summary 1, Prompt 2] $\xrightarrow{\text{GPT4: Solver}}$ [Summary 1, Prompt 2, Completion 2]

4. [Summary 1, Prompt 2, Completion 2] $\xrightarrow{\text{GPT4: Summarizer}}$ [Summary 2]

5. [Summary 2, Prompt 3] $\xrightarrow{\text{GPT4: Solver}}$ [Summary 2, Prompt 3, Completion 3]

...

$2N-1$. [Summary $N$-1, Prompt $N$] $\xrightarrow{\text{GPT4: Solver}}$ [Summary $N$-1, Prompt $N$, Completion $N$]

This summarizer has the following prompt, where the curvy brackets are the placeholders for the previous background

~~~~
Below is a conversation about a physics problem showing after ```.
The format is 1. Background of the question. 2: Question. 3: Answer.
You should summarize the history.
You should remove redundant information, and keep the main physics, especially, paying attention to the latex equations.
Return the summarized text.
```
**Background**
{background}

**Question**
question

**Answer**
answer
```
~~~~

### E. Abstract-based Execution

In Fig. 1 in the main text, we present an "Abstract-based Execution" example, where we fix the notation used in the paper (since it is not related to the essence of physics), and aim to extract essential physics-related information directly from the abstract. This process resulted in identifying 10 key placeholders (listed in the first column of Table III), for which we formulated 10 corresponding questions (outlined in the second column of Table III).

In the third column, we document the rough accuracy of how GPT-4 performs on each question. The accuracy is estimated as $1/T$, where $T$ the number of trials until success.

Since GPT-4 did not answer perfectly for all questions, we manually rerun it several times until the correct answer appeared when querying these 10 questions (note that no rerun is done for tasks in the execution stage). The concatenation of all correct answers composed the best run results as shown below.

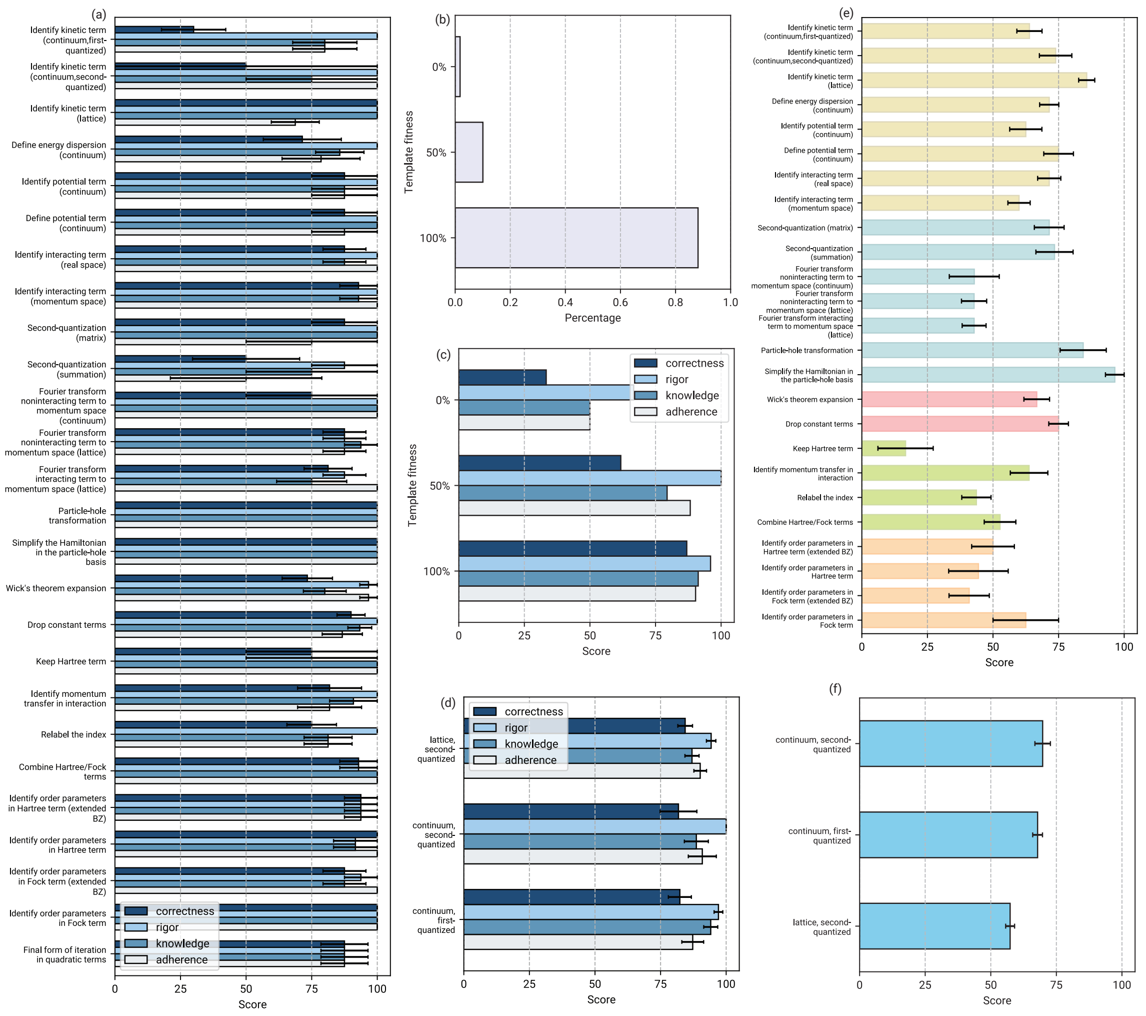


SFig. 1: (a) The performance of the execution results from the four aspects for all prompts; (b) Most prompts (> 80%) fit the prompt templates well; (c) The performance of the execution results given the template fitness from the four aspects. The better scores from the good fitness indicate that template fitness is a crucial factor; (d) The performance of the execution results from the four aspects for all branches of papers. The similar performance indicates that the execution results are generically good for all branches of paper; (e) The performance of the information extraction results for all prompts; (f) The performance of the information extraction results from the four aspects for all branches of papers.

TABLE III: 10 placeholders for the extraction from abstract

| Placeholder | Questions | Accuracy |
|---|---|---|
| system | What is the system to study? | 100% |
| degrees_of_freedom | What are the independent degrees of freedom that should be included in the Hamiltonian, namely, the independent flavor of the creation/annihilation operator? Remember the system is spin-valley locked. | 100% |
| parabolic\|Dirac\|cos | What should the energy dispersion of the kinetic term be like in this system? Choose from parabolic, Dirac, or cos-like. | 100% |
| electrons\|holes | Does the dispersion characterize electrons or holes in this system? | 100% |
| potential_degrees_of_freedom | When constructing the potential term for such system, which two components of flavor can mix? Namely, Is there a mixing between opposite valleys? Is there a mixing between opposite layers? | 100% |
| expression_diag | What is the mathematical formula of the diagonal terms in the noninteracting moire potential term written in real space? Combine with your a priori knowledge when necessary. | $\sim$33% |
| expression_offdiag | What is the mathematical formula of the off-diagonal terms (which mixes the top and bottom layers) in the moire potential term written in real space? Combine with your a priori knowledge when necessary. | $\sim$33% |
| interaction | What type of interaction should be used in the system? Remember the actual experimental device is usually dual-gated. | 100% |
| int_form | What is the mathematical formula for this interaction used in the Hamiltonian? You write it in the momentum space. Remember the interaction is a dual-gated screened Coulomb interaction (i.e., like a two-slab capacitor). | $\sim$50% |
| Not a placeholder | Do you need to keep both Hartree term and fock term in order to solve the problem in this paper? | 100% |

# 1 Preamble

## 1.1 One-shot Example

### 1.1.1

**Prompt:** I am reading a paper with the following abstract. I want you to first extract the essential information from it and then execute my instructions in order to create the Hamiltonian in the Hartree Fock Approximation.

To extract information, I will provide you with a set of questions about the calculation (this type of prompt will start with **Extraction**). You should first try your best to answer them. You should first quote the relevant part from the abstract which you think can lead to an answer. Then, you provide your rationale from this quote to the answer. Finally, you should give a succinct final version of the answer.

To execute the calculation, I will provide a set of tasks. You should follow the instructions strictly. Your reply should be succinct while complete. You should not expand any unwanted content. You will be learning background knowledge by examples if necessary.

A crucial part of execution is two-step: (1) fill in the paper-specific information from the extraction into a provided template (this prompts will start with **Execution–Core information**); (2) combine with the predetermined notations provided by me (this prompts will start with **Execution–Notation**), and then, you should proceed to execute the instruction. Note that there might be cases where no paper-specific information is needed from the abstract in certain execution tasks.

I will provide three examples (Example 1, Example 2, and Example 3) for **Extraction**, **Execution–Core information**, and **Execution**–Notation**, respectively, for you to learn. Confirm and repeat your duty if you understand it.

Example 1

"‘

**Extraction Abstract** We present a theory on the quantum phase diagram of AB-stacked $MoTe_2/WSe_2$ using a self-consistent Hartree-Fock calculation performed in the plane-wave basis, motivated by the observation of topological states in this system. At filling factor $\nu = 2$ (two holes per moir’e unit cell), Coulomb interaction can stabilize a $\mathbb{Z}_2$ topological insulator by opening a charge gap. At $\nu = 1$, the interaction induces three classes of competing states, spin density wave states, an in-plane ferromagnetic state, and a valley polarized state, which undergo first-order phase transitions tuned by an out-of-plane displacement field. The valley polarized state becomes a Chern insulator for certain displacement fields. Moreover, we predict a topological charge density wave forming a honeycomb lattice with ferromagnetism at $\nu = 2/3$. Future directions on this versatile system hosting a rich set of quantum phases are discussed.

**Question**: 1. What are the degrees of freedom that should be included in the Hamiltonian? 2. [Another question]

"‘

You response should be:

"‘

1. What are the degrees of freedom that should be included in the Hamiltonian? **Quote**: AB-stacked $MoTe_2/WSe_2$ **Explanation**: First the studied system is $MoTe_2/WSe_2$ , which is a heterostructure of bilayer. Therefore, layer is a degree of freedom that should be included in the Hamiltonian. Secod, because $MoTe_2$ and $WSe_2$ are both TMD materials which have strong Ising type spin orbit coupling. This coupling ties the electron’s spin to its valley index, resulting in distinct energy levels for spins aligned parallel or antiparallel to the orbital angular momentum. Since $MoTe_2$ and $WSe_2$ usually have the topmost valence band at +K/-K valley. This means the valley index is coupled to the spin index. Therefore, only two types of degrees of freedom (layer and valley) should be considered in the Hamiltonian. **Anwser**: layer, valley
2. [Another question] [Another answer]

"‘

Example 2

"‘

**Execution–Core information** You should fill in the specific information from above into the following template, and then repeat it. ”’

You will be instructed to describe the kinetic term of Hamiltonian in{system of interest}.

The degrees of freedom of the system are:{independent degree of freedom} ”’ "‘

Your response should be:

"‘

You will be instructed to describe the kinetic term of Hamiltonian in AB-stacked $MoTe_2/WSe_2$. The degrees of freedom of the system are: Layer and the combined spin-valley degree.

"‘

Example 3

"‘

**Execution: Notation** Here I provide the notation you should use for this task. You should combine it with previous **Execution: Core information** to obtain the full instruction for execution. In the response, you will first repeat the instruction

for execution and then proceed with the calculation. "' Express the Kinetic Hamiltonian $H_T$ using $E_{+K,b}$, $E_{-K,t}$, $E_{-K,b}$, $E_{-K,t}$ which are only on the diagonal terms, and arrange the basis in the order of (+K,bottom), (+K,top), (-K,bottom), (-K,top).

Use the following conventions for the symbols:

$\tau = \pm 1$ represents $\pm K$ valleys, bottom layer ($\mathfrak{b}$) and top layer ($\mathfrak{t}$)

"'

"'

Your response should be:

"'

**Instructions to execute**: You will be instructed to describe the kinetic term of Hamiltonian in AB-stacked $MoTe_2/WSe_2$. The degrees of freedom of the system are: Layer and the combined spin-valley degree. Express the Kinetic Hamiltonian $H_T$ using $E_{+K,b}$, $E_{-K,t}$, $E_{-K,b}$, $E_{-K,t}$ which are only on the diagonal terms, and arrange the basis in the order of (+K,bottom), (+K,top), (-K,bottom), (-K,top).

Use the following conventions for the symbols:

$\tau = \pm 1$ represents $\pm K$ valleys, bottom layer ($\mathfrak{b}$) and top layer ($\mathfrak{t}$)

**Answer** [The answer to the above 'Instructions to execute'] "'

#### 1.1.2

**Completion:** I understand my duties as follows:

1. **Extraction**: When provided with an abstract or excerpt from a paper, I will extract essential information by:

- Quoting relevant parts of the abstract.
- Providing a rationale from this quote to the answer.
- Giving a succinct final version of the answer.

2. **Execution - Core Information**: I will fill in paper-specific information from the extraction into a provided template and then repeat the filled-in template.

3. **Execution - Notation**: I will combine the provided notation with the "Execution - Core Information" to execute the instruction. The response will include:

- Repeating the instruction for execution.
- Proceeding with the calculation or explanation as required.

Let's proceed with your instructions.

# 2 Identify kinetic term (continuum,first-quantized)

## 2.1 Extraction

#### 2.1.1

**Prompt: Extraction Abstract** We present a theory on the quantum phase diagram of AB-stacked $MoTe_2/WSe_2$ using a self-consistent Hartree-Fock calculation performed in the plane-wave basis, motivated by the observation of topological states in this system. At filling factor $\nu = 2$ (two holes per moir'e unit cell), Coulomb interaction can stabilize a $\mathbb{Z}_2$ topological insulator by opening a charge gap. At $\nu = 1$, the interaction induces three classes of competing states, spin density wave states, an in-plane ferromagnetic state, and a valley polarized state, which undergo first-order phase transitions tuned by an out-of-plane displacement field. The valley polarized state becomes a Chern insulator for certain displacement fields. Moreover, we predict a topological charge density wave forming a honeycomb lattice with ferromagnetism at $\nu = 2/3$. Future directions on this versatile system hosting a rich set of quantum phases are discussed.

**Question**: 1. What is the system to study? 2. What are the independent degrees of freedom that should be included in the Hamiltonian, namely, the independent flavor of the creation/annihilation operator? Remember the system is spin-valley locked.

#### 2.1.2

**Completion:** 1. **What is the system to study? Quote**: "AB-stacked $MoTe_2/WSe_2$" **Explanation**: The system under study is explicitly stated in the abstract as "AB-stacked $MoTe_2/WSe_2$". This refers to a heterostructure composed of layers of $MoTe_2$ and $WSe_2$ materials, arranged in an AB stacking configuration. **Answer**: AB-stacked $MoTe_2/WSe_2$.

2. **What are the independent degrees of freedom that should be included in the Hamiltonian, namely, the independent flavor of the creation/annihilation operator? Remember the system is spin-valley locked.** **Quote**: "the observation of topological states in this system" and "spin density wave states, an in-plane ferromagnetic state, and a valley polarized state" **Explanation**: The abstract mentions topological states, spin density waves, ferromagnetic states, and valley polarization in the AB-stacked $MoTe_2/WSe_2$ system. Since the system is spin-valley locked, the spins and valleys are not independent degrees of freedom; they are coupled. This coupling implies that the spin and valley degrees of freedom cannot be varied independently and are considered as one combined degree of freedom in the Hamiltonian. **Answer**: The independent degrees of freedom in the Hamiltonian are the combined spin-valley degree and the layer degree (from the AB-stacked configuration).

## 2.2 Execution–Core information

### 2.2.1

**Prompt: Execution–Core information** You should fill in the specific information from above into the following template, and then repeat it. "' You will be instructed to describe the kinetic term of Hamiltonian in {system of study}. The degrees of freedom of the system are: {independent degree of freedom} "'

### 2.2.2

**Completion:** You will be instructed to describe the kinetic term of the Hamiltonian in AB-stacked $MoTe_2/WSe_2$. The degrees of freedom of the system are: the combined spin-valley degree and the layer degree.

## 2.3 Execution: Notation:

### 2.3.1

**Prompt: Execution: Notation** Here I provide the notation you should use for this task. You should combine it with previous **Execution: Core information** to obtain the full instruction for execution. In the response, you will first repeat the instruction for execution and then proceed with the calculation. "' Express the Kinetic Hamiltonian $H_T$ using $E_{+K,b}$, $E_{-K,t}$, $E_{-K,b}$, $E_{-K,t}$ which are only on the diagonal terms, and arrange the basis in the order of (+K,bottom), (+K,top), (-K,bottom), (-K,top).

Use the following conventions for the symbols:

$\tau = \pm 1$ represents $\pm K$ valleys, bottom layer ($\mathfrak{b}$) and top layer ($\mathfrak{t}$) "'

### 2.3.2

**Completion: Instructions to execute**: You will be instructed to describe the kinetic term of the Hamiltonian in AB-stacked $MoTe_2/WSe_2$. The degrees of freedom of the system are: the combined spin-valley degree and the layer degree. Express the Kinetic Hamiltonian $H_T$ using $E_{+K,b}$, $E_{-K,t}$, $E_{-K,b}$, $E_{-K,t}$, which are only on the diagonal terms, and arrange the basis in the order of (+K,bottom), (+K,top), (-K,bottom), (-K,top).

Use the following conventions for the symbols:

$\tau = \pm 1$ represents $\pm K$ valleys, bottom layer ($\mathfrak{b}$) and top layer ($\mathfrak{t}$).

**Answer**: The kinetic Hamiltonian $H_T$ for the AB-stacked $MoTe_2/WSe_2$ system with the considered degrees of freedom can be expressed in a matrix form as follows:

$$H_T = \begin{pmatrix} E_{+K,b} & 0 & 0 & 0 \\ 0 & E_{+K,t} & 0 & 0 \\ 0 & 0 & E_{-K,b} & 0 \\ 0 & 0 & 0 & E_{-K,t} \end{pmatrix} \tag{1}$$

In this matrix: - The diagonal elements represent the energy levels for each state. - $E_{+K,b}$ and $E_{+K,t}$ are the energy levels at the +K valley for the bottom and top layers, respectively. - $E_{-K,b}$ and $E_{-K,t}$ are the energy levels at the -K valley for the bottom and top layers, respectively. - The off-diagonal elements are all zero, indicating no direct coupling between these states in the kinetic term of the Hamiltonian.

# 3 Define energy dispersion (continuum)

## 3.1 Extraction

### 3.1.1

**Prompt: Extraction Extraction Abstract** We present a theory on the quantum phase diagram of AB-stacked $MoTe_2/WSe_2$ using a self-consistent Hartree-Fock calculation performed in the plane-wave basis, motivated by the observation of topological states in this system. At filling factor $\nu = 2$ (two holes per moir'e unit cell), Coulomb interaction can stabilize a $\mathbb{Z}_2$ topological insulator by opening a charge gap. At $\nu = 1$, the interaction induces three classes of competing states, spin density wave states, an in-plane ferromagnetic state, and a valley polarized state, which undergo first-order phase transitions tuned by an out-of-plane displacement field. The valley polarized state becomes a Chern insulator for certain displacement fields. Moreover, we predict a topological charge density wave forming a honeycomb lattice with ferromagnetism at $\nu = 2/3$. Future directions on this versatile system hosting a rich set of quantum phases are discussed.

**Question**: 1. What should the energy dispersion of the kinetic term be like in this system? Choose from parabolic, Dirac, or cos-like. 2. Does the dispersion characterize electrons or holes in this system?

### 3.1.2

**Completion:** 1. **What should the energy dispersion of the kinetic term be like in this system? Choose from parabolic, Dirac, or cos-like. Quote**: "using a self-consistent Hartree-Fock calculation performed in the plane-wave basis" **Explanation**: The mention of a plane-wave basis in the Hartree-Fock calculation suggests that the energy dispersion in this system is likely to be parabolic. In solid-state physics, a plane-wave basis is often used to describe free electrons, which have a parabolic energy dispersion. While the abstract does not explicitly describe the dispersion type, the use of a plane-wave basis is a strong indicator of parabolic dispersion, as it is a common approach for systems where electron behavior can be approximated as free particle-like. **Answer**: The energy dispersion of the kinetic term in this system should be parabolic.

2. **Does the dispersion characterize electrons or holes in this system? Quote**: "At filling factor $\nu = 2$ (two holes per moiré unit cell)" **Explanation**: The abstract specifically mentions "two holes per moiré unit cell" at a filling factor $\nu = 2$. This indicates that the dispersion characterizes holes rather than electrons in this system. In semiconductor physics, when discussing holes, it is often in the context of the absence of an electron in an otherwise filled band, which affects the electronic properties of the material. **Answer**: The dispersion characterizes holes in this system.

## 3.2 Execution-Core Information

### 3.2.1

**Prompt: Execution–Core information** You should fill in the specific information from above into the following template, and then repeat it. "' For all energy dispersions, they characterize the {energy dispersion}. dispersion for {electron or hole}. "'

### 3.2.2

**Completion:** For all energy dispersions, they characterize the parabolic dispersion for holes.

## 3.3 Execution-Notation

### 3.3.1

**Prompt: Execution: Notation** Here I provide the notation you should use for this task. You should combine it with previous **Execution: Core information** to obtain the full instruction for execution. In the response, you will first repeat the instruction for execution and then proceed with the calculation. "' You will be instructed to construct each term, namely $E_{+K,b}$, $E_{-K,t}$, $E_{-K,b}$, $E_{-K,t}$.

In addition, a shift of $+\kappa$ and $-\kappa$ in the momentum $\boldsymbol{k}$ for $E_{t,+K}$ and $E_{t,-K}$, respectively.

You should follow the EXAMPLE below to obtain the correct energy dispersion, select the correct EXAMPLE by noticing the type of dispersion.

Finally, in the real space, the momentum $\boldsymbol{k} = -i\partial_{\boldsymbol{r}}$. You should keep the form of $\boldsymbol{k}$ in the Hamiltonian for short notations but should remember $\boldsymbol{k}$ is an operator.

You should recall that

$$H_T = \begin{pmatrix} E_{+K,b} & 0 & 0 & 0 \\ 0 & E_{+K,t} & 0 & 0 \\ 0 & 0 & E_{-K,b} & 0 \\ 0 & 0 & 0 & E_{-K,t} \end{pmatrix} \tag{2}$$

.

Return the expression for $E_{+K,b}$, $E_{-K,t}$, $E_{-K,b}$, $E_{-K,t}$ in the Kinetic Hamiltonian, and substitute it into the Kinetic Hamiltonian $H_T$.

Use the following conventions for the symbols (You should also obey the conventions in all my previous prompts if you encounter undefined symbols. If you find it is never defined or has conflicts in the conventions, you should stop and let me know):

$\boldsymbol{\kappa} = \frac{4\pi}{3a_M}(1,0)$ is at a corner of the moir'e Brillouin zone, $(m_{\mathfrak{b}}, m_{\mathfrak{t}}) = (0.65, 0.35)m_e$ ($m_e$ is the rest electron mass)

===

EXAMPLE 1:

A parabolic dispersion for electron is $E_\alpha = \frac{\hbar^2 k^2}{2m_\alpha}$, where $\alpha$ indicates the type of electron. If there is a further shift of $q$ in the momentum $k$, the dispersion will become $E_\alpha = \frac{\hbar^2 (k-q)^2}{2m_\alpha}$.

EXAMPLE 2: A cos dispersion is $E_\alpha = -\cos(ka/2)$, where $\alpha$ indicates the type of particle. If there is a further shift of $q$ in the momentum $k$, the dispersion will become $E_\alpha = -\cos((k-q)a/2))$. However, there could be more prefactors before cos depending on the geometry of the lattice.

EXAMPLE 3:

A dirac dispersion for electron/hole is a 2 by 2 matrix, i.e., $h_\theta(k) = -\hbar v_D |k| \begin{pmatrix} 0 & e^{i(\theta_k - \theta)} \\ e^{-i(\theta_{\bar{k}} - \theta)} & 0 \end{pmatrix}$, where $v_D$ is the Fermi velocity, $\theta$ is the twist angle, and $\theta_k$ indicates the azumith angle of $k$. If there is a further shift of $K_\theta$ in the momentum $k$, the dispersion will become $h_\theta(k) = -\hbar v_D |k - K_\theta| \begin{pmatrix} 0 & e^{i(\theta_{k-K_\theta} - \theta)} \\ e^{-i(\theta_{k-K_\theta} - \theta)} & 0 \end{pmatrix}$. ",'

### 3.3.2

**Completion: Instructions to execute**: For all energy dispersions, they characterize the parabolic dispersion for holes. You will be instructed to construct each term, namely $E_{+K,b}$, $E_{-K,t}$, $E_{-K,b}$, $E_{-K,t}$, with a shift of $+\kappa$ and $-\kappa$ in the momentum $\boldsymbol{k}$ for $E_{t,+K}$ and $E_{t,-K}$, respectively. You should follow the parabolic dispersion for holes as in Example 1 to obtain the correct energy dispersion. In real space, the momentum $\boldsymbol{k} = -i\partial_{\boldsymbol{r}}$. Keep the form of $\boldsymbol{k}$ in the Hamiltonian for short notations but remember $\boldsymbol{k}$ is an operator. Recall that

$$H_T = \begin{pmatrix} E_{+K,b} & 0 & 0 & 0 \\ 0 & E_{+K,t} & 0 & 0 \\ 0 & 0 & E_{-K,b} & 0 \\ 0 & 0 & 0 & E_{-K,t} \end{pmatrix}. \tag{3}$$

Use the following conventions for the symbols: $\boldsymbol{\kappa} = \frac{4\pi}{3a_M}(1,0)$ is at a corner of the moiré Brillouin zone, $(m_{\mathfrak{b}}, m_{\mathfrak{t}}) = (0.65, 0.35)m_e$ ($m_e$ is the rest electron mass).

**Answer**: Since the system describes holes with a parabolic dispersion, the dispersion relation is the inverse of that for electrons. Therefore, for a hole, the energy dispersion is $E_\alpha = -\frac{\hbar^2 k^2}{2m_\alpha}$ (negative sign because we are dealing with holes).

Considering the shifts in momentum for top layer terms, the expressions for each energy term will be: - $E_{+K,b} = -\frac{\hbar^2 k^2}{2m_{\mathfrak{b}}}$ - $E_{+K,t} = -\frac{\hbar^2 (k+\boldsymbol{\kappa})^2}{2m_{\mathfrak{t}}}$ - $E_{-K,b} = -\frac{\hbar^2 k^2}{2m_{\mathfrak{b}}}$ - $E_{-K,t} = -\frac{\hbar^2 (k-\boldsymbol{\kappa})^2}{2m_{\mathfrak{t}}}$

Substituting these into the kinetic Hamiltonian $H_T$, we get:

$$H_T = \begin{pmatrix} -\frac{\hbar^2 k^2}{2m_{\mathfrak{b}}} & 0 & 0 & 0 \\ 0 & -\frac{\hbar^2 (k+\boldsymbol{\kappa})^2}{2m_{\mathfrak{t}}} & 0 & 0 \\ 0 & 0 & -\frac{\hbar^2 k^2}{2m_{\mathfrak{b}}} & 0 \\ 0 & 0 & 0 & -\frac{\hbar^2 (k-\boldsymbol{\kappa})^2}{2m_{\mathfrak{t}}} \end{pmatrix} \tag{4}$$

Here, $\boldsymbol{k}$ remains as an operator, and the energy terms account for the parabolic dispersion of holes with the given mass parameters and momentum shifts.

# 4 Identify potential term (continuum)

## 4.1 Extraction

### 4.1.1

**Prompt: Extraction Abstract** We present a theory on the quantum phase diagram of AB-stacked $MoTe_2/WSe_2$ using a self-consistent Hartree-Fock calculation performed in the plane-wave basis, motivated by the observation of topological states in this system. At filling factor $\nu = 2$ (two holes per moir'e unit cell), Coulomb interaction can stabilize a $\mathbb{Z}_2$ topological insulator

by opening a charge gap. At $\nu = 1$, the interaction induces three classes of competing states, spin density wave states, an in-plane ferromagnetic state, and a valley polarized state, which undergo first-order phase transitions tuned by an out-of-plane displacement field. The valley polarized state becomes a Chern insulator for certain displacement fields. Moreover, we predict a topological charge density wave forming a honeycomb lattice with ferromagnetism at $\nu = 2/3$. Future directions on this versatile system hosting a rich set of quantum phases are discussed.

**Question**: 1. When constructing the potential term for such system, which two components of flavor can mix? Namely, Is there a mixing between opposite valleys? Is there a mixing between opposite layers?

#### 4.1.2

**Completion:** 1. **When constructing the potential term for such a system, which two components of flavor can mix? Namely, is there a mixing between opposite valleys? Is there a mixing between opposite layers? Quote**: "At $\nu = 1$, the interaction induces three classes of competing states, spin density wave states, an in-plane ferromagnetic state, and a valley polarized state, which undergo first-order phase transitions tuned by an out-of-plane displacement field." **Explanation**: The mention of "valley polarized state" suggests that there is distinct behavior associated with different valleys, indicating that the valleys are a significant factor in the system's physics. However, the absence of explicit mention of mixing between opposite valleys in the abstract suggests that such mixing might not be a primary focus in this system. On the other hand, the reference to phase transitions "tuned by an out-of-plane displacement field" implies that there could be interactions or effects that involve both layers, as an out-of-plane field would affect the system in a direction perpendicular to the layers. This could hint at possible mixing between layers, depending on the nature of these interactions. **Answer**: There is likely no significant mixing between opposite valleys as implied by the focus on valley polarization, but there could be mixing between opposite layers, as suggested by the influence of the out-of-plane displacement field.

### 4.2 Execution-Core Information

#### 4.2.1

**Prompt: Execution–Core information** You should fill in the specific information from above into the following template, and then repeat it.

The off-diagonal terms are the coupling between Mixing between {flavors}.

#### 4.2.2

**Completion:** The off-diagonal terms are the coupling between mixing between opposite layers.

### 4.3 Execution-Notation

#### 4.3.1

**Prompt: Execution: Notation** Here I provide the notation you should use for this task. You should combine it with previous **Execution: Core information** to obtain the full instruction for execution. In the response, you will first repeat the instruction for execution and then proceed with the calculation. "' You will be instructed to describe the potential term of Hamiltonian $H_V$ in the real space in the single-particle form.

The potential Hamiltonian has the same degrees of freedom as the kinetic Hamiltonian.

The diagonal terms are $\Delta_t(r)$ and $\Delta_b(r)$.

The off-diagonal terms are $\Delta_{\mathrm{T},\tau}(\boldsymbol{r})$ and $\Delta_{\mathrm{T},\tau}^{\dagger}(\boldsymbol{r})$, which should be kept hermitian.

All other terms are zero. Express the potential Hamiltonian $H_V$ using $\Delta_t(r)$ and $\Delta_b(r)$ and $\Delta_{\mathrm{T},\tau}(\boldsymbol{r})$ and $\Delta_{\mathrm{T},\tau}^{\dagger}(\boldsymbol{r})$.

"'

#### 4.3.2

**Completion: Instructions to execute**: You will be instructed to describe the potential term of Hamiltonian $H_V$ in the real space in the single-particle form. The potential Hamiltonian has the same degrees of freedom as the kinetic Hamiltonian. The diagonal terms are $\Delta_t(r)$ and $\Delta_b(r)$. The off-diagonal terms are $\Delta_{\mathrm{T},\tau}(\boldsymbol{r})$ and $\Delta_{\mathrm{T},\tau}^{\dagger}(\boldsymbol{r})$, which should be kept hermitian. All other terms are zero. Express the potential Hamiltonian $H_V$ using $\Delta_t(r)$ and $\Delta_b(r)$ and $\Delta_{\mathrm{T},\tau}(\boldsymbol{r})$ and $\Delta_{\mathrm{T},\tau}^{\dagger}(\boldsymbol{r})$. The off-diagonal terms are the coupling between mixing between opposite layers.

**Answer**: The potential Hamiltonian $H_V$ in the real space for the AB-stacked $MoTe_2/WSe_2$ system, considering the specified degrees of freedom and the hermitian nature of the off-diagonal terms, can be expressed as:

$$H_V = \begin{pmatrix} \Delta_b(r) & \Delta_{\mathrm{T},\tau}(\boldsymbol{r}) & 0 & 0 \\ \Delta_{\mathrm{T},\tau}^\dagger(\boldsymbol{r}) & \Delta_t(r) & 0 & 0 \\ 0 & 0 & \Delta_b(r) & \Delta_{\mathrm{T},\tau}(\boldsymbol{r}) \\ 0 & 0 & \Delta_{\mathrm{T},\tau}^\dagger(\boldsymbol{r}) & \Delta_t(r) \end{pmatrix} \tag{5}$$

In this matrix: - $\Delta_b(r)$ and $\Delta_t(r)$ are the potential terms for the bottom and top layers respectively, which appear on the diagonal. - $\Delta_{\mathrm{T},\tau}(\boldsymbol{r})$ and its hermitian conjugate $\Delta_{\mathrm{T},\tau}^\dagger(\boldsymbol{r})$ are the off-diagonal terms that represent the coupling between the opposite layers. - The zero terms represent no direct potential coupling between other combinations of degrees of freedom.

# 5 Define potential term (continuum)

## 5.1 Extraction

### 5.1.1

**Prompt: Extraction Abstract** We present a theory on the quantum phase diagram of AB-stacked $MoTe_2/WSe_2$ using a self-consistent Hartree-Fock calculation performed in the plane-wave basis, motivated by the observation of topological states in this system. At filling factor $\nu = 2$ (two holes per moir'e unit cell), Coulomb interaction can stabilize a $\mathbb{Z}_2$ topological insulator by opening a charge gap. At $\nu = 1$, the interaction induces three classes of competing states, spin density wave states, an in-plane ferromagnetic state, and a valley polarized state, which undergo first-order phase transitions tuned by an out-of-plane displacement field. The valley polarized state becomes a Chern insulator for certain displacement fields. Moreover, we predict a topological charge density wave forming a honeycomb lattice with ferromagnetism at $\nu = 2/3$. Future directions on this versatile system hosting a rich set of quantum phases are discussed.

**Question**: 1. What is the mathematical formula of the diagonal terms in the noninteracting moire potential term written in real space? Combine with your a priori knowledge when necessary. 2. What is the mathematical formula of the off-diagonal terms (which mixes the top and bottom layers) in the moire potential term written in real space? Combine with your a priori knowledge when necessary.

### 5.1.2

**Completion:** 1. **What is the mathematical formula of the diagonal terms in the noninteracting moire potential term written in real space? Quote**: None directly relevant to the mathematical formula of the diagonal terms in the noninteracting moire potential term. **Explanation**: The abstract does not provide a specific formula for the diagonal terms of the moire potential. However, based on a priori knowledge about moire potentials in similar systems, the diagonal terms usually represent the potential energy landscape in each layer. For a system like AB-stacked $MoTe_2/WSe_2$, the moire potential is typically a periodic function reflecting the moire superlattice structure. It can be represented mathematically as a sum of cosines corresponding to the periodicity of the moire pattern. **Answer**: A typical form for the diagonal terms in the moire potential, written in real space, could be:

$$\Delta_\alpha(r) = V_0 \sum_{i=1}^{3} \cos(\boldsymbol{G}_i \cdot \boldsymbol{r} + \phi_\alpha) \tag{6}$$

where $\alpha$ is either the top or bottom layer, $V_0$ is the potential strength, $\boldsymbol{G}_i$ are the reciprocal lattice vectors of the moire pattern, $\boldsymbol{r}$ is the position vector, and $\phi_\alpha$ is a phase shift that may differ between layers.

2. **What is the mathematical formula of the off-diagonal terms (which mixes the top and bottom layers) in the moire potential term written in real space? Quote**: None directly relevant to the mathematical formula of the off-diagonal terms. **Explanation**: Similar to the diagonal terms, the abstract does not provide explicit information about the mathematical form of the off-diagonal terms of the moire potential. However, the off-diagonal terms in a moire potential usually represent tunneling or coupling between layers. These terms are often modeled as a spatially varying function that depends on the alignment and the periodicity of the layers. **Answer**: A typical form for the off-diagonal terms in the moire potential, which mix the top and bottom layers and are written in real space, could be modeled as:

$$\Delta_{\mathrm{T},\tau}(\boldsymbol{r}) = T_0 \sum_{i=1}^{3} e^{i\boldsymbol{G}_i \cdot \boldsymbol{r}} \tag{7}$$

where $T_0$ is the tunneling strength, and $\boldsymbol{G}_i$ are the reciprocal lattice vectors of the moire pattern. This term allows for spatially dependent coupling between the layers.

### 5.2 Execution-Core Information

#### 5.2.1

**Prompt: Execution–Core information** You should fill in the specific information from above into the following template, and then repeat it. "' The expression for diagonal terms are: {diagonal terms} The expression for off-diagonal terms are: {offdiagonal terms} "'

#### 5.2.2

**Completion:** The expression for diagonal terms are:

$$\Delta_\alpha(r) = V_0 \sum_{i=1}^{3} \cos(\boldsymbol{G}_i \cdot \boldsymbol{r} + \phi_\alpha) \tag{8}$$

The expression for off-diagonal terms are:

$$\Delta_{\mathrm{T},\tau}(\boldsymbol{r}) = T_0 \sum_{i=1}^{3} e^{i\boldsymbol{G}_i \cdot \boldsymbol{r}} \tag{9}$$

### 5.3 Execution-Notation

#### 5.3.1

**Prompt: Execution: Notation** Here I provide the notation you should use for this task. You should combine it with previous **Execution: Core information** to obtain the full instruction for execution. In the response, you will first repeat the instruction for execution and then proceed with the calculation. "' You will be instructed to construct each term $H_V$, namely, $\Delta_t(r)$, $\Delta_b(r)$ , $\Delta_{\mathrm{T},\tau}(\boldsymbol{r})$ and $\Delta^\dagger_{\mathrm{T},\tau}(\boldsymbol{r})$.

You should recall that

$$H_V = \begin{pmatrix} \Delta_b(r) & \Delta_{\mathrm{T},+K}(\boldsymbol{r}) & 0 & 0 \\ \Delta^\dagger_{\mathrm{T},+K}(\boldsymbol{r}) & \Delta_t(r) & 0 & 0 \\ 0 & 0 & \Delta_b(r) & \Delta_{\mathrm{T},-K}(\boldsymbol{r}) \\ 0 & 0 & \Delta^\dagger_{\mathrm{T},-K}(\boldsymbol{r}) & \Delta_t(r) \end{pmatrix} \tag{10}$$

.Return the expressions for $\Delta_t(r)$, $\Delta_b(r)$ , $\Delta_{\mathrm{T},\tau}(\boldsymbol{r})$ and $\Delta^\dagger_{\mathrm{T},\tau}(\boldsymbol{r})$, and substitute it into the potential Hamiltonian $H_V$.

Use the following conventions for the symbols (You should also obey the conventions in all my previous prompts if you encounter undefined symbols. If you find it is never defined or has conflicts in the conventions, you should stop and let me know):the off diagonal terms describe the interlayer tunneling $\Delta_{\mathrm{T},\tau}$, intralayer potential $\Delta_{\mathfrak{b}/\mathfrak{t}}$ "'

#### 5.3.2

**Completion: Instructions to execute**: You will be instructed to construct each term $H_V$, namely, $\Delta_t(r)$, $\Delta_b(r)$, $\Delta_{\mathrm{T},\tau}(\boldsymbol{r})$ and $\Delta^\dagger_{\mathrm{T},\tau}(\boldsymbol{r})$. Recall that

$$H_V = \begin{pmatrix} \Delta_b(r) & \Delta_{\mathrm{T},+K}(\boldsymbol{r}) & 0 & 0 \\ \Delta^\dagger_{\mathrm{T},+K}(\boldsymbol{r}) & \Delta_t(r) & 0 & 0 \\ 0 & 0 & \Delta_b(r) & \Delta_{\mathrm{T},-K}(\boldsymbol{r}) \\ 0 & 0 & \Delta^\dagger_{\mathrm{T},-K}(\boldsymbol{r}) & \Delta_t(r) \end{pmatrix}. \tag{11}$$

The expression for diagonal terms are: $\Delta_\alpha(r) = V_0 \sum_{i=1}^{3} \cos(\boldsymbol{G}_i \cdot \boldsymbol{r} + \phi_\alpha)$ The expression for off-diagonal terms are: $\Delta_{\mathrm{T},\tau}(\boldsymbol{r}) = T_0 \sum_{i=1}^{3} e^{i\boldsymbol{G}_i \cdot \boldsymbol{r}}$

**Answer**: The expressions for $\Delta_t(r)$, $\Delta_b(r)$, $\Delta_{\mathrm{T},\tau}(\boldsymbol{r})$ and $\Delta^\dagger_{\mathrm{T},\tau}(\boldsymbol{r})$ are as follows: - $\Delta_t(r) = V_0 \sum_{i=1}^{3} \cos(\boldsymbol{G}_i \cdot \boldsymbol{r} + \phi_t)$ - $\Delta_b(r) = V_0 \sum_{i=1}^{3} \cos(\boldsymbol{G}_i \cdot \boldsymbol{r} + \phi_b)$ - $\Delta_{\mathrm{T},+K}(\boldsymbol{r}) = T_0 \sum_{i=1}^{3} e^{i\boldsymbol{G}_i \cdot \boldsymbol{r}}$ - $\Delta_{\mathrm{T},-K}(\boldsymbol{r}) = T_0 \sum_{i=1}^{3} e^{-i\boldsymbol{G}_i \cdot \boldsymbol{r}}$

Substituting these into the potential Hamiltonian $H_V$, we get:

$$H_V = \begin{pmatrix} V_0 \sum_{i=1}^{3} \cos(\boldsymbol{G}_i \cdot \boldsymbol{r} + \phi_b) & T_0 \sum_{i=1}^{3} e^{i\boldsymbol{G}_i \cdot \boldsymbol{r}} & 0 & 0 \\ T_0 \sum_{i=1}^{3} e^{-i\boldsymbol{G}_i \cdot \boldsymbol{r}} & V_0 \sum_{i=1}^{3} \cos(\boldsymbol{G}_i \cdot \boldsymbol{r} + \phi_t) & 0 & 0 \\ 0 & 0 & V_0 \sum_{i=1}^{3} \cos(\boldsymbol{G}_i \cdot \boldsymbol{r} + \phi_b) & T_0 \sum_{i=1}^{3} e^{-i\boldsymbol{G}_i \cdot \boldsymbol{r}} \\ 0 & 0 & T_0 \sum_{i=1}^{3} e^{i\boldsymbol{G}_i \cdot \boldsymbol{r}} & V_0 \sum_{i=1}^{3} \cos(\boldsymbol{G}_i \cdot \boldsymbol{r} + \phi_t) \end{pmatrix} \tag{12}$$

Here, $\phi_t$ and $\phi_b$ are the phase shifts for the top and bottom layers respectively, and $\boldsymbol{G}_i$ are the reciprocal lattice vectors of the moiré pattern. The potential terms represent intralayer potentials and interlayer tunneling, consistent with the AB-stacked $MoTe_2/WSe_2$ system described.

# 6 Second-quantization (matrix)

## 6.1 Execution-Notation

### 6.1.1

**Prompt: Execution: Notation** Here I provide the notation you should use for this task. You should combine it with previous **Execution: Core information** to obtain the full instruction for execution. In the response, you will first repeat the instruction for execution and then proceed with the calculation. "' You will be instructed to construct the second quantized form of the total noninteracting Hamiltonian in the real space.The noninteracting Hamiltonian in the real space $H_0$ is the sum of Kinetic Hamiltonian $H_T$ and Potential Hamiltonian $H_V$.To construct the second quantized form of a Hamiltonian. You should construct the creation and annihilation operators from the basis explicitly. You should follow the EXAMPLE below to convert a Hamiltonian from the single-particle form to second-quantized form.Finally by "total", it means you need to take a summation over the real space position $r$.Return the second quantized form of the total noninteracting Hamiltonian $\hat{H}^0$

Use the following conventions for the symbols (You should also obey the conventions in all my previous prompts if you encounter undefined symbols. If you find it is never defined or has conflicts in the conventions, you should stop and let me know):Note that the spin index of the fermion operators $\Psi_\tau$ is both layer and valley dependent.

===EXAMPLE:For a Hamiltonian $H$, where $H = \begin{pmatrix} H_{a,a} & H_{a,b} \\ H_{b,a} & H_{b,b} \end{pmatrix}$ and the order of basis is (a), (b), we can construct the creation operators $\psi_a^\dagger$ and $\psi_b^\dagger$, and the annihilation operator $\psi_a$ and $\psi_b$.The corresponding second quantized form is $\hat{H} = \vec{\psi}^\dagger H \vec{\psi}$, where $\vec{\psi} = \begin{pmatrix} \psi_a \\ \psi_b \end{pmatrix}$ and $\vec{\psi}^\dagger = \begin{pmatrix} \psi_a^\dagger & \psi_b^\dagger \end{pmatrix}$. "'

### 6.1.2

**Completion: Instructions to execute**: You will be instructed to construct the second quantized form of the total noninteracting Hamiltonian in the real space. The noninteracting Hamiltonian in the real space $H_0$ is the sum of Kinetic Hamiltonian $H_T$ and Potential Hamiltonian $H_V$. To construct the second quantized form of a Hamiltonian, you should construct the creation and annihilation operators from the basis explicitly. Finally, by "total," it means you need to take a summation over the real space position $r$. Return the second quantized form of the total noninteracting Hamiltonian $\hat{H}^0$.

**Answer**: First, let's express the kinetic and potential Hamiltonians in the single-particle form: - Kinetic Hamiltonian $H_T$:

$$H_T = \begin{pmatrix} E_{+K,b} & 0 & 0 & 0 \\ 0 & E_{+K,t} & 0 & 0 \\ 0 & 0 & E_{-K,b} & 0 \\ 0 & 0 & 0 & E_{-K,t} \end{pmatrix} \tag{13}$$

- Potential Hamiltonian $H_V$:

$$H_V = \begin{pmatrix} \Delta_b(r) & \Delta_{\mathrm{T},+K}(\boldsymbol{r}) & 0 & 0 \\ \Delta_{\mathrm{T},+K}^\dagger(\boldsymbol{r}) & \Delta_t(r) & 0 & 0 \\ 0 & 0 & \Delta_b(r) & \Delta_{\mathrm{T},-K}(\boldsymbol{r}) \\ 0 & 0 & \Delta_{\mathrm{T},-K}^\dagger(\boldsymbol{r}) & \Delta_t(r) \end{pmatrix} \tag{14}$$

Now, to construct the second quantized form, let's define the creation ($\psi^\dagger$) and annihilation ($\psi$) operators for each of the basis states: (+K,bottom), (+K,top), (-K,bottom), and (-K,top). The basis order corresponds to the order of terms in the Hamiltonians.

The second quantized form of the total noninteracting Hamiltonian $\hat{H}^0$ is given by:

$$\hat{H}^0 = \int d\boldsymbol{r}\, \Psi^\dagger(\boldsymbol{r})\,(H_T + H_V)\,\Psi(\boldsymbol{r}) \tag{15}$$

where $\Psi(\boldsymbol{r})$ is the column vector of annihilation operators and $\Psi^\dagger(\boldsymbol{r})$ is the row vector of creation operators, defined as:

$$\Psi(\boldsymbol{r}) = \begin{pmatrix} \psi_{+K,b}(\boldsymbol{r}) \\ \psi_{+K,t}(\boldsymbol{r}) \\ \psi_{-K,b}(\boldsymbol{r}) \\ \psi_{-K,t}(\boldsymbol{r}) \end{pmatrix}, \quad \Psi^\dagger(\boldsymbol{r}) = \begin{pmatrix} \psi_{+K,b}^\dagger(\boldsymbol{r}) & \psi_{+K,t}^\dagger(\boldsymbol{r}) & \psi_{-K,b}^\dagger(\boldsymbol{r}) & \psi_{-K,t}^\dagger(\boldsymbol{r}) \end{pmatrix} \tag{16}$$

The creation and annihilation operators correspond to different layers and valleys as indicated by their subscripts. The spin index of these fermion operators is both layer and valley dependent as per the conventions provided. The integration over $\boldsymbol{r}$ takes the sum over all space, accounting for the real space position in the Hamiltonian.

# 7 Second-quantization (summation)

## 7.1 Execution-Notation

### 7.1.1

**Prompt: Execution: Notation** Here I provide the notation you should use for this task. You should combine it with previous **Execution: Core information** to obtain the full instruction for execution. In the response, you will first repeat the instruction for execution and then proceed with the calculation. "' You will be instructed to expand the second-quantized form Hamiltonian $\hat{H}^0$ using $H_\tau$ and $\Psi_\tau$. You should follow the EXAMPLE below to expand the Hamiltonian.You should use any previous knowledge to simplify it. For example, if any term of $H_\tau$ is zero, you should remove it from the summation. You should recall that $\hat{H}^0$ is

$$\hat{H}^0 = \int d\mathbf{r}\, \Psi^\dagger(\mathbf{r}) \begin{pmatrix} E_{+K,b}+V(\mathbf{r}) & T(\mathbf{r}) & 0 & 0 \\ T^\dagger(\mathbf{r}) & E_{+K,t}+V(\mathbf{r}) & 0 & 0 \\ 0 & 0 & E_{-K,b}+V(\mathbf{r}) & T(\mathbf{r}) \\ 0 & 0 & T^\dagger(\mathbf{r}) & E_{-K,t}+V(\mathbf{r}) \end{pmatrix} \Psi(\mathbf{r}) \tag{17}$$

.Return the expanded form of $\hat{H}^0$ after simplification.

Use the following conventions for the symbols (You should also obey the conventions in all my previous prompts if you encounter undefined symbols. If you find it is never defined or has conflicts in the conventions, you should stop and let me know):$\hat{\mathcal{H}}_0$ is the second-quantized form Hamiltonian, $H_\tau$ is the matrix element, and $\Psi_\tau$ is the basis. $\tau = \pm$ represents $\pm K$ valleys. The spin index of the fermion operators $\Psi_\tau$ is both layer and valley dependent.

===EXAMPLE:For a $\hat{H} = \vec{\psi}^\dagger H \vec{\psi}$, where $\vec{\psi} = \begin{pmatrix}\psi_a \\ \psi_b\end{pmatrix}$ and $\vec{\psi}^\dagger = \begin{pmatrix}\psi_a^\dagger & \psi_b^\dagger\end{pmatrix}$, we can expand it as $\hat{H} = \sum_{i,j=\{a,b\}} \psi_i^\dagger H_{i,j} \psi_j$. "'

### 7.1.2

**Completion: Instructions to execute**: You will be instructed to expand the second-quantized form Hamiltonian $\hat{H}^0$ using $H_\tau$ and $\Psi_\tau$. Recall that $\hat{H}^0$ is given by

$$\hat{H}^0 = \int d\mathbf{r}\, \Psi^\dagger(\mathbf{r}) \begin{pmatrix} E_{+K,b}+V(\mathbf{r}) & T(\mathbf{r}) & 0 & 0 \\ T^\dagger(\mathbf{r}) & E_{+K,t}+V(\mathbf{r}) & 0 & 0 \\ 0 & 0 & E_{-K,b}+V(\mathbf{r}) & T(\mathbf{r}) \\ 0 & 0 & T^\dagger(\mathbf{r}) & E_{-K,t}+V(\mathbf{r}) \end{pmatrix} \Psi(\mathbf{r})\,. \tag{18}$$

You should use any previous knowledge to simplify it, including removing any zero terms from the summation. The spin index of the fermion operators $\Psi_\tau$ is both layer and valley dependent.

**Answer**: Given the structure of $\hat{H}^0$, we can expand it as follows:

$$\hat{H}^0 \tag{19}$$

$$= \int d\mathbf{r}\, \Big[\Psi^\dagger_{+K,b}(\mathbf{r})\left(E_{+K,b}+V(\mathbf{r})\right)\Psi_{+K,b}(\mathbf{r}) + \Psi^\dagger_{+K,b}(\mathbf{r})T(\mathbf{r})\Psi_{+K,t}(\mathbf{r}) + \Psi^\dagger_{+K,t}(\mathbf{r})T^\dagger(\mathbf{r})\Psi_{+K,b}(\mathbf{r}) + \Psi^\dagger_{+K,t}(\mathbf{r})\left(E_{+K,t}+V(\mathbf{r})\right)\Psi_{+K,t}(\mathbf{r})$$

$$+\Psi^\dagger_{-K,b}(\mathbf{r})\left(E_{-K,b}+V(\mathbf{r})\right)\Psi_{-K,b}(\mathbf{r}) + \Psi^\dagger_{-K,b}(\mathbf{r})T(\mathbf{r})\Psi_{-K,t}(\mathbf{r}) + \Psi^\dagger_{-K,t}(\mathbf{r})T^\dagger(\mathbf{r})\Psi_{-K,b}(\mathbf{r}) + \Psi^\dagger_{-K,t}(\mathbf{r})\left(E_{-K,t}+V(\mathbf{r})\right)\Psi_{-K,t}(\mathbf{r})\Big] \tag{20}$$

In this expansion: - $\Psi^\dagger_{\tau,\alpha}(\mathbf{r})$ and $\Psi_{\tau,\alpha}(\mathbf{r})$ are the creation and annihilation operators for valley $\tau$ and layer $\alpha$ at position $\mathbf{r}$. - $E_{\tau,\alpha}$ represents the energy level for valley $\tau$ and layer $\alpha$. - $V(\mathbf{r})$ is the potential at position $\mathbf{r}$. - $T(\mathbf{r})$ and $T^\dagger(\mathbf{r})$ are the tunneling terms between the layers.

The integration over $\mathbf{r}$ sums these contributions over all space. The expansion includes all the necessary terms while adhering to the conventions and structure provided.

# 8 Fourier transform noninteracting term to momentum space (continuum)

## 8.1 Execution-Notation

### 8.1.1

**Prompt: Execution: Notation** Here I provide the notation you should use for this task. You should combine it with previous **Execution: Core information** to obtain the full instruction for execution. In the response, you will first repeat the instruction for execution and then proceed with the calculation. "' You will be instructed to convert the total noninteracting Hamiltonian in

the second quantized form from the basis in real space to the basis by momentum space.To do that, you should apply the Fourier transform to $\psi_{\tau,l}^\dagger(r)$ in the real space to the $c_{\tau,l}^\dagger(k)$ in the momentum space, which is defined as $c_{\tau,l}^\dagger(k) = \frac{1}{\sqrt{V}} \int dr \psi_{\tau,l}^\dagger(r) e^{ik\cdot r}$, where $\boldsymbol{r}$ is integrated over the entire real space. You should follow the EXAMPLE below to apply the Fourier transform.Express the total noninteracting Hamiltonian $\hat{H}^0$ in terms of $c_{\tau,l}^\dagger(k)$. Simplify any summation index if possible.

Use the following conventions for the symbols (You should also obey the conventions in all my previous prompts if you encounter undefined symbols. If you find it is never defined or has conflicts in the conventions, you should stop and let me know):$\tau = \pm$ represents $\pm K$ valleys, $\hbar \boldsymbol{k} = -i\hbar \partial_{\boldsymbol{r}}$ is the momentum operator, $\boldsymbol{\kappa} = \frac{4\pi}{3a_M}(1,0)$ is at a corner of the moir'e Brillouin zone, and $a_M$ is the moir'e lattice constant. The spin index of the fermion operators $\Psi_\tau$ is both layer and valley dependent. $h^{(\tau)}$ is the Hamiltonian $H_\tau$ expanded in the plane-wave basis, and the momentum $\boldsymbol{k}$ is defined in the extended Brillouin zone that spans the full momentum space, i.e., $\boldsymbol{k} \in \mathbb{R}^2$. The subscripts $\alpha, \beta$ are index for momenta. Due to Bloch's theorem, $h_{\boldsymbol{k}_\alpha l_\alpha, \boldsymbol{k}_\beta l_\beta}^{(\tau)}$ is nonzero only when $\boldsymbol{k}_\alpha - \boldsymbol{k}_\beta$ is equal to the linear combination of any multiples of one of the moir'e reciprocal lattice vectors (including the zero vector).

===EXAMPLE:Write a Hamiltonian $\hat{H}$ in the second quantized form, $\hat{H} = \int dr \psi(r)^\dagger H(r) \psi(r)$, where $r$ is integrated over the entire real space.Define the Fourier transform $c^\dagger(k) = \frac{1}{\sqrt{V}} \int \psi^\dagger(r) e^{ik\cdot r} dr$, where $r$ is integrated over the entire real space, and $V$ is the area of the unit cell in the real space.This leads to the inverse Fourier transform $\psi^\dagger(r) = \frac{1}{\sqrt{V}} \sum_k c^\dagger(k) e^{-ik\cdot r}$, where $k$ is summed over the extended Brillouin zone (i.e., the entire momentum space), $\Omega$ is the area of Brillouin zone in the momentum space.Thus, substitute $\psi^\dagger(r)$ and $\psi(r)$ into $\hat{H}$, we get

$$\begin{aligned}
\hat{H} &= \int dr \frac{1}{\sqrt{V}} \sum_{k_1} c^\dagger(k_1) e^{-ik_1\cdot r} H(r) \frac{1}{\sqrt{V}} \sum_{k_2} c(k_2) e^{ik_2\cdot r} \\
&= \sum_{k_1,k_2} c^\dagger(k_1) \frac{1}{V} \int dr e^{-i(k_1-k_2)\cdot r} H(r) c(k_2) \qquad (21) \\
&= \sum_{k_1,k_2} c^\dagger(k_1) H(k_1,k_2) c(k_2)
\end{aligned}$$

, where we define the Fourier transform of $H(r)$ as $H(k_1,k_2) = \frac{1}{V} \int dr e^{-i(k_1-k_2)\cdot r} H(r)$. "'

### 8.1.2

**Completion: Instructions to execute**: You will be instructed to convert the total noninteracting Hamiltonian in the second quantized form from the basis in real space to the basis in momentum space. Apply the Fourier transform to $\psi_{\tau,l}^\dagger(r)$ in the real space to $c_{\tau,l}^\dagger(k)$ in the momentum space. Express the total noninteracting Hamiltonian $\hat{H}^0$ in terms of $c_{\tau,l}^\dagger(k)$ and simplify any summation index if possible. Recall the conventions regarding the representation of valleys, momentum, reciprocal lattice vectors, and the relation of Hamiltonian matrix elements in the plane-wave basis.

**Answer**: First, let's define the Fourier transform for the creation and annihilation operators:

$$c_{\tau,l}^\dagger(k) = \frac{1}{\sqrt{V}} \int dr\, \psi_{\tau,l}^\dagger(r) e^{ik\cdot r} \qquad (22)$$

$$c_{\tau,l}(k) = \frac{1}{\sqrt{V}} \int dr\, \psi_{\tau,l}(r) e^{-ik\cdot r} \qquad (23)$$

where $V$ is the volume of the system.

The inverse Fourier transform is then:

$$\psi_{\tau,l}^\dagger(r) = \frac{1}{\sqrt{V}} \sum_k c_{\tau,l}^\dagger(k) e^{-ik\cdot r} \qquad (24)$$

$$\psi_{\tau,l}(r) = \frac{1}{\sqrt{V}} \sum_k c_{\tau,l}(k) e^{ik\cdot r} \qquad (25)$$

Substituting these into $\hat{H}^0$, we get:

$$\hat{H}^0 = \int dr \frac{1}{\sqrt{V}} \sum_{k_1} c_{\tau,l}^\dagger(k_1) e^{-ik_1\cdot r} H(r) \frac{1}{\sqrt{V}} \sum_{k_2} c_{\tau,l}(k_2) e^{ik_2\cdot r} \qquad (26)$$

$$= \sum_{k_1,k_2} c_{\tau,l}^\dagger(k_1) \frac{1}{V} \int dr\, e^{-i(k_1-k_2)\cdot r} H(r) c_{\tau,l}(k_2) \qquad (27)$$

$$= \sum_{k_1,k_2} c^{\dagger}_{\tau,l}(k_1) H_{\tau}(k_1,k_2) c_{\tau,l}(k_2) \tag{28}$$

where $H_\tau(k_1, k_2)$ is the Fourier transform of the Hamiltonian $H(r)$ and is defined as:

$$H_\tau(k_1,k_2) = \frac{1}{V}\int dr\, e^{-i(k_1-k_2)\cdot r} H(r) \tag{29}$$

This represents the total noninteracting Hamiltonian $\hat{H}^0$ in the momentum space, with $k_1$ and $k_2$ being the momentum indices summed over the extended Brillouin zone. The Hamiltonian matrix elements are nonzero only when $\boldsymbol{k}_\alpha - \boldsymbol{k}_\beta$ equals a linear combination of moiré reciprocal lattice vectors (including the zero vector), according to Bloch's theorem.

# 9 Particle-hole transformation

## 9.1 Execution-Notation

### 9.1.1

**Prompt: Execution: Notation** Here I provide the notation you should use for this task. You should combine it with previous **Execution: Core information** to obtain the full instruction for execution. In the response, you will first repeat the instruction for execution and then proceed with the calculation. "' You will be instructed to perform a particle-hole transformation.Define a hole operator, $b_{\boldsymbol{k},l,\tau}$, which equals $c^\dagger_{\boldsymbol{k},l,\tau}$.You should replace $c^\dagger_{\boldsymbol{k},l,\tau}$ with $b_{\boldsymbol{k},l,\tau}$, and $c_{\boldsymbol{k},l,\tau}$ with $b^\dagger_{\boldsymbol{k},l,\tau}$. You should follow the EXAMPLE below to apply the particle-hole transformation.You should recall that $\hat{H}^0 = \sum_{\tau,k_\alpha,k_\beta} c^\dagger_{\tau,l}(k_\alpha) h^{(\tau)}_{\boldsymbol{k}_\alpha l_\alpha,\boldsymbol{k}_\beta l_\beta} c_{\tau,l}(k_\beta)$. Return the $\hat{H}^0$ in the hole operators.

Use the following conventions for the symbols (You should also obey the conventions in all my previous prompts if you encounter undefined symbols. If you find it is never defined or has conflicts in the conventions, you should stop and let me know):The hole operator is defined as $b_{\boldsymbol{k},l,\tau} = c^\dagger_{\boldsymbol{k},l,\tau}$. The Hamiltonian in the hole basis is represented as $\hat{\mathcal{H}}_0$.

===EXAMPLE:Give a Hamiltonian $\hat{H} = \sum_{k_1,k_2} c^\dagger(k_1) h(k_1,k_2) c(k_2)$ , and the particle-hole transformation as $b(k) = c^\dagger(k)$. The transformed Hamiltonian is $\hat{H} = \sum_{k_1,k_2} b(k_1) h(k_1,k_2) b^\dagger(k_2)$ "'

### 9.1.2

**Completion: Instructions to execute**: You will be instructed to perform a particle-hole transformation. Define a hole operator, $b_{\boldsymbol{k},l,\tau}$, which equals $c^\dagger_{\boldsymbol{k},l,\tau}$. Replace $c^\dagger_{\boldsymbol{k},l,\tau}$ with $b_{\boldsymbol{k},l,\tau}$, and $c_{\boldsymbol{k},l,\tau}$ with $b^\dagger_{\boldsymbol{k},l,\tau}$. Recall that $\hat{H}^0 = \sum_{\tau,k_\alpha,k_\beta} c^\dagger_{\tau,l}(k_\alpha) h^{(\tau)}_{\boldsymbol{k}_\alpha l_\alpha,\boldsymbol{k}_\beta l_\beta} c_{\tau,l}(k_\beta)$. Return the $\hat{H}^0$ in the hole operators.

**Answer**: Given the definition of the hole operator $b_{\boldsymbol{k},l,\tau} = c^\dagger_{\boldsymbol{k},l,\tau}$ and the particle-hole transformation, the transformed Hamiltonian can be written as:

$$\hat{H}^0_{\text{hole}} = \sum_{\tau,k_\alpha,k_\beta} b_{\boldsymbol{k}_\alpha l_\alpha,\tau}(k_\alpha) h^{(\tau)}_{\boldsymbol{k}_\alpha l_\alpha,\boldsymbol{k}_\beta l_\beta} b^\dagger_{\boldsymbol{k}_\beta l_\beta,\tau}(k_\beta) \tag{30}$$

This expression represents the total noninteracting Hamiltonian $\hat{H}^0$ in terms of the hole operators $b_{\boldsymbol{k},l,\tau}$ and $b^\dagger_{\boldsymbol{k},l,\tau}$. The Hamiltonian matrix elements $h^{(\tau)}_{\boldsymbol{k}_\alpha l_\alpha,\boldsymbol{k}_\beta l_\beta}$ remain unchanged, as they depend on the system's physical properties, which are independent of the chosen particle or hole representation. The transformation effectively switches the roles of filled and empty states in the system, which is a common technique in studying systems where the particle-like excitations are holes rather than electrons.

# 10 Simplify the Hamiltonian in the particle-hole basis

## 10.1 Execution-Notation

### 10.1.1

**Prompt: Execution: Notation** Here I provide the notation you should use for this task. You should combine it with previous **Execution: Core information** to obtain the full instruction for execution. In the response, you will first repeat the instruction for execution and then proceed with the calculation. "' You will be instructed to simplify the $\hat{H}^0$ in the hole basis.You should use canonical commutator relation for fermions to reorder the hole operator to the normal order. Normal order means that creation operators always appear before the annihilation operators. You should follow the EXAMPLE below to simplify it to the normal order.Express the $\hat{H}^0$ in the normal order of $b_{\boldsymbol{k},l,\tau}$ and also make $\boldsymbol{k}_\alpha$ always appear before $\boldsymbol{k}_\beta$ in the index of $b_{\boldsymbol{k},l,\tau}$

and $[h^{(\tau)}]^{\intercal}_{\boldsymbol{k}_\alpha l_\alpha,\boldsymbol{k}_\beta l_\beta}$.You should recall that $\hat{H}^0 = \sum_{\tau,k_\alpha,k_\beta} b_{\boldsymbol{k}_\alpha,l_\alpha,\tau} h^{(\tau)}_{\boldsymbol{k}_\alpha l_\alpha,\boldsymbol{k}_\beta l_\beta} b^\dagger_{\boldsymbol{k}_\beta,l_\beta,\tau}$ Use the following conventions for the symbols (You should also obey the conventions in all my previous prompts if you encounter undefined symbols. If you find it is never defined or has conflicts in the conventions, you should stop and let me know):$b_{\boldsymbol{k},l,\tau} = c^\dagger_{\boldsymbol{k},l,\tau}$

=== EXAMPLE:For $\hat{H}^0 = \sum_{i,j} b_i H_{i,j} b_j^\dagger$, where $b_i$ satisfies fermion statistics (anticommuting to its self-adjoint operator).This gives '$[b_i, b_j^\dagger]_+ = \delta_{i,j}$', which means $b_i b_j^\dagger = \delta_{i,j} - b_j^\dagger b_i$.Substitute it into $\hat{H}^0$, we have $\hat{H}^0 = \sum_{i,j}(\delta_{i,j} - b_j^\dagger b_i) H_{i,j} = \sum_{i,j}\delta_{i,j} H_{i,j} - \sum_{i,j} b_j^\dagger b_i H_{i,j} = \sum_i H_{i,i} - \sum_{i,j} b_j^\dagger b_i H_{i,j}$.The first term is simply $\sum_i H_{i,i}$ by summing over the index $j$ due to $\delta_{i,j}$. The second term is $-\sum_{i,j} b_j^\dagger b_i H_{i,j}$.Relabeling the index of $i$ and $j$ by swapping them to make it consistent with the original order of index (namely, $i$ appears before $j$ in the index of $b$ and $H$), it becomes $-\sum_{i,j} b_i^\dagger H_{j,i} b_j$. Finally, to fix the order of the index in $H$ such that $i$ appears before $j$, we notice that '$H_{j,i} = (H_{i,j})^*$', where '*' means complex conjugate, because the Hamiltonian is Hermitian.Thus, we end up in $\hat{H}^0 = \sum_{i,j} b_i H_{i,j} b_j^\dagger = \sum_i H_{i,i} - \sum_{i,j} b_i^\dagger (H_{i,j})^* b_j$ "'

#### 10.1.2

**Completion: Instructions to execute**: You will be instructed to simplify the $\hat{H}^0$ in the hole basis to normal order, where creation operators always appear before annihilation operators. Use the canonical commutator relation for fermions to reorder the hole operator. Express the $\hat{H}^0$ in the normal order of $b_{\boldsymbol{k},l,\tau}$ and ensure $\boldsymbol{k}_\alpha$ always appears before $\boldsymbol{k}_\beta$ in the index. Recall that $\hat{H}^0 = \sum_{\tau,k_\alpha,k_\beta} b_{\boldsymbol{k}_\alpha,l_\alpha,\tau} h^{(\tau)}_{\boldsymbol{k}_\alpha l_\alpha,\boldsymbol{k}_\beta l_\beta} b^\dagger_{\boldsymbol{k}_\beta,l_\beta,\tau}$.

**Answer**: Starting from the given Hamiltonian in the hole basis:

$$\hat{H}^0 = \sum_{\tau,k_\alpha,k_\beta} b_{\boldsymbol{k}_\alpha,l_\alpha,\tau} h^{(\tau)}_{\boldsymbol{k}_\alpha l_\alpha,\boldsymbol{k}_\beta l_\beta} b^\dagger_{\boldsymbol{k}_\beta,l_\beta,\tau} \tag{31}$$

We apply the fermionic anticommutation relations:

$$[b_{\boldsymbol{k}_\alpha,l_\alpha,\tau}, b^\dagger_{\boldsymbol{k}_\beta,l_\beta,\tau}]_+ = \delta_{\boldsymbol{k}_\alpha,\boldsymbol{k}_\beta}\delta_{l_\alpha,l_\beta}\delta_{\tau,\tau} \tag{32}$$

which implies:

$$b_{\boldsymbol{k}_\alpha,l_\alpha,\tau} b^\dagger_{\boldsymbol{k}_\beta,l_\beta,\tau} = \delta_{\boldsymbol{k}_\alpha,\boldsymbol{k}_\beta}\delta_{l_\alpha,l_\beta}\delta_{\tau,\tau} - b^\dagger_{\boldsymbol{k}_\beta,l_\beta,\tau} b_{\boldsymbol{k}_\alpha,l_\alpha,\tau} \tag{33}$$

Substituting this into $\hat{H}^0$:

$$\hat{H}^0 = \sum_{\tau,k_\alpha,k_\beta} (\delta_{\boldsymbol{k}_\alpha,\boldsymbol{k}_\beta}\delta_{l_\alpha,l_\beta}\delta_{\tau,\tau} - b^\dagger_{\boldsymbol{k}_\beta,l_\beta,\tau} b_{\boldsymbol{k}_\alpha,l_\alpha,\tau}) h^{(\tau)}_{\boldsymbol{k}_\alpha l_\alpha,\boldsymbol{k}_\beta l_\beta} \tag{34}$$

Simplifying and reordering the indices:

$$\hat{H}^0 = \sum_{\tau,k_\alpha,k_\beta} \delta_{\boldsymbol{k}_\alpha,\boldsymbol{k}_\beta}\delta_{l_\alpha,l_\beta}\delta_{\tau,\tau} h^{(\tau)}_{\boldsymbol{k}_\alpha l_\alpha,\boldsymbol{k}_\beta l_\beta} - \sum_{\tau,k_\alpha,k_\beta} b^\dagger_{\boldsymbol{k}_\beta,l_\beta,\tau} h^{(\tau)}_{\boldsymbol{k}_\alpha l_\alpha,\boldsymbol{k}_\beta l_\beta} b_{\boldsymbol{k}_\alpha,l_\alpha,\tau} \tag{35}$$

Using the fact that $h^{(\tau)}_{\boldsymbol{k}_\alpha l_\alpha,\boldsymbol{k}_\beta l_\beta}$ is Hermitian, and relabeling the indices:

$$\hat{H}^0 = \sum_{\tau,k} h^{(\tau)}_{\boldsymbol{k}l,\boldsymbol{k}l} - \sum_{\tau,k_\alpha,k_\beta} b^\dagger_{\boldsymbol{k}_\alpha,l_\alpha,\tau} [h^{(\tau)}_{\boldsymbol{k}_\beta l_\beta,\boldsymbol{k}_\alpha l_\alpha}]^* b_{\boldsymbol{k}_\beta,l_\beta,\tau} \tag{36}$$

This is the Hamiltonian $\hat{H}^0$ in the normal order of $b_{\boldsymbol{k},l,\tau}$ operators, with $\boldsymbol{k}_\alpha$ always appearing before $\boldsymbol{k}_\beta$ in the indices, and the Hamiltonian matrix elements $h^{(\tau)}_{\boldsymbol{k}_\alpha l_\alpha,\boldsymbol{k}_\beta l_\beta}$ transposed and conjugated accordingly.

# 11 Identify interacting term (momentum space)

## 11.1 Extraction

#### 11.1.1

**Prompt: Extraction Abstract** We present a theory on the quantum phase diagram of AB-stacked $MoTe_2/WSe_2$ using a self-consistent Hartree-Fock calculation performed in the plane-wave basis, motivated by the observation of topological states in this system. At filling factor $\nu = 2$ (two holes per moir'e unit cell), Coulomb interaction can stabilize a $\mathbb{Z}_2$ topological insulator by opening a charge gap. At $\nu = 1$, the interaction induces three classes of competing states, spin density wave states, an in-plane ferromagnetic state, and a valley polarized state, which undergo first-order phase transitions tuned by an out-of-plane displacement field. The valley polarized state becomes a Chern insulator for certain displacement fields. Moreover, we predict a

topological charge density wave forming a honeycomb lattice with ferromagnetism at $\nu = 2/3$. Future directions on this versatile system hosting a rich set of quantum phases are discussed.

**Question**: 1. What type of interaction should be used in the system? Remember the actual experimental device is usually dual-gated. 2. What is the mathematical formula for this interaction used in the Hamiltonian? You write it in the momentum space. Remember the interaction is a dual-gated screened Coulomb interaction (i.e., like a two-slab capacitor).

#### 11.1.2

**Completion:** 1. **What type of interaction should be used in the system? Quote**: "Coulomb interaction can stabilize a $\mathbb{Z}_2$ topological insulator" and "interaction induces three classes of competing states" **Explanation**: The abstract explicitly mentions the role of Coulomb interaction in stabilizing various quantum states in the AB-stacked $MoTe_2/WSe_2$ system. Given that the actual experimental device is usually dual-gated, which typically influences the screening of interactions, the type of interaction to be used in the system is a screened Coulomb interaction. This type of interaction accounts for the screening effect due to the presence of gates, which can modify the strength and range of the Coulomb interaction between charged particles. **Answer**: The type of interaction to be used in the system should be a dual-gated screened Coulomb interaction.

2. **What is the mathematical formula for this interaction used in the Hamiltonian in the momentum space?** **Explanation**: The screened Coulomb interaction in a dual-gated system, such as a two-slab capacitor, is typically described by a formula that accounts for the screening effect of the gates. In momentum space, the screened Coulomb interaction can be represented as a function of the wave vector, which modifies the standard Coulomb potential due to the presence of the gates. **Answer**: The mathematical formula for the dual-gated screened Coulomb interaction in momentum space can be written as:

$$V(\boldsymbol{k}) = \frac{e^2}{2\epsilon_0\epsilon_r|\boldsymbol{k}|}\frac{\tanh(|\boldsymbol{k}|d)}{|\boldsymbol{k}|d} \tag{37}$$

Here, $V(\boldsymbol{k})$ is the potential in momentum space, $\boldsymbol{k}$ is the wave vector, $e$ is the elementary charge, $\epsilon_0$ is the vacuum permittivity, $\epsilon_r$ is the relative permittivity of the material, and $d$ is the distance between the gates. The term $\tanh(|\boldsymbol{k}|d)/(|\boldsymbol{k}|d)$ represents the screening effect due to the dual-gate structure.

## 11.2 Execution-Core Information

#### 11.2.1

**Prompt: Execution–Core information** You should fill in the specific information from above into the following template, and then repeat it. "' To obtain the interaction form. You should use type of interaction with mathematical expression of interaction, where $q$ is the transferred total momentum between a creation operator and an annihilation operator with the same the valley index and layer index, namely $q = k_1 - k_4$.

#### 11.2.2

**Completion:** To obtain the interaction form, you should use dual-gated screened Coulomb interaction with the mathematical expression $V(\boldsymbol{q}) = \frac{e^2}{2\epsilon_0\epsilon_r|\boldsymbol{q}|}\frac{\tanh(|\boldsymbol{q}|d)}{|\boldsymbol{q}|d}$, where $\boldsymbol{q}$ is the transferred total momentum between a creation operator and an annihilation operator with the same valley index and layer index, namely $\boldsymbol{q} = \boldsymbol{k}_1 - \boldsymbol{k}_4$.

## 11.3 Execution-Notation

#### 11.3.1

**Prompt: Execution: Notation** Here I provide the notation you should use for this task. You should combine it with previous **Execution: Core information** to obtain the full instruction for execution. In the response, you will first repeat the instruction for execution and then proceed with the calculation. "' You will be instructed to construct the interaction part of the Hamiltonian $\hat{H}_{\text{int}}$ in the momentum space.

The interaction Hamiltonian is a product of the aforementioned interaction form and the following three parts. The first part is the product of four operators with two creation and two annihilation operators following the normal order, namely, creation operators are before annihilation operators. You should follow the order of $1, 2, 2, 1$ for the valley index and layer index, and $1, 2, 3, 4$ for the momentum. The second part is the constraint of total momentum conservation, namely the total momentum of all creation operators should be the same as that of all annihilation operators.The last is the normalization factor, you should use $\frac{1}{2A}$ here. Finally, the summation should be running over all the valley index and layer index, and momentum Return the interaction term $\hat{H}_{\text{int}}$ in terms of $b^\dagger_{\boldsymbol{k}_\alpha,l_\alpha,\tau_\alpha}$, $b^\dagger_{\boldsymbol{k}_\beta,l_\beta,\tau_\beta}$, $b_{\boldsymbol{k}_\gamma,l_\beta,\tau_\beta}$, $b_{\boldsymbol{k}_\delta,l_\alpha,\tau_\alpha}$ and $V(q)$ (with $q$ expressed in terms of momentum).

Use the following conventions for the symbols (You should also obey the conventions in all my previous prompts if you encounter undefined symbols. If you find it is never defined or has conflicts in the conventions, you should stop and let me

know):$\boldsymbol{k}_\alpha, \boldsymbol{k}_\beta, \boldsymbol{k}_\gamma, \boldsymbol{k}_\delta$ are the momenta, $l_\alpha, l_\beta$ are the indices of operators, $\tau_\alpha, \tau_\beta$ are the spin indices, $V(\boldsymbol{k})$ is the dual-gate screened Coulomb interaction, $d$ is the sample-to-gate distance, and $\epsilon$ is the dielectric constant. $\delta(..)$ is the Dirac delta function for momentum conservation. "'

#### 11.3.2

**Completion: Instructions to execute**: You will be instructed to construct the interaction part of the Hamiltonian $\hat{H}_{\text{int}}$ in the momentum space. The interaction Hamiltonian involves the dual-gated screened Coulomb interaction, a product of four fermionic operators in normal order (creation operators before annihilation operators), momentum conservation, and a normalization factor. The momentum conservation ensures the total momentum of all creation operators equals that of all annihilation operators. The normalization factor is $\frac{1}{2A}$. Sum over all valley indices, layer indices, and momenta. Return the interaction term $\hat{H}_{\text{int}}$ using $b^\dagger_{\boldsymbol{k}_\alpha,l_\alpha,\tau_\alpha}$, $b^\dagger_{\boldsymbol{k}_\beta,l_\beta,\tau_\beta}$, $b_{\boldsymbol{k}_\gamma,l_\beta,\tau_\beta}$, $b_{\boldsymbol{k}_\delta,l_\alpha,\tau_\alpha}$ and $V(q)$, with $q$ expressed in terms of momentum.

**Answer**: The interaction Hamiltonian $\hat{H}_{\text{int}}$ in momentum space is given by:

$$\hat{H}_{\text{int}} = \frac{1}{2A} \sum_{\substack{\boldsymbol{k}_\alpha,\boldsymbol{k}_\beta,\boldsymbol{k}_\gamma,\boldsymbol{k}_\delta \\ l_\alpha,l_\beta \\ \tau_\alpha,\tau_\beta}} V(\boldsymbol{q})\delta(\boldsymbol{k}_\alpha + \boldsymbol{k}_\beta - \boldsymbol{k}_\gamma - \boldsymbol{k}_\delta) b^\dagger_{\boldsymbol{k}_\alpha,l_\alpha,\tau_\alpha} b^\dagger_{\boldsymbol{k}_\beta,l_\beta,\tau_\beta} b_{\boldsymbol{k}_\gamma,l_\beta,\tau_\beta} b_{\boldsymbol{k}_\delta,l_\alpha,\tau_\alpha} \tag{38}$$

where

$$V(\boldsymbol{q}) = \frac{e^2}{2\epsilon_0\epsilon_r|\boldsymbol{q}|}\frac{\tanh(|\boldsymbol{q}|d)}{|\boldsymbol{q}|d} \tag{39}$$

and

$$\boldsymbol{q} = \boldsymbol{k}_\alpha - \boldsymbol{k}_\delta \tag{40}$$

In this Hamiltonian: - $b^\dagger_{\boldsymbol{k}_\alpha,l_\alpha,\tau_\alpha}$ and $b^\dagger_{\boldsymbol{k}_\beta,l_\beta,\tau_\beta}$ are creation operators. - $b_{\boldsymbol{k}_\gamma,l_\beta,\tau_\beta}$ and $b_{\boldsymbol{k}_\delta,l_\alpha,\tau_\alpha}$ are annihilation operators. - $V(\boldsymbol{q})$ is the dual-gated screened Coulomb interaction potential. - The delta function $\delta(\boldsymbol{k}_\alpha + \boldsymbol{k}_\beta - \boldsymbol{k}_\gamma - \boldsymbol{k}_\delta)$ enforces momentum conservation. - The normalization factor is $\frac{1}{2A}$, where $A$ is the area of the system.

This Hamiltonian describes the interaction between particles (holes in this case) in the AB-stacked $MoTe_2/WSe_2$ system, taking into account the screening effect due to the dual-gated setup and momentum conservation.

# 12 Wick's theorem expansion

## 12.1 Execution-Notation

#### 12.1.1

**Prompt: Execution: Notation** Here I provide the notation you should use for this task. You should combine it with previous **Execution: Core information** to obtain the full instruction for execution. In the response, you will first repeat the instruction for execution and then proceed with the calculation. "' You will be instructed to perform a Hartree-Fock approximation to expand the interaction term, $\hat{H}_{\text{int}}$.You should use Wick's theorem to expand the four-fermion term in $\hat{H}_{\text{int}}$ into quadratic terms. You should strictly follow the EXAMPLE below to expand using Wick's theorem, select the correct EXAMPLE by noticing the order of four-term product with and without $^\dagger$, and be extremely cautious about the order of the index and sign before each term.You should only preserve the normal terms. Here, the normal terms mean the product of a creation operator and an annihilation operator.You should recall that $\hat{H}_{\text{int}}$ is $\hat{H}_{\text{int}} = \frac{1}{2A}\sum_{\substack{\tau_\alpha,\tau_\beta \\ l_\alpha,l_\beta}} \sum_{\boldsymbol{k}_\alpha,\boldsymbol{k}_\beta,\boldsymbol{k}_\gamma,\boldsymbol{k}_\delta} b^\dagger_{\boldsymbol{k}_\alpha,l_\alpha,\tau_\alpha} b^\dagger_{\boldsymbol{k}_\beta,l_\beta,\tau_\beta} b_{\boldsymbol{k}_\gamma,l_\beta,\tau_\beta} b_{\boldsymbol{k}_\delta,l_\alpha,\tau_\alpha} V(\boldsymbol{k}_\alpha - \boldsymbol{k}_\delta)\delta_{\boldsymbol{k}_\alpha+\boldsymbol{k}_\beta,\boldsymbol{k}_\gamma+\boldsymbol{k}_\delta}$.Return the expanded interaction term after Hartree-Fock approximation as $\hat{H}^{\text{HF}}$.

Use the following conventions for the symbols (You should also obey the conventions in all my previous prompts if you encounter undefined symbols. If you find it is never defined or has conflicts in the conventions, you should stop and let me know):$\hat{H}^{\text{HF}}$ is the Hartree-Fock Hamiltonian, $\hat{H}^{\text{HF}}_{\text{int}}$ is the interaction term in the Hartree-Fock Hamiltonian, $\boldsymbol{k}_\alpha, \boldsymbol{k}_\beta, \boldsymbol{k}_\gamma, \boldsymbol{k}_\delta$ are the momentum vectors, $l_\alpha, l_\beta$ are the orbital quantum numbers, $\tau_\alpha, \tau_\beta$ are the spin quantum numbers, $V(\boldsymbol{k}_\alpha - \boldsymbol{k}_\delta)$ is the interaction potential, $b^\dagger_{\boldsymbol{k}_\alpha,l_\alpha,\tau_\alpha}$ and $b_{\boldsymbol{k}_\delta,l_\alpha,\tau_\alpha}$ are the creation and annihilation operators, and $\langle ... \rangle$ denotes the expectation value.

===EXAMPLE 1:For a four-fermion term $a_1^\dagger a_2^\dagger a_3 a_4$, using Wick's theorem and preserving only the normal terms. this is expanded as $a_1^\dagger a_2^\dagger a_3 a_4 = \langle a_1^\dagger a_4\rangle a_2^\dagger a_3 + \langle a_2^\dagger a_3\rangle a_1^\dagger a_4 - \langle a_1^\dagger a_4\rangle\langle a_2^\dagger a_3\rangle - \langle a_1^\dagger a_3\rangle a_2^\dagger a_4 - \langle a_2^\dagger a_4\rangle a_1^\dagger a_3 + \langle a_1^\dagger a_3\rangle\langle a_2^\dagger a_4\rangle$Be cautious about the order of the index and sign before each term here.

EXAMPLE 2:For a four-fermion term $a_1^\dagger a_2 a_3^\dagger a_4$, using Wick's theorem and preserving only the normal terms. this is expanded as $a_1^\dagger a_2 a_3^\dagger a_4 = \langle a_1^\dagger a_2\rangle a_3^\dagger a_4 + \langle a_3^\dagger a_4\rangle a_1^\dagger a_2 - \langle a_1^\dagger a_2\rangle\langle a_3^\dagger a_4\rangle - \langle a_1^\dagger a_4\rangle a_3^\dagger a_2 - \langle a_3^\dagger a_2\rangle a_1^\dagger a_4 + \langle a_1^\dagger a_4\rangle\langle a_3^\dagger a_2\rangle$Be cautious about the order of the index and sign before each term here. "'

#### 12.1.2

**Completion: Instructions to execute**: You will be instructed to perform a Hartree-Fock approximation to expand the interaction term, $\hat{H}_{\text{int}}$, using Wick's theorem. The expansion should be carried out for the four-fermion term in $\hat{H}_{\text{int}}$ into quadratic terms, preserving only the normal terms (product of a creation operator and an annihilation operator). The interaction term $\hat{H}_{\text{int}}$ is given as $\hat{H}_{\text{int}} = \frac{1}{2A}\sum_{\substack{\tau_\alpha,\tau_\beta \\ l_\alpha,l_\beta}}\sum_{\boldsymbol{k}_\alpha,\boldsymbol{k}_\beta,\boldsymbol{k}_\gamma,\boldsymbol{k}_\delta} b^\dagger_{\boldsymbol{k}_\alpha,l_\alpha,\tau_\alpha} b^\dagger_{\boldsymbol{k}_\beta,l_\beta,\tau_\beta} b_{\boldsymbol{k}_\gamma,l_\beta,\tau_\beta} b_{\boldsymbol{k}_\delta,l_\alpha,\tau_\alpha} V(\boldsymbol{k}_\alpha - \boldsymbol{k}_\delta)\delta_{\boldsymbol{k}_\alpha+\boldsymbol{k}_\beta,\boldsymbol{k}_\gamma+\boldsymbol{k}_\delta}$. Return the expanded interaction term after the Hartree-Fock approximation as $\hat{H}^{\text{HF}}$.

**Answer**: Using Wick's theorem and preserving only the normal terms, the interaction term $\hat{H}_{\text{int}}$ can be expanded. The order of the product is $1^\dagger, 2^\dagger, 3, 4$, so following Example 1:

$$\hat{H}_{\text{int}} = \frac{1}{2A}\sum_{\substack{\tau_\alpha,\tau_\beta \\ l_\alpha,l_\beta}}\sum_{\boldsymbol{k}_\alpha,\boldsymbol{k}_\beta,\boldsymbol{k}_\gamma,\boldsymbol{k}_\delta} \Big(\langle b^\dagger_{\boldsymbol{k}_\alpha,l_\alpha,\tau_\alpha} b_{\boldsymbol{k}_\delta,l_\alpha,\tau_\alpha}\rangle b^\dagger_{\boldsymbol{k}_\beta,l_\beta,\tau_\beta} b_{\boldsymbol{k}_\gamma,l_\beta,\tau_\beta} \tag{41}$$

$$+\langle b^\dagger_{\boldsymbol{k}_\beta,l_\beta,\tau_\beta} b_{\boldsymbol{k}_\gamma,l_\beta,\tau_\beta}\rangle b^\dagger_{\boldsymbol{k}_\alpha,l_\alpha,\tau_\alpha} b_{\boldsymbol{k}_\delta,l_\alpha,\tau_\alpha} \tag{42}$$

$$-\langle b^\dagger_{\boldsymbol{k}_\alpha,l_\alpha,\tau_\alpha} b_{\boldsymbol{k}_\delta,l_\alpha,\tau_\alpha}\rangle \langle b^\dagger_{\boldsymbol{k}_\beta,l_\beta,\tau_\beta} b_{\boldsymbol{k}_\gamma,l_\beta,\tau_\beta}\rangle \tag{43}$$

$$-\langle b^\dagger_{\boldsymbol{k}_\alpha,l_\alpha,\tau_\alpha} b_{\boldsymbol{k}_\gamma,l_\beta,\tau_\beta}\rangle b^\dagger_{\boldsymbol{k}_\beta,l_\beta,\tau_\beta} b_{\boldsymbol{k}_\delta,l_\alpha,\tau_\alpha} - \langle b^\dagger_{\boldsymbol{k}_\beta,l_\beta,\tau_\beta} b_{\boldsymbol{k}_\delta,l_\alpha,\tau_\alpha}\rangle b^\dagger_{\boldsymbol{k}_\alpha,l_\alpha,\tau_\alpha} b_{\boldsymbol{k}_\gamma,l_\beta,\tau_\beta}\Big) \tag{44}$$

$$+\langle b^\dagger_{\boldsymbol{k}_\alpha,l_\alpha,\tau_\alpha} b_{\boldsymbol{k}_\gamma,l_\beta,\tau_\beta}\rangle \langle b^\dagger_{\boldsymbol{k}_\beta,l_\beta,\tau_\beta} b_{\boldsymbol{k}_\delta,l_\alpha,\tau_\alpha}\rangle V(\boldsymbol{k}_\alpha - \boldsymbol{k}_\delta)\delta_{\boldsymbol{k}_\alpha+\boldsymbol{k}_\beta,\boldsymbol{k}_\gamma+\boldsymbol{k}_\delta} \tag{45}$$

This expansion of $\hat{H}_{\text{int}}$ yields $\hat{H}^{\text{HF}}$, the Hartree-Fock Hamiltonian, where each term is the product of a creation operator and an annihilation operator (normal terms), and expectation values represent average occupations in the system. The terms involve sums over all possible combinations of momenta, layers, and spins, and include the interaction potential $V(\boldsymbol{k}_\alpha - \boldsymbol{k}_\delta)$, ensuring momentum conservation.

# 13 Drop constant terms

## 13.1 Execution-Notation

#### 13.1.1

**Prompt: Execution: Notation** Here I provide the notation you should use for this task. You should combine it with previous **Execution: Core information** to obtain the full instruction for execution. In the response, you will first repeat the instruction for execution and then proceed with the calculation. "' You will be instructed to extract the quadratic terms in the $\hat{H}^{\text{HF}}$.The quadratic terms mean terms that are proportional to $b^\dagger_{\boldsymbol{k}_\beta,l_\beta,\tau_\beta} b_{\boldsymbol{k}_\gamma,l_\beta,\tau_\beta}$ and $b^\dagger_{\boldsymbol{k}_\beta,l_\beta,\tau_\beta} b_{\boldsymbol{k}_\delta,l_\alpha,\tau_\alpha}$, which excludes terms that are solely expectations or products of expectations.You should only preserve the quadratic terms in $\hat{H}^{\text{HF}}$, denoted as $\hat{H}^{\text{HF}}_{\text{int}}$.You should recall that $\hat{H}^{\text{HF}}$ is

$$\hat{H}^{\text{HF}} = \frac{1}{2A}\sum_{\substack{\tau_\alpha,\tau_\beta \\ l_\alpha,l_\beta}}\sum_{\boldsymbol{k}_\alpha,\boldsymbol{k}_\beta,\boldsymbol{k}_\gamma,\boldsymbol{k}_\delta} \Bigg(\langle b^\dagger_{\boldsymbol{k}_\alpha,l_\alpha,\tau_\alpha} b_{\boldsymbol{k}_\delta,l_\alpha,\tau_\alpha}\rangle b^\dagger_{\boldsymbol{k}_\beta,l_\beta,\tau_\beta} b_{\boldsymbol{k}_\gamma,l_\beta,\tau_\beta} \tag{46}$$

$$+\langle b^\dagger_{\boldsymbol{k}_\beta,l_\beta,\tau_\beta} b_{\boldsymbol{k}_\gamma,l_\beta,\tau_\beta}\rangle b^\dagger_{\boldsymbol{k}_\alpha,l_\alpha,\tau_\alpha} b_{\boldsymbol{k}_\delta,l_\alpha,\tau_\alpha} - \langle b^\dagger_{\boldsymbol{k}_\alpha,l_\alpha,\tau_\alpha} b_{\boldsymbol{k}_\delta,l_\alpha,\tau_\alpha}\rangle \langle b^\dagger_{\boldsymbol{k}_\beta,l_\beta,\tau_\beta} b_{\boldsymbol{k}_\gamma,l_\beta,\tau_\beta}\rangle \tag{47}$$

$$-\langle b^\dagger_{\boldsymbol{k}_\alpha,l_\alpha,\tau_\alpha} b_{\boldsymbol{k}_\gamma,l_\beta,\tau_\beta}\rangle b^\dagger_{\boldsymbol{k}_\beta,l_\beta,\tau_\beta} b_{\boldsymbol{k}_\delta,l_\alpha,\tau_\alpha} - \langle b^\dagger_{\boldsymbol{k}_\beta,l_\beta,\tau_\beta} b_{\boldsymbol{k}_\delta,l_\alpha,\tau_\alpha}\rangle b^\dagger_{\boldsymbol{k}_\alpha,l_\alpha,\tau_\alpha} b_{\boldsymbol{k}_\gamma,l_\beta,\tau_\beta} \tag{48}$$

$$+\langle b^\dagger_{\boldsymbol{k}_\alpha,l_\alpha,\tau_\alpha} b_{\boldsymbol{k}_\gamma,l_\beta,\tau_\beta}\rangle \langle b^\dagger_{\boldsymbol{k}_\beta,l_\beta,\tau_\beta} b_{\boldsymbol{k}_\delta,l_\alpha,\tau_\alpha}\rangle\Bigg) V(\boldsymbol{k}_\alpha - \boldsymbol{k}_\delta)\delta_{\boldsymbol{k}_\alpha+\boldsymbol{k}_\beta,\boldsymbol{k}_\gamma+\boldsymbol{k}_\delta} \tag{49}$$

.Return $\hat{H}^{\text{HF}}_{\text{int}}$. "'

### 13.1.2

**Completion: Instructions to execute**: You will be instructed to extract the quadratic terms from the Hartree-Fock Hamiltonian, $\hat{H}^{\mathrm{HF}}$. The quadratic terms are those proportional to $b^{\dagger}_{\boldsymbol{k}_\beta,l_\beta,\tau_\beta} b_{\boldsymbol{k}_\gamma,l_\beta,\tau_\beta}$ and $b^{\dagger}_{\boldsymbol{k}_\beta,l_\beta,\tau_\beta} b_{\boldsymbol{k}_\delta,l_\alpha,\tau_\alpha}$, excluding terms that are solely expectations or products of expectations. Preserve only the quadratic terms in $\hat{H}^{\mathrm{HF}}$, denoted as $\hat{H}^{\mathrm{HF}}_{\mathrm{int}}$. Recall the expression for $\hat{H}^{\mathrm{HF}}$ as provided.

**Answer**: From the Hartree-Fock Hamiltonian $\hat{H}^{\mathrm{HF}}$, the quadratic terms can be extracted as $\hat{H}^{\mathrm{HF}}_{\mathrm{int}}$:

$$\hat{H}^{\mathrm{HF}}_{\mathrm{int}} = \frac{1}{2A} \sum_{\substack{\tau_\alpha,\tau_\beta \\ l_\alpha,l_\beta}} \sum_{\boldsymbol{k}_\alpha,\boldsymbol{k}_\beta,\boldsymbol{k}_\gamma,\boldsymbol{k}_\delta} \Bigg( \langle b^{\dagger}_{\boldsymbol{k}_\alpha,l_\alpha,\tau_\alpha} b_{\boldsymbol{k}_\delta,l_\alpha,\tau_\alpha} \rangle b^{\dagger}_{\boldsymbol{k}_\beta,l_\beta,\tau_\beta} b_{\boldsymbol{k}_\gamma,l_\beta,\tau_\beta} \tag{50}$$

$$+\langle b^{\dagger}_{\boldsymbol{k}_\beta,l_\beta,\tau_\beta} b_{\boldsymbol{k}_\gamma,l_\beta,\tau_\beta} \rangle b^{\dagger}_{\boldsymbol{k}_\alpha,l_\alpha,\tau_\alpha} b_{\boldsymbol{k}_\delta,l_\alpha,\tau_\alpha} \tag{51}$$

$$-\langle b^{\dagger}_{\boldsymbol{k}_\alpha,l_\alpha,\tau_\alpha} b_{\boldsymbol{k}_\gamma,l_\beta,\tau_\beta} \rangle b^{\dagger}_{\boldsymbol{k}_\beta,l_\beta,\tau_\beta} b_{\boldsymbol{k}_\delta,l_\alpha,\tau_\alpha} \tag{52}$$

$$-\langle b^{\dagger}_{\boldsymbol{k}_\beta,l_\beta,\tau_\beta} b_{\boldsymbol{k}_\delta,l_\alpha,\tau_\alpha} \rangle b^{\dagger}_{\boldsymbol{k}_\alpha,l_\alpha,\tau_\alpha} b_{\boldsymbol{k}_\gamma,l_\beta,\tau_\beta} \Bigg) V(\boldsymbol{k}_\alpha - \boldsymbol{k}_\delta) \delta_{\boldsymbol{k}_\alpha+\boldsymbol{k}_\beta,\boldsymbol{k}_\gamma+\boldsymbol{k}_\delta} \tag{53}$$

This expression for $\hat{H}^{\mathrm{HF}}_{\mathrm{int}}$ includes only the quadratic terms from the Hartree-Fock Hamiltonian. Each term involves a product of a creation operator and an annihilation operator, weighted by the expectation values of the corresponding operator pairs. The interaction potential $V(\boldsymbol{k}_\alpha - \boldsymbol{k}_\delta)$ is included, and momentum conservation is enforced by the delta function $\delta_{\boldsymbol{k}_\alpha+\boldsymbol{k}_\beta,\boldsymbol{k}_\gamma+\boldsymbol{k}_\delta}$. This Hamiltonian represents the effective interaction between particles (holes) in the system after applying the Hartree-Fock approximation.

# 14 Combine Hartree/Fock terms

## 14.1 Extraction

### 14.1.1

**Prompt: Extraction Abstract** We present a theory on the quantum phase diagram of AB-stacked $MoTe_2/WSe_2$ using a self-consistent Hartree-Fock calculation performed in the plane-wave basis, motivated by the observation of topological states in this system. At filling factor $\nu = 2$ (two holes per moir'e unit cell), Coulomb interaction can stabilize a $\mathbb{Z}_2$ topological insulator by opening a charge gap. At $\nu = 1$, the interaction induces three classes of competing states, spin density wave states, an in-plane ferromagnetic state, and a valley polarized state, which undergo first-order phase transitions tuned by an out-of-plane displacement field. The valley polarized state becomes a Chern insulator for certain displacement fields. Moreover, we predict a topological charge density wave forming a honeycomb lattice with ferromagnetism at $\nu = 2/3$. Future directions on this versatile system hosting a rich set of quantum phases are discussed.

**Question**: 1. Do you need to keep both Hartree term and fock term in order to solve the problem in this paper?

### 14.1.2

**Completion:** 1. **Do you need to keep both Hartree term and Fock term in order to solve the problem in this paper? Quote**: "Coulomb interaction can stabilize a $\mathbb{Z}_2$ topological insulator" and "interaction induces three classes of competing states, spin density wave states, an in-plane ferromagnetic state, and a valley polarized state" **Explanation**: The abstract indicates the importance of Coulomb interactions in stabilizing various states in the system, including a $\mathbb{Z}_2$ topological insulator, spin density wave states, an in-plane ferromagnetic state, and a valley polarized state. The Hartree and Fock terms represent different aspects of electron-electron interactions in the Hartree-Fock approximation. The Hartree term accounts for the average field effect due to electron-electron interactions, while the Fock term incorporates the exchange interaction, which is crucial for capturing the quantum mechanical nature of electrons, especially in systems showing topological and magnetic properties.

Given the complexity and variety of states mentioned, including those influenced by topological aspects and phase transitions, both Hartree and Fock terms seem necessary. The Hartree term would contribute to understanding the general field effects due to electron-electron interactions, while the Fock term is essential for capturing the exchange effects that can lead to phenomena like spin density waves and other magnetic states.

**Answer**: Yes, both the Hartree term and the Fock term should be retained to solve the problem in this paper, as they collectively capture the critical aspects of electron-electron interactions necessary for understanding the various complex states mentioned, including topological insulators, spin density wave states, ferromagnetic states, and valley polarized states.

## 14.2 Execution-Notation

### 14.2.1

**Prompt: Execution: Notation** Here I provide the notation you should use for this task. You should combine it with previous **Execution: Core information** to obtain the full instruction for execution. In the response, you will first repeat the instruction for execution and then proceed with the calculation. "' You will be instructed to simplify the quadratic term $\hat{H}_{\text{int}}^{\text{HF}}$ through relabeling the index to combine the two Hartree/Fock term into one Hartree/Fock term.The logic is that the expected value ($\langle b_{\boldsymbol{k}_\alpha,l_\alpha,\tau_\alpha}^\dagger b_{\boldsymbol{k}_\delta,l_\alpha,\tau_\alpha}\rangle$) in the first Hartree term ($\langle b_{\tau_\alpha,l_\alpha}^\dagger(k_\alpha) b_{\tau_\alpha,l_\alpha}(k_\delta)\rangle b_{\tau_\beta,l_\beta}^\dagger(k_\beta) b_{\tau_\beta,l_\beta}(k_3)$) has the same form as the quadratic operators in the second Hartree term ($\langle b_{\tau_\beta,l_\beta}^\dagger(k_\beta) b_{\tau_\beta,l_\beta}(k_\gamma)\rangle b_{\tau_\alpha,l_\alpha}^\dagger(k_\alpha) b_{\tau_\alpha,l_\alpha}(k_\delta)$), and vice versa. The same applies to the Fock term.This means, if you relabel the index by swapping the index in the "expected value" and "quadratic operators" in the second Hartree term, you can make the second Hartree term look identical to the first Hartree term, as long as $V(q)=V(-q)$, which is naturally satisfied in Coulomb interaction. You should follow the EXAMPLE below to simplify it through relabeling the index.You should perform this trick of "relabeling the index" for both two Hartree terms and two Fock terms to reduce them to one Hartree term, and one Fock term.You should recall that $\hat{H}_{\text{int}}^{\text{HF}}$ is

$$\hat{H}_{\text{int}}^{\text{HF}} = \frac{1}{2A}\sum_{\substack{\tau_\alpha,\tau_\beta\\ l_\alpha,l_\beta}}\sum_{\boldsymbol{k}_\alpha,\boldsymbol{k}_\beta,\boldsymbol{k}_\gamma,\boldsymbol{k}_\delta}\Bigg(\langle b_{\boldsymbol{k}_\alpha,l_\alpha,\tau_\alpha}^\dagger b_{\boldsymbol{k}_\delta,l_\alpha,\tau_\alpha}\rangle b_{\boldsymbol{k}_\beta,l_\beta,\tau_\beta}^\dagger b_{\boldsymbol{k}_\gamma,l_\beta,\tau_\beta} \tag{54}$$

$$+\langle b_{\boldsymbol{k}_\beta,l_\beta,\tau_\beta}^\dagger b_{\boldsymbol{k}_\gamma,l_\beta,\tau_\beta}\rangle b_{\boldsymbol{k}_\alpha,l_\alpha,\tau_\alpha}^\dagger b_{\boldsymbol{k}_\delta,l_\alpha,\tau_\alpha} - \langle b_{\boldsymbol{k}_\alpha,l_\alpha,\tau_\alpha}^\dagger b_{\boldsymbol{k}_\gamma,l_\beta,\tau_\beta}\rangle b_{\boldsymbol{k}_\beta,l_\beta,\tau_\beta}^\dagger b_{\boldsymbol{k}_\delta,l_\alpha,\tau_\alpha} \tag{55}$$

$$-\langle b_{\boldsymbol{k}_\beta,l_\beta,\tau_\beta}^\dagger b_{\boldsymbol{k}_\delta,l_\alpha,\tau_\alpha}\rangle b_{\boldsymbol{k}_\alpha,l_\alpha,\tau_\alpha}^\dagger b_{\boldsymbol{k}_\gamma,l_\beta,\tau_\beta}\Bigg) V(\boldsymbol{k}_\alpha-\boldsymbol{k}_\delta)\delta_{\boldsymbol{k}_\alpha+\boldsymbol{k}_\beta,\boldsymbol{k}_\gamma+\boldsymbol{k}_\delta} \tag{56}$$

.Return the simplified $\hat{H}_{\text{int}}^{\text{HF}}$ which reduces from four terms (two Hartree and two Fock terms) to only two terms (one Hartree and one Fock term)

===EXAMPLE: Given a Hamiltonian $\hat{H} = \sum_{k_1,k_2,k_3,k_4,\sigma_1,\sigma_2,\sigma_3,\sigma_4} V(k_1-k_4)(\langle c_{\sigma_1}^\dagger(k_1) c_{\sigma_4}(k_4)\rangle c_{\sigma_2}^\dagger(k_2) c_{\sigma_3}(k_3) + \langle c_{\sigma_2}^\dagger(k_2) c_{\sigma_3}(k_3)\rangle c_{\sigma_1}^\dagger(k_1) c_{\sigma_4}(k_4))\delta_{k_1+k_2,k_3+k_4}$, where $V(q)=V(-q)$.In the second term, we relabel the index to swap the index in expected value and the index in quadratic operators, namely, $\sigma_1\leftrightarrow\sigma_2$, $\sigma_3\leftrightarrow\sigma_4$, $k_1\leftrightarrow k_2$, $k_3\leftrightarrow k_4$. After the replacement, the second term becomes $\sum_{k_1,k_2,k_3,k_4,\sigma_1,\sigma_2,\sigma_3,\sigma_4} V(k_2-k_3)\langle c_{\sigma_1}^\dagger(k_1) c_{\sigma_4}(k_4)\rangle c_{\sigma_2}^\dagger(k_2) c_{\sigma_3}(k_3)\delta_{k_4+k_3,k_2+k_1}$.Note that the Kronecker dirac function $\delta_{k_4+k_3,k_2+k_1}$ implies $k_1+k_2=k_3+k_4$, i.e., $k_2-k_3=k_4-k_1$. Thus, the second term simplifies to $\sum_{k_1,k_2,k_3,k_4,\sigma_1,\sigma_2,\sigma_3,\sigma_4} V(k_4-k_1)\langle c_{\sigma_1}^\dagger(k_1) c_{\sigma_4}(k_4)\rangle c_{\sigma_2}^\dagger(k_2) c_{\sigma_3}(k_3)\delta_{k_4+k_3,k_2+k_1}$. Because $V(q)=V(-q)$, meaning $V(k_4-k_1)=V(k_1-k_4)$, the second term further simplifies to $\sum_{k_1,k_2,k_3,k_4,\sigma_1,\sigma_2,\sigma_3,\sigma_4} V(k_1-k_4)\langle c_{\sigma_1}^\dagger(k_1) c_{\sigma_4}(k_4)\rangle c_{\sigma_2}^\dagger(k_2) c_{\sigma_3}(k_3)\delta_{k_4+k_3,k_2+k_1}$. Note that this form of second term after relabeling is identical to the first term.Finally, we have the simplified Hamiltonian as $\hat{H} = 2\sum_{k_1,k_2,k_3,k_4,\sigma_1,\sigma_2,\sigma_3,\sigma_4} V(k_1-k_4)\langle c_{\sigma_1}^\dagger(k_1) c_{\sigma_4}(k_4)\rangle c_{\sigma_2}^\dagger(k_2) c_{\sigma_3}(k_3)\delta_{k_4+k_3,k_2+k_1}$. "'

### 14.2.2

**Completion: Instructions to execute**: You will be instructed to simplify the quadratic term $\hat{H}_{\text{int}}^{\text{HF}}$ by relabeling indices to combine the two Hartree and two Fock terms into one Hartree term and one Fock term. The expected value in one term can be made identical to the quadratic operators in another term by relabeling, as long as $V(q)=V(-q)$, which is naturally satisfied in the Coulomb interaction. Perform this relabeling for both the Hartree and Fock terms to reduce them to one Hartree term and one Fock term. Recall that $\hat{H}_{\text{int}}^{\text{HF}}$ is given by the specified formula with four terms. Return the simplified $\hat{H}_{\text{int}}^{\text{HF}}$ with only two terms.

**Answer**: Starting with the Hartree-Fock interaction Hamiltonian $\hat{H}_{\text{int}}^{\text{HF}}$ and using the relabeling trick as described, we can simplify it:

Original $\hat{H}_{\text{int}}^{\text{HF}}$:

$$\hat{H}_{\text{int}}^{\text{HF}} = \frac{1}{2A}\sum_{\substack{\tau_\alpha,\tau_\beta\\ l_\alpha,l_\beta}}\sum_{\boldsymbol{k}_\alpha,\boldsymbol{k}_\beta,\boldsymbol{k}_\gamma,\boldsymbol{k}_\delta}\Bigg(\langle b_{\boldsymbol{k}_\alpha,l_\alpha,\tau_\alpha}^\dagger b_{\boldsymbol{k}_\delta,l_\alpha,\tau_\alpha}\rangle b_{\boldsymbol{k}_\beta,l_\beta,\tau_\beta}^\dagger b_{\boldsymbol{k}_\gamma,l_\beta,\tau_\beta} \tag{57}$$

$$+\langle b_{\boldsymbol{k}_\beta,l_\beta,\tau_\beta}^\dagger b_{\boldsymbol{k}_\gamma,l_\beta,\tau_\beta}\rangle b_{\boldsymbol{k}_\alpha,l_\alpha,\tau_\alpha}^\dagger b_{\boldsymbol{k}_\delta,l_\alpha,\tau_\alpha}\Bigg) V(\boldsymbol{k}_\alpha-\boldsymbol{k}_\delta)\delta_{\boldsymbol{k}_\alpha+\boldsymbol{k}_\beta,\boldsymbol{k}_\gamma+\boldsymbol{k}_\delta} \tag{58}$$

$$-\langle b_{\boldsymbol{k}_\alpha,l_\alpha,\tau_\alpha}^\dagger b_{\boldsymbol{k}_\gamma,l_\beta,\tau_\beta}\rangle b_{\boldsymbol{k}_\beta,l_\beta,\tau_\beta}^\dagger b_{\boldsymbol{k}_\delta,l_\alpha,\tau_\alpha} - \langle b_{\boldsymbol{k}_\beta,l_\beta,\tau_\beta}^\dagger b_{\boldsymbol{k}_\delta,l_\alpha,\tau_\alpha}\rangle b_{\boldsymbol{k}_\alpha,l_\alpha,\tau_\alpha}^\dagger b_{\boldsymbol{k}_\gamma,l_\beta,\tau_\beta} \tag{59}$$

Relabeling the indices in the second and fourth terms: - Swap $\boldsymbol{k}_\alpha \leftrightarrow \boldsymbol{k}_\beta$ and $\boldsymbol{k}_\gamma \leftrightarrow \boldsymbol{k}_\delta$ in the second term. - Swap $\boldsymbol{k}_\alpha \leftrightarrow \boldsymbol{k}_\beta$ and $\boldsymbol{k}_\gamma \leftrightarrow \boldsymbol{k}_\delta$ in the fourth term.

After relabeling, these terms become identical to the first and third terms respectively, due to $V(\boldsymbol{k}_\alpha - \boldsymbol{k}_\delta) = V(-(\boldsymbol{k}_\alpha - \boldsymbol{k}_\delta)) = V(\boldsymbol{k}_\delta - \boldsymbol{k}_\alpha)$, and the delta function enforcing momentum conservation. Thus, the simplified $\hat{H}^{\rm HF}_{\rm int}$ reduces to:

$$\hat{H}^{\rm HF}_{\rm int} = \frac{1}{A} \sum_{\substack{\tau_\alpha,\tau_\beta \\ l_\alpha,l_\beta}} \sum_{\boldsymbol{k}_\alpha,\boldsymbol{k}_\beta,\boldsymbol{k}_\gamma,\boldsymbol{k}_\delta} \Bigg( \langle b^\dagger_{\boldsymbol{k}_\alpha,l_\alpha,\tau_\alpha} b_{\boldsymbol{k}_\delta,l_\alpha,\tau_\alpha}\rangle b^\dagger_{\boldsymbol{k}_\beta,l_\beta,\tau_\beta} b_{\boldsymbol{k}_\gamma,l_\beta,\tau_\beta} \tag{60}$$

$$- \langle b^\dagger_{\boldsymbol{k}_\alpha,l_\alpha,\tau_\alpha} b_{\boldsymbol{k}_\gamma,l_\beta,\tau_\beta}\rangle b^\dagger_{\boldsymbol{k}_\beta,l_\beta,\tau_\beta} b_{\boldsymbol{k}_\delta,l_\alpha,\tau_\alpha} \Bigg) V(\boldsymbol{k}_\alpha - \boldsymbol{k}_\delta)\delta_{\boldsymbol{k}_\alpha+\boldsymbol{k}_\beta,\boldsymbol{k}_\gamma+\boldsymbol{k}_\delta} \tag{61}$$

This simplified Hamiltonian consists of just two terms, one Hartree and one Fock term, thus reducing the complexity of $\hat{H}^{\rm HF}_{\rm int}$ in the Hartree-Fock approximation.

# 15 Identify order parameters in Hartree term (extended BZ)

## 15.1 Execution-Notation

### 15.1.1

**Prompt: Execution: Notation** Here I provide the notation you should use for this task. You should combine it with previous **Execution: Core information** to obtain the full instruction for execution. In the response, you will first repeat the instruction for execution and then proceed with the calculation. "' You will be instructed to simplify the Hartree term in $H_{\rm Hartree}$ by reducing the momentum inside the expected value $\langle b^\dagger_{l_\alpha,\tau_\alpha,q_\alpha}(k_\alpha) b_{l_\alpha,\tau_\alpha,q_\delta}(k_\delta)\rangle$.The expected value $\langle b^\dagger_{l_\alpha,\tau_\alpha,q_\alpha}(k_\alpha) b_{l_\alpha,\tau_\alpha,q_\delta}(k_\delta)\rangle$ is only nonzero when the two momenta $k_i, k_j$ are the same, namely, $\langle b^\dagger_{l_\alpha,\tau_\alpha,q_\alpha}(k_\alpha) b_{l_\alpha,\tau_\alpha,q_\delta}(k_\delta)\rangle = \langle b^\dagger_{l_\alpha,\tau_\alpha,q_\alpha}(k_\alpha) b_{l_\alpha,\tau_\alpha,q_\delta}(k_\delta)\rangle \delta_{k_\alpha,k_\delta}$.You should use the property of Kronecker delta function $\delta_{k_i,k_j}$ to reduce one momentum $k_i$ but not $b_i$. Once you reduce one momentum inside the expected value $\langle \dots \rangle$. You will also notice the total momentum conservation will reduce another momentum in the quadratic term. Therefore, you should end up with only two momenta left in the summation.You should follow the EXAMPLE below to reduce one momentum in the Hartree term, and another momentum in the quadratic term.You should recall that $H_{\rm Hartree}$ is

$$\hat{H}^{\rm HF}_{\rm int} = \frac{1}{A} \sum_{\substack{\tau_\alpha,\tau_\beta \\ l_\alpha,l_\beta}} \sum_{\boldsymbol{k}_\alpha,\boldsymbol{k}_\beta,\boldsymbol{k}_\gamma,\boldsymbol{k}_\delta} \langle b^\dagger_{\boldsymbol{k}_\alpha,l_\alpha,\tau_\alpha} b_{\boldsymbol{k}_\delta,l_\alpha,\tau_\alpha}\rangle b^\dagger_{\boldsymbol{k}_\beta,l_\beta,\tau_\beta} b_{\boldsymbol{k}_\gamma,l_\beta,\tau_\beta} V(\boldsymbol{k}_\alpha - \boldsymbol{k}_\delta)\delta_{\boldsymbol{k}_\alpha+\boldsymbol{k}_\beta,\boldsymbol{k}_\gamma+\boldsymbol{k}_\delta} \tag{62}$$

.Return the final simplified Hartree term $H_{\rm Hartree}$.

===EXAMPLE:Given a Hamiltonian where the Hartree term $\hat{H}^{Hartree} = \sum_{k_1,k_2,k_3,k_4,b_1,b_2,b_3,b_4} V(k_1 - k_4 + b_1 - b_4) \langle c_{b_1}^\dagger(k_1) c_{b_4}(k_4)\rangle c_{b_2}^\dagger(k_2) c_{b_3}(k_3) \delta_{k_1+k_2+b_1+b_2,k_3+k_4+b_3+b_4}$, where $k_i$ is the momentum inside first Brilloun zone and $b_i$ is the reciprocal lattice.Inside the expected value, we realize $\langle c_{b_1}^\dagger(k_1) c_{b_4}(k_4)\rangle$ is nonzero only when $k_1 = k_4$, i.e., $\langle c_{b_1}^\dagger(k_1) c_{b_4}(k_4)\rangle = \langle c_{b_1}^\dagger(k_1) c_{b_4}(k_4)\rangle\delta_{k_1,k_4}$.Thus, the Hartree term becomes $\sum_{k_1,k_2,k_3,k_4,b_1,b_2,b_3,b_4} V(k_1 - k_4 + b_1 - b_4) \langle c_{b_1}^\dagger(k_1) c_{b_4}(k_4)\rangle \delta_{k_1,k_4} c_{b_2}^\dagger(k_2) c_{b_3}(k_3) \delta_{k_1+k_2+b_1+b_2,k_3+k_4+b_3+b_4}$.Use the property of Kronecker delta function $\delta_{k_1,k_4}$ to sum over $k_4$, we have $\sum_{k_1,k_2,k_3,b_1,b_2,b_3,b_4} V(k_1 - k_1 + b_1 - b_4) \langle c_{b_1}^\dagger(k_1) c_{b_4}(k_1)\rangle c_{b_2}^\dagger(k_2) c_{b_3}(k_3) \delta_{k_1+k_2+b_1+b_2,k_3+k_1+b_3+b_4} = \sum_{k_1,k_2,k_3,b_1,b_2,b_3,b_4} V(b_1 - b_4) \langle c_{b_1}^\dagger(k_1) c_{b_4}(k_1)\rangle c_{b_2}^\dagger(k_2) c_{b_3}(k_3) \delta_{k_2+b_1+b_2,k_3+b_3+b_4}$.Because $k_i$ is momentum inside first Brilloun zone while $b_i$ is the reciprocal lattice. It is only when $k_2 = k_3$ that $\delta_{k_2+b_1+b_2,k_3+b_3+b_4}$ is nonzero, i.e., $\delta_{k_2+b_1+b_2,k_3+b_3+b_4} = \delta_{b_1+b_2,b_3+b_4}\delta_{k_2,k_3}$. Therefore, the Hartree term simplifies to $\sum_{k_1,k_2,k_3,b_1,b_2,b_3,b_4} V(b_1 - b_4) \langle c_{b_1}^\dagger(k_1) c_{b_4}(k_1)\rangle c_{b_2}^\dagger(k_2) c_{b_3}(k_3) \delta_{b_1+b_2,b_3+b_4}\delta_{k_2,k_3} = \sum_{k_1,k_2,b_1,b_2,b_3,b_4} V(b_1 - b_4) \langle c_{b_1}^\dagger(k_1) c_{b_4}(k_1)\rangle c_{b_2}^\dagger(k_2) c_{b_3}(k_2) \delta_{b_1+b_2,b_3+b_4}$.Therefore, the final simplified Hartree term after reducing two momenta is $\hat{H}^{Hartree} = \sum_{k_1,k_2,b_1,b_2,b_3,b_4} V(b_1 - b_4) \langle c_{b_1}^\dagger(k_1) c_{b_4}(k_1)\rangle c_{b_2}^\dagger(k_2) c_{b_3}(k_2) \delta_{b_1+b_2,b_3+b_4}$ "'

### 15.1.2

**Completion: Instructions to execute**: You will be instructed to simplify the Hartree term in $\hat{H}^{\rm HF}_{\rm int}$ by reducing the momentum inside the expected value $\langle b^\dagger_{l_\alpha,\tau_\alpha,q_\alpha}(k_\alpha) b_{l_\alpha,\tau_\alpha,q_\delta}(k_\delta)\rangle$. This expected value is nonzero only when the two momenta $k_\alpha$ and $k_\delta$ are the same. Use the property of the Kronecker delta function to reduce one momentum $k_i$ (but not $b_i$). After reducing one momentum inside the expected value, you will notice the total momentum conservation will reduce another momentum in the quadratic term. You should end up with only two momenta left in the summation. Follow the example provided to reduce one momentum in the Hartree term and another momentum in the quadratic term. Recall that $H_{\rm Hartree}$ is given by the specified formula. Return the final simplified Hartree term $H_{\rm Hartree}$.

**Answer**: Starting with the Hartree term in $\hat{H}_{\text{int}}^{\text{HF}}$:

$$\hat{H}_{\text{int}}^{\text{HF}} = \frac{1}{A} \sum_{\substack{\tau_\alpha,\tau_\beta \\ l_\alpha,l_\beta}} \sum_{\boldsymbol{k}_\alpha,\boldsymbol{k}_\beta,\boldsymbol{k}_\gamma,\boldsymbol{k}_\delta} \langle b^\dagger_{\boldsymbol{k}_\alpha,l_\alpha,\tau_\alpha} b_{\boldsymbol{k}_\delta,l_\alpha,\tau_\alpha}\rangle b^\dagger_{\boldsymbol{k}_\beta,l_\beta,\tau_\beta} b_{\boldsymbol{k}_\gamma,l_\beta,\tau_\beta} V(\boldsymbol{k}_\alpha - \boldsymbol{k}_\delta)\delta_{\boldsymbol{k}_\alpha+\boldsymbol{k}_\beta,\boldsymbol{k}_\gamma+\boldsymbol{k}_\delta} \tag{63}$$

By using the property that the expectation value is nonzero only when $k_\alpha = k_\delta$:

$$\langle b^\dagger_{\boldsymbol{k}_\alpha,l_\alpha,\tau_\alpha} b_{\boldsymbol{k}_\delta,l_\alpha,\tau_\alpha}\rangle = \langle b^\dagger_{\boldsymbol{k}_\alpha,l_\alpha,\tau_\alpha} b_{\boldsymbol{k}_\delta,l_\alpha,\tau_\alpha}\rangle \delta_{\boldsymbol{k}_\alpha,\boldsymbol{k}_\delta} \tag{64}$$

The Hartree term becomes:

$$\hat{H}_{\text{Hartree}} = \frac{1}{A} \sum_{\substack{\tau_\alpha,\tau_\beta \\ l_\alpha,l_\beta}} \sum_{\boldsymbol{k}_\alpha,\boldsymbol{k}_\beta,\boldsymbol{k}_\gamma} \langle b^\dagger_{\boldsymbol{k}_\alpha,l_\alpha,\tau_\alpha} b_{\boldsymbol{k}_\alpha,l_\alpha,\tau_\alpha}\rangle b^\dagger_{\boldsymbol{k}_\beta,l_\beta,\tau_\beta} b_{\boldsymbol{k}_\gamma,l_\beta,\tau_\beta} V(0)\delta_{\boldsymbol{k}_\alpha+\boldsymbol{k}_\beta,\boldsymbol{k}_\gamma+\boldsymbol{k}_\alpha} \tag{65}$$

Simplifying further using momentum conservation:

$$\hat{H}_{\text{Hartree}} = \frac{1}{A} \sum_{\substack{\tau_\alpha,\tau_\beta \\ l_\alpha,l_\beta}} \sum_{\boldsymbol{k}_\alpha,\boldsymbol{k}_\beta} \langle b^\dagger_{\boldsymbol{k}_\alpha,l_\alpha,\tau_\alpha} b_{\boldsymbol{k}_\alpha,l_\alpha,\tau_\alpha}\rangle b^\dagger_{\boldsymbol{k}_\beta,l_\beta,\tau_\beta} b_{\boldsymbol{k}_\beta,l_\beta,\tau_\beta} V(0) \tag{66}$$

This is the final simplified Hartree term, $H_{\text{Hartree}}$, reduced to two momenta in the summation with the interaction potential $V(0)$ representing the static screened Coulomb interaction at zero momentum transfer.

# 16 Identify order parameters in Fock term (extended BZ)

## 16.1 Execution-Notation

### 16.1.1

**Prompt: Execution: Notation** Here I provide the notation you should use for this task. You should combine it with previous **Execution: Core information** to obtain the full instruction for execution. In the response, you will first repeat the instruction for execution and then proceed with the calculation. "' You will be instructed to simplify the Fock term in $H_{\text{Fock}}$ by reducing the momentum inside the expected value $\langle b^\dagger_{l_\alpha,\tau_\alpha,q_\alpha}(k_\alpha) b_{l_\beta,\tau_\beta,q_\gamma}(k_\gamma)\rangle$.The expected value $\langle b^\dagger_{l_\alpha,\tau_\alpha,q_\alpha}(k_\alpha) b_{l_\beta,\tau_\beta,q_\gamma}(k_\gamma)\rangle$ is only nonzero when the two momenta $k_i, k_j$ are the same, namely, $\langle b^\dagger_{l_\alpha,\tau_\alpha,q_\alpha}(k_\alpha) b_{l_\beta,\tau_\beta,q_\gamma}(k_\gamma)\rangle = \langle b^\dagger_{l_\alpha,\tau_\alpha,q_\alpha}(k_\alpha) b_{l_\beta,\tau_\beta,q_\gamma}(k_\gamma)\rangle \delta_{k_\alpha,k_\gamma}$.You should use the property of Kronecker delta function $\delta_{k_i,k_j}$ to reduce one momentum $k_i$ but not $b_i$.Once you reduce one momentum inside the expected value $\langle\dots\rangle$. You will also notice the total momentum conservation will reduce another momentum in the quadratic term. Therefore, you should end up with only two momenta left in the summation. You should follow the EXAMPLE below to reduce one momentum in the Fock term, and another momentum in the quadratic term.You should recall that $H_{\text{Fock}}$ is

$$\hat{H}_{\text{int}}^{\text{HF}} = -\frac{1}{A} \sum_{\substack{\tau_\alpha,\tau_\beta \\ l_\alpha,l_\beta}} \sum_{\boldsymbol{k}_\alpha,\boldsymbol{k}_\beta,\boldsymbol{k}_\gamma,\boldsymbol{k}_\delta} \langle b^\dagger_{\boldsymbol{k}_\alpha,l_\alpha,\tau_\alpha} b_{\boldsymbol{k}_\gamma,l_\beta,\tau_\beta}\rangle b^\dagger_{\boldsymbol{k}_\beta,l_\beta,\tau_\beta} b_{\boldsymbol{k}_\delta,l_\alpha,\tau_\alpha} V(\boldsymbol{k}_\alpha - \boldsymbol{k}_\delta)\delta_{\boldsymbol{k}_\alpha+\boldsymbol{k}_\beta,\boldsymbol{k}_\gamma+\boldsymbol{k}_\delta} \tag{67}$$

.Return the final simplified Fock term $H_{\text{Fock}}$.

===EXAMPLE:Given a Hamiltonian where the Fock term $\hat{H}^{Fock} = -\sum_{k_1,k_2,k_3,k_4,b_1,b_2,b_3,b_4} V(k_1 - k_4 + b_1 - b_4)\langle c_{b_1}^\dagger(k_1) c_{b_3}(k_3)\rangle c_{b_2}^\dagger(k_2) c_{b_4}(k_4) \delta_{k_1+k_2+b_1+b_2,k_3+k_4+b_3+b_4}$, where $k_i$ is the momentum inside first Brilloun zone and $b_i$ is the reciprocal lattice.Inside the expected value, we realize $\langle c_{b_1}^\dagger(k_1) c_{b_3}(k_3)\rangle$ is nonzero only when $k_1 = k_3$, i.e., $\langle c_{b_1}^\dagger(k_1) c_{b_3}(k_3)\rangle = \langle c_{b_1}^\dagger(k_1) c_{b_3}(k_3)\rangle\delta_{k_1,k_3}$.Thus, the Fock term becomes $-\sum_{k_1,k_2,k_3,k_4,b_1,b_2,b_3,b_4} V(k_1 - k_4 + b_1 - b_4)\langle c_{b_1}^\dagger(k_1) c_{b_3}(k_3)\rangle\delta_{k_1,k_3} c_{b_2}^\dagger(k_2) c_{b_4}(k_4) \delta_{k_1+k_2+b_1+b_2,k_3+k_4+b_3+b_4}$.Use the property of Kronecker delta function $\delta_{k_1,k_3}$ to sum over $k_3$, we have $-\sum_{k_1,k_2,k_4,b_1,b_2,b_3,b_4} V(k_1 - k_4 + b_1 - b_4)\langle c_{b_1}^\dagger(k_1) c_{b_3}(k_1)\rangle c_{b_2}^\dagger(k_2) c_{b_4}(k_4) \delta_{k_1+k_2+b_1+b_2,k_1+k_4+b_3+b_4} = -\sum_{k_1,k_2,k_4,b_1,b_2,b_3,b_4} V(k_1 - k_4 + b_1 - b_4)\langle c_{b_1}^\dagger(k_1) c_{b_3}(k_1)\rangle c_{b_2}^\dagger(k_2) c_{b_4}(k_4) \delta_{k_2+b_1+b_2,k_4+b_3+b_4}$.Because $k_i$ is momentum inside first Brilloun zone while $b_i$ is the reciprocal lattice. It is only when $k_2 = k_4$ that $\delta_{k_2+b_1+b_2,k_4+b_3+b_4}$ is nonzero, i.e., $\delta_{k_2+b_1+b_2,k_4+b_3+b_4} = \delta_{b_1+b_2,b_3+b_4}\delta_{k_2,k_4}$.Therefore, the Fock term simplifies to $-\sum_{k_1,k_2,k_4,b_1,b_2,b_3,b_4} V(k_1 - k_4 + b_1 - b_4)\langle c_{b_1}^\dagger(k_1) c_{b_3}(k_1)\rangle c_{b_2}^\dagger(k_2) c_{b_4}(k_4) \delta_{b_1+b_2,b_3+b_4}\delta_{k_2,k_4} = -\sum_{k_1,k_2,b_1,b_2,b_3,b_4} V(k_1 - k_2 + b_1 - b_4)\langle c_{b_1}^\dagger(k_1) c_{b_3}(k_1)\rangle c_{b_2}^\dagger(k_2) c_{b_4}(k_2) \delta_{b_1+b_2,b_3+b_4}$.Therefore, the final simplified Fock term after reducing two momenta is $\hat{H}^{Fock} = -\sum_{k_1,k_2,b_1,b_2,b_3,b_4} V(k_1 - k_2 + b_1 - b_4)\langle c_{b_1}^\dagger(k_1) c_{b_3}(k_1)\rangle c_{b_2}^\dagger(k_2) c_{b_4}(k_2) \delta_{b_1+b_2,b_3+b_4}$ "'

#### 16.1.2

**Completion: Instructions to execute**: You will be instructed to simplify the Fock term in $H_{\text{Fock}}$ by reducing the momentum inside the expected value $\langle b^\dagger_{l_\alpha,\tau_\alpha,q_\alpha}(k_\alpha) b_{l_\beta,\tau_\beta,q_\gamma}(k_\gamma)\rangle$. This expected value is nonzero only when the two momenta $k_\alpha$ and $k_\gamma$ are the same, i.e., $\langle b^\dagger_{l_\alpha,\tau_\alpha,q_\alpha}(k_\alpha) b_{l_\beta,\tau_\beta,q_\gamma}(k_\gamma)\rangle = \langle b^\dagger_{l_\alpha,\tau_\alpha,q_\alpha}(k_\alpha) b_{l_\beta,\tau_\beta,q_\gamma}(k_\gamma)\rangle \delta_{k_\alpha,k_\gamma}$. Use the property of the Kronecker delta function to reduce one momentum $k_i$ but not $b_i$. Once you reduce one momentum inside the expected value $\langle\dots\rangle$, total momentum conservation will reduce another momentum in the quadratic term. End up with only two momenta left in the summation. Follow the example to reduce one momentum in the Fock term, and another in the quadratic term. Recall that $H_{\text{Fock}}$ is given by the specified formula. Return the final simplified Fock term $H_{\text{Fock}}$.

**Answer**: Starting with the Fock term in $\hat{H}^{\text{HF}}_{\text{int}}$:

$$\hat{H}^{\text{HF}}_{\text{int}} = -\frac{1}{A} \sum_{\substack{\tau_\alpha,\tau_\beta \\ l_\alpha,l_\beta}} \sum_{\boldsymbol{k}_\alpha,\boldsymbol{k}_\beta,\boldsymbol{k}_\gamma,\boldsymbol{k}_\delta} \langle b^\dagger_{\boldsymbol{k}_\alpha,l_\alpha,\tau_\alpha} b_{\boldsymbol{k}_\gamma,l_\beta,\tau_\beta}\rangle b^\dagger_{\boldsymbol{k}_\beta,l_\beta,\tau_\beta} b_{\boldsymbol{k}_\delta,l_\alpha,\tau_\alpha} V(\boldsymbol{k}_\alpha - \boldsymbol{k}_\delta) \delta_{\boldsymbol{k}_\alpha+\boldsymbol{k}_\beta,\boldsymbol{k}_\gamma+\boldsymbol{k}_\delta} \tag{68}$$

By using the property that the expectation value is nonzero only when $k_\alpha = k_\gamma$:

$$\langle b^\dagger_{\boldsymbol{k}_\alpha,l_\alpha,\tau_\alpha} b_{\boldsymbol{k}_\gamma,l_\beta,\tau_\beta}\rangle = \langle b^\dagger_{\boldsymbol{k}_\alpha,l_\alpha,\tau_\alpha} b_{\boldsymbol{k}_\gamma,l_\beta,\tau_\beta}\rangle \delta_{\boldsymbol{k}_\alpha,\boldsymbol{k}_\gamma} \tag{69}$$

The Fock term becomes:

$$\hat{H}_{\text{Fock}} = -\frac{1}{A} \sum_{\substack{\tau_\alpha,\tau_\beta \\ l_\alpha,l_\beta}} \sum_{\boldsymbol{k}_\alpha,\boldsymbol{k}_\beta,\boldsymbol{k}_\delta} \langle b^\dagger_{\boldsymbol{k}_\alpha,l_\alpha,\tau_\alpha} b_{\boldsymbol{k}_\alpha,l_\beta,\tau_\beta}\rangle b^\dagger_{\boldsymbol{k}_\beta,l_\beta,\tau_\beta} b_{\boldsymbol{k}_\delta,l_\alpha,\tau_\alpha} V(\boldsymbol{k}_\alpha - \boldsymbol{k}_\delta) \delta_{\boldsymbol{k}_\alpha+\boldsymbol{k}_\beta,\boldsymbol{k}_\alpha+\boldsymbol{k}_\delta} \tag{70}$$

Simplifying further using momentum conservation:

$$\hat{H}_{\text{Fock}} = -\frac{1}{A} \sum_{\substack{\tau_\alpha,\tau_\beta \\ l_\alpha,l_\beta}} \sum_{\boldsymbol{k}_\alpha,\boldsymbol{k}_\beta} \langle b^\dagger_{\boldsymbol{k}_\alpha,l_\alpha,\tau_\alpha} b_{\boldsymbol{k}_\alpha,l_\beta,\tau_\beta}\rangle b^\dagger_{\boldsymbol{k}_\beta,l_\beta,\tau_\beta} b_{\boldsymbol{k}_\beta,l_\alpha,\tau_\alpha} V(\boldsymbol{k}_\alpha - \boldsymbol{k}_\beta) \tag{71}$$

This is the final simplified Fock term, $H_{\text{Fock}}$, reduced to two momenta in the summation with the interaction potential $V(\boldsymbol{k}_\alpha - \boldsymbol{k}_\beta)$ representing the screened Coulomb interaction between the relevant momentum states.

# 17 Final form of iteration in quadratic terms

## 17.1 Execution-Notation

#### 17.1.1

**Prompt: Execution: Notation** Here I provide the notation you should use for this task. You should combine it with previous **Execution: Core information** to obtain the full instruction for execution. In the response, you will first repeat the instruction for execution and then proceed with the calculation. "' You will now be instructed to combine the Hartree term $H_{\text{Hartree}}$ and the Fock term $H_{\text{Fock}}$.You should recall that the Hartree term $H_{\text{Hartree}} = \frac{1}{A}\sum_{\substack{\tau_\alpha,\tau_\beta \\ l_\alpha,l_\beta}} \sum_{\boldsymbol{k}_\alpha,\boldsymbol{k}_\beta} \langle b^\dagger_{\boldsymbol{k}_\alpha,l_\alpha,\tau_\alpha} b_{\boldsymbol{k}_\alpha,l_\alpha,\tau_\alpha}\rangle b^\dagger_{\boldsymbol{k}_\beta,l_\beta,\tau_\beta} b_{\boldsymbol{k}_\beta,l_\beta,\tau_\beta} V(0)$ ,and the Fock term $H_{\text{Fock}} = -\frac{1}{A}\sum_{\substack{\tau_\alpha,\tau_\beta \\ l_\alpha,l_\beta}} \sum_{\boldsymbol{k}_\alpha,\boldsymbol{k}_\beta} \langle b^\dagger_{\boldsymbol{k}_\alpha,l_\alpha,\tau_\alpha} b_{\boldsymbol{k}_\alpha,l_\beta,\tau_\beta}\rangle b^\dagger_{\boldsymbol{k}_\beta,l_\beta,\tau_\beta} b_{\boldsymbol{k}_\beta,l_\alpha,\tau_\alpha} V(\boldsymbol{k}_\alpha - \boldsymbol{k}_\beta)$ .You should perform the same trick of relabeling the index in the Fock term to make the quadratic operators in the Fock term the same as those in the Hartree term. The relabeling should be done with a swap : Not needed. You should add them, relabel the index in Fock term, and simply their sum. Return the final sum of Hartree and Fock term. "'

#### 17.1.2

**Completion: Instructions to execute**: You will be instructed to combine the Hartree term $H_{\text{Hartree}}$ and the Fock term $H_{\text{Fock}}$. Recall the expressions for both the Hartree and Fock terms. Relabel the indices in the Fock term to make the quadratic operators the same as those in the Hartree term, if needed. Then add them together and simplify their sum. Return the final combined sum of the Hartree and Fock terms.

**Answer**: Starting with the given Hartree term $H_{\text{Hartree}}$ and Fock term $H_{\text{Fock}}$:

Hartree term $H_{\text{Hartree}}$:

$$H_{\text{Hartree}} = \frac{1}{A} \sum_{\substack{\tau_\alpha,\tau_\beta \\ l_\alpha,l_\beta}} \sum_{\boldsymbol{k}_\alpha,\boldsymbol{k}_\beta} \langle b^\dagger_{\boldsymbol{k}_\alpha,l_\alpha,\tau_\alpha} b_{\boldsymbol{k}_\alpha,l_\alpha,\tau_\alpha}\rangle b^\dagger_{\boldsymbol{k}_\beta,l_\beta,\tau_\beta} b_{\boldsymbol{k}_\beta,l_\beta,\tau_\beta} V(0) \tag{72}$$

Fock term $H_{\text{Fock}}$:

$$H_{\text{Fock}} = -\frac{1}{A} \sum_{\substack{\tau_\alpha,\tau_\beta \\ l_\alpha,l_\beta}} \sum_{\boldsymbol{k}_\alpha,\boldsymbol{k}_\beta} \langle b^\dagger_{\boldsymbol{k}_\alpha,l_\alpha,\tau_\alpha} b_{\boldsymbol{k}_\alpha,l_\beta,\tau_\beta} \rangle b^\dagger_{\boldsymbol{k}_\beta,l_\beta,\tau_\beta} b_{\boldsymbol{k}_\beta,l_\alpha,\tau_\alpha} V(\boldsymbol{k}_\alpha - \boldsymbol{k}_\beta) \tag{73}$$

Since the quadratic operators in the Fock term already match those in the Hartree term, there is no need for additional relabeling. The final combined sum of the Hartree and Fock terms is:

$$H_{\text{combined}} = H_{\text{Hartree}} + H_{\text{Fock}} \tag{74}$$

$$= \frac{1}{A} \sum_{\substack{\tau_\alpha,\tau_\beta \\ l_\alpha,l_\beta}} \sum_{\boldsymbol{k}_\alpha,\boldsymbol{k}_\beta} \Bigg( \langle b^\dagger_{\boldsymbol{k}_\alpha,l_\alpha,\tau_\alpha} b_{\boldsymbol{k}_\alpha,l_\alpha,\tau_\alpha} \rangle b^\dagger_{\boldsymbol{k}_\beta,l_\beta,\tau_\beta} b_{\boldsymbol{k}_\beta,l_\beta,\tau_\beta} V(0) \tag{75}$$

$$- \langle b^\dagger_{\boldsymbol{k}_\alpha,l_\alpha,\tau_\alpha} b_{\boldsymbol{k}_\alpha,l_\beta,\tau_\beta} \rangle b^\dagger_{\boldsymbol{k}_\beta,l_\beta,\tau_\beta} b_{\boldsymbol{k}_\beta,l_\alpha,\tau_\alpha} V(\boldsymbol{k}_\alpha - \boldsymbol{k}_\beta) \Bigg) \tag{76}$$

This expression represents the final combined sum of the Hartree and Fock terms, simplified and ready to be used in further calculations.

## F. Code

All codes and data used in this work can be found at [17].

## G. Example of spotting a typo

The LLM spotted a typo in the Hamiltonian Eq.(1) in [4], which is the kinetic term in the Emery model. The correct Hamiltonian should include another hopping process connecting the $d$-orbital at $i$ and the $p$-orbital at $i-\hat{\nu}/2$ with an opposite hopping magnitude than $i$ and $i+\hat{\nu}/2$, where $\hat{\nu}=x,y$, namely, the missing term is $t_{pd}\sum_{i,s}\sum_{\nu}\left(\hat{d}^{\dagger}_{i,s}\hat{p}_{i-\hat{\nu}/2,s}+\text{ h.c. }\right)$. The same term should also be included for the hopping process between the $p$-orbitals at $i+\hat{\nu}/2$ and $i+\hat{\nu}'/2$. The typo becomes evident when the LLM performed the Fourier transform of the original Hamiltonian Eq.(1) in the paper and generated a different equation than Eq. (10-11) in momentum space, and was later verified by manual check.

### H. One-shot prompting for extraction

TEMPLATE: You will be instructed to convert the interacting Hamiltonian, {second_int_symbol}, in the {single-particle|second-quantized} form the basis in real space to the basis in momentum space.
To do that, you should apply the Fourier transformation to {real_creation_op} in the real space to the {momentum_creation_op} in the momentum space, which is defined as {definition_of_Fourier_Transformation}, where {real_variable} is integrated over all sites in the entire real space, and {momentum_var} is defined within the first Brillouin zone. You should follow the EXAMPLE below to apply the Fourier transformation. [Note that interaction have no position dependence now: {TRUE|FALSE}]
You should recall that {second_int_symbol} is {expression_int}. Express {second_int_symbol} in terms of {momentum_creation_op}. Simplify any summation index if possible.

===
Here is an example of an excerpt and its completed template.
EXCERPT:

$$H = \sum_{s}\sum_{i,j} t_s\left(\boldsymbol{R}_i - \boldsymbol{R}_j\right) c_{i,s}^{\dagger} c_{j,s} \\ + \frac{1}{2}\sum_{s,s'}\sum_{i,j} U(\boldsymbol{R}_i - \boldsymbol{R}_j) c_{i,s}^{\dagger} c_{j,s'}^{\dagger} c_{j,s'} c_{i,s},$$

where $t_s\left(\boldsymbol{R}_i - \boldsymbol{R}_j\right)$ is the hopping between the moiré lattice site $i$ and $j$, fitted from the first moiré valence band of twisted $WSe_2$ at $\pm K$ valleys in the noninteracting picture, and $s = \uparrow$ and $\downarrow$ are coupled with the $+K$ and $-K$ valleys [9]. $U(\boldsymbol{R}_i - \boldsymbol{R}_j)$ describes the Coulomb repulsion between site $i$ and $j$. We control the range of the Coulomb interactions by including a finite number of neighbors coupled in the theory. These neighbors are denoted by hexagonal "shells" (e.g., on-site interaction $U_0$ is 0-shell, 1-shell means six nearest-neighbor interactions $U_1$ plus $U_0$) in the following results. By comparing the results of short-range (few shells) and long-range (many shells) interactions, we investigate the role of the interaction range.

COMPLETED TEMPLATE: You will be instructed to convert the interacting Hamiltonian, $H_{int}$, in the second-quantized form the basis in real space to the basis in momentum space.
To do that, you should apply the Fourier transformation to $c_{i,s}^{\dagger}$ in the real space to the $c_{k,s}^{\dagger}$ in the momentum space, which is defined as $c_{k,s}^{\dagger} = \frac{1}{\sqrt{N}}\sum_i c_{R_{i,s}}^{\dagger} e^{ik\cdot R_i}$, where $\boldsymbol{R}_i$ is integrated over all sites in the entire real space, and k is defined within the first Brillouin zone. You should follow the EXAMPLE below to apply the Fourier transformation. [Note that interaction have no position dependence now: FALSE]
You should recall that $H_{int}$ is {expression_int}.
Express $H_{int}$ in terms of $c_{k,s}^{\dagger}$. Simplify any summation index if possible.

===
Now generate the completed template for the following excerpt.
EXCERPT: `<Test Excerpt>`

In this section, we examined the performance on the extraction task for the template $T_4$, Fourier transforming the interaction term $H_{int}$ in a One-Shot-setting (eg: [18]), i.e. the model is additionally provided a single example of an excerpt and its correct target output (see H). The input and annotated template, corresponding to arXiv:2110.11330 served as the One-Shot example. We tested the performance on 5 other papers that had this task: arXiv:{1106.6060, 1310.2674, 2008.08998, 2012.04554, 2110.11330, 2308.03843}. Since each task contained 8 placeholders, the baseline performance on the substitutions for the 40 placeholders in the baseline (Zero-Shot) setting and the One-Shot setting was examined using HP's scores. The performance across all placeholders in the baseline setting was $43.8 \pm 7.6$ on 100. After One-Shot prompting, the performance was $80 \pm 5.9$ on 100 (Main, Figure 4, Panel i)). One-Shot prompting significantly enhances performance on extraction for this task, in particular for the placeholders corresponding to `change of basis`, `k-basis creation operator` and `r-basis creation operator`, and improves our ability to elicit substi-

tutions that are more aligned with the target outputs.

### I. Automatic Evaluation

In this section, we examined whether GPT-4 was able to score its execution responses, and the extent to which these scores were aligned with human evaluation. Our extraction and execution experiments, underscored the crucial role of human evaluation in assessing the accuracy of responses. An interesting line of exploration in this direction is whether an LLM is able to *evaluate* the outputs of the execution task. Previous work [19, 20] has examined the ability of LLMs to score the outputs of text-to-image models and solutions to STEM textbook questions. [21] entasked GPT-3 to express a verbalized confidence in its answer while solving elementary math problems. In our context, quantifying the ability of an LLM to evaluate its execution of Hartree-Fock computations allows us to examine whether LLMs could potentially be used to supplement human evaluation or correct their own outputs in a highly specialized domain where the bottleneck on experiments is human evaluation. In our case, the evaluator-LLM and the execution-LLM are both GPT-4.

In our experiments, we supply the model with a (`Problem`, `Solution`) tuple where the `Problem` corresponds to the input to the execution step, and the `Solution` corresponds to the language model's (GPT-4's) output for the execution step. The corpus of execution tasks consisted of 160 tasks across 14 papers. While the human evaluation of execution had four criteria in the evaluation rubric, we designate the human-assigned **Correctness** score as the ground-truth target score, since the **Correctness** score required the answer to be exactly correct and penalized the `Solution` for errors in the other three evaluation criteria. The model is instructed to score the responses in a binary fashion: **0** if the response is either partially or completely incorrect, or **1** if the response is correct. Thus, the desired target LM output for all execution tuples with human-assigned **Correctness** scores of 0 and 50 is 0, and for all human-assigned **Correctness** scores of 100, is 1. Two versions of the LM scoring experiment were run. In the first version (Zero-Shot), the model is simply asked to return either 0 or 1 indicating the score. In the second version (Few-Shot with Rationale), the model is instructed to return a dictionary with two keys, `Score`, and `Reason`, and is provided two examples from the corpus.

#### 1. Zero-Shot

**System Prompt:**
You are a condensed matter physicist. You need to score the SOLUTION to a described PROBLEM. Your score must either be 0 or 1.
The correctness of the SOLUTION is crucial. Use the following rubric to score the SOLUTION:
Score 1: The SOLUTION is fully correct.
Score 0: The SOLUTION is fully or partially wrong. The SOLUTION may be partially wrong because of minor errors such as incorrect indices.
Your reply must consist of a single integer indicating the score: 0, or 1.

**User Prompt:**
PROBLEM: `<Input to the Execution Task>`
SOLUTION: `<GPT-4's Output for the Execution Task>`

Of the 160 tasks, 119 (74%) had a ground truth correctness score of 2. Owing to this skewed distribution, computing the accuracy with all tasks receiving the same weight favors a more lenient evaluator, i.e. a model that is more likely to predict 1. We thus report both the accuracy (where all tasks are weighted equally) as well as the class-balanced accuracy in Table IV. The model's accuracy is 78% and its class-balanced accuracy is 69%. Both the accuracy and the class-balanced accuracy for this model are higher than the theoretical expectation for a random predictor, or an evaluator that scores all execution tuples as correct (1).

TABLE IV: Performance of the Zero-Shot LLM Scorer relative to a random predictor and a predictor that scores all solutions as correct on 160 execution responses.

| Metric (%) | Accuracy | Class-Balanced Accuracy | Class-wise Precision [0\|1] | | Class-wise Recall [0\|1] | |
|---|---|---|---|---|---|---|
| Zero-Shot LLM Scorer | **78.12** | **69.31** | **58.33** | **83.87** | **51.22** | **87.39** |
| Random Predictor | 50 | 50 | 25.62 | 74.38 | 50 | 50 |
| Always predicts 1 | 74.38 | 50 | `ill-def.` | 74.38 | 0 | 100 |

### 2. Few (2)-Shot with Rationale

TABLE V: Performance of the Few-Shot with Rationale LLM Scorer relative to the Zero-Shot Scorer, a random predictor or a predictor that scores all solutions as correct on 158 execution responses.

| Metric (%) | Accuracy | Class-Balanced Accuracy | Class-wise Precision [0\|1] | | Class-wise Recall [0\|1] | |
|---|---|---|---|---|---|---|
| Few-Shot with Rationale LLM Scorer | 74.68 | **73.96** | 50 | **89** | **72.5** | 75.42 |
| Zero-Shot LLM Scorer | **78.48** | 69.89 | **58.33** | 84.42 | 52.5 | **87.29** |
| Random Predictor | 50 | 50 | 25.32 | 74.68 | 50 | 50 |
| Always predicts 1 | 74.68 | 50 | `ill-def.` | 74.68 | 0 | 100 |

In this setting, the model is instructed to return a dictionary with 2 keys: `Score` is the same integer score as in the Zero-Shot setting, and the `Reason` is supposed to be the language model's justification for why the execution is incorrect, if it receives a score of 0, and an empty string if the model is scored 1. We additionally supply the model two examples of a target solution, using the human evaluator's comment for the incorrect example. The example for the execution tuple that should be scored incorrectly corresponds to the `Construct Potential Hamiltonian (continuum version)` task for 2308.07488 and that for the correct example corresponds to the `Construct Kinetic Hamiltonian (lattice version)` task for 2308.03843 (see I 2).

We exclude the example problems from our analysis in Table V, resulting in 158 tasks. In this experiment, we find that the model behaves as a stricter evaluator, with a higher recall for the incorrect execution tuples (72% vs 52% in the Zero-Shot setting on 158 tasks), at the cost of incorrectly scoring more correct solutions as incorrect (75% vs 87% recall on correct tuples). The overall accuracy is 75% and the class-balanced accuracy is 74%. Four randomly selected examples of problem-solution tuples that the LLM scored incorrectly are displayed below, along with *"GT Score"*: the ground-truth correctness score, *"GT Score (Reason)"*: the reason from the human evaluator for problems that received a ground-truth score of 0 or 1, and the *"Target Solution"*: the correct answer to the execution task. The *"GT Score"*s of 0/1/2 correspond to 0/50/100 on a scale of 100. The full list of problem-solution tuples that the model designated as incorrect are available at LM-Incorrect.

## 1 arXiv:2112.07523, Define each term in Kinetic Hamiltonian (continuum version)

**SCORE PROMPT**: PROBLEM: You will be instructed to construct each term, namely $h_\uparrow(\boldsymbol{k})$ and $h_\downarrow(\boldsymbol{k})$. For all energy dispersions, $h_\uparrow(\boldsymbol{k})$ and $h_\downarrow(\boldsymbol{k})$, it characterizes the parabolic dispersion for electrons and holes. In addition, a shift of $\boldsymbol{Q}$ in the momentum $\boldsymbol{k}$ for diagonal elements of $h_\uparrow(\boldsymbol{k})$ and $h_\downarrow(\boldsymbol{k})$, respectively. You should follow the EXAMPLE below to obtain correct energy dispersion, select the correct EXAMPLE by noticing the type of dispersion. Finally, in the real space, the momentum $\boldsymbol{k} = -i\partial_{\boldsymbol{r}}$. You should keep the form of $\boldsymbol{k}$ in the Hamiltonian for short notations but should remember $\boldsymbol{k}$ is an operator. You should recall that $H_{\text{BHZ}} = \sum_{\boldsymbol{k}} \psi_{\boldsymbol{k}}^\dagger \begin{pmatrix} h_\uparrow(\boldsymbol{k}) & 0 \\ 0 & h_\downarrow(\boldsymbol{k}) \end{pmatrix} \psi_{\boldsymbol{k}},$ . Return the expression for $h_\uparrow(\boldsymbol{k})$ and $h_\downarrow(\boldsymbol{k})$ in the Kinetic Hamiltonian, and substitute it into the Kinetic Hamiltonian $H_{\text{BHZ}}$. Use the following conventions for the symbols (You should also obey the conventions in all my previous prompts if you encounter undefined symbols. If you find it is never defined or has conflicts in the conventions, you should stop and let me know): $\psi_{\boldsymbol{k}}$: field operators, $c$ and $v$: conduction and valence bands, $\uparrow$ and $\downarrow$: two opposite spins, $h_\uparrow$ and $h_\downarrow$: two $2 \times 2$ matrices, $m_e$ and $m_h$: effective masses of electrons and holes, $E_g$: band gap, $A$: strength of hybridization between the conduction and valence bands, $\boldsymbol{Q}$: momentum shift due to the in-plane magnetic field. ===

EXAMPLE 1: A parabolic dispersion for electron is $E_\alpha = \frac{\hbar^2 k^2}{2m_\alpha}$, where $\alpha$ indicates the type of electron. If there is a further shift of $q$ in the momentum $k$, the dispersion will become $E_\alpha = \frac{\hbar^2 (k-q)^2}{2m_\alpha}$.

EXAMPLE 2: A cos dispersion is $E_\alpha = -\cos(ka/2)$, where $\alpha$ indicates the type of particle. If there is a further shift of $q$ in the momentum $k$, the dispersion will become $E_\alpha = -\cos((k-q)a/2))$. However, there could be more prefactors before cos depending on the geometry of the lattice.

EXAMPLE 3: A dirac dispersion for electron/hole is a 2 by 2 matrix, i.e., $h_\theta(k) = -\hbar v_D |k| \begin{pmatrix} 0 & e^{i(\theta_k - \theta)} \\ e^{-i(\theta_{\bar{k}} - \theta)} & 0 \end{pmatrix}$, where $v_D$ is the Fermi velocity, $\theta$ is the twist angle, and $\theta_k$ indicates the azumith angle of $k$. If there is a further shift of $K_\theta$ in the momentum $k$, the dispersion will become $h_\theta(k) = -\hbar v_D |k - K_\theta| \begin{pmatrix} 0 & e^{i(\theta_{k-K_\theta} - \theta)} \\ e^{-i(\theta_{k-K_\theta} - \theta)} & 0 \end{pmatrix}$.

SOLUTION: Given the parabolic dispersion for electrons and holes, and the shift of $\boldsymbol{Q}$ in the momentum $\boldsymbol{k}$, we can construct the terms $h_\uparrow(\boldsymbol{k})$ and $h_\downarrow(\boldsymbol{k})$ using EXAMPLE 1 and EXAMPLE 2. For $h_\uparrow(\boldsymbol{k})$, we use EXAMPLE 1 for electrons:

$$h_\uparrow(\boldsymbol{k}) = \frac{\hbar^2 (\boldsymbol{k} - \boldsymbol{Q})^2}{2m_e}. \tag{2}$$

For $h_\downarrow(\boldsymbol{k})$, we use EXAMPLE 2 for holes:

$$h_\downarrow(\boldsymbol{k}) = -\frac{\hbar^2 (\boldsymbol{k} - \boldsymbol{Q})^2}{2m_h}. \tag{3}$$

Substituting these into the Kinetic Hamiltonian $H_{\text{BHZ}}$, we get:

$$H_{\text{BHZ}} = \sum_{\boldsymbol{k}} \psi_{\boldsymbol{k}}^\dagger \begin{pmatrix} \frac{\hbar^2 (\boldsymbol{k}-\boldsymbol{Q})^2}{2m_e} & 0 \\ 0 & -\frac{\hbar^2 (\boldsymbol{k}-\boldsymbol{Q})^2}{2m_h} \end{pmatrix} \psi_{\boldsymbol{k}}. \tag{4}$$

SCORE:

**LM Score (Binary)**: 0

**LM Reason**: "The SOLUTION is incorrect. The term $h_\downarrow(\boldsymbol{k})$ should not be negative, and it should also be based on the parabolic dispersion for holes, not the cos dispersion. The correct form should be $h_\downarrow(\boldsymbol{k}) = \frac{\hbar^2 (\boldsymbol{k}-\boldsymbol{Q})^2}{2m_h}$."

**GT Score (0/1/2)**: 0

**GT Reason**: Diagonal terms should have opposite momentum shift.

**Target Solution**:

$$h_\uparrow = \begin{pmatrix} E_g/2 + \frac{(\boldsymbol{k}-\boldsymbol{Q})^2}{2m_e} & A(\boldsymbol{k}) \\ A(\boldsymbol{k}) & -E_g/2 - \frac{(\boldsymbol{k}+\boldsymbol{Q})^2}{2m_h} \end{pmatrix} \tag{5}$$

and

$$h_\downarrow = \begin{pmatrix} E_g/2 + \frac{(\boldsymbol{k}-\boldsymbol{Q})^2}{2m_e} & -A(\boldsymbol{k}) \\ -A(\boldsymbol{k}) & -E_g/2 - \frac{(\boldsymbol{k}+\boldsymbol{Q})^2}{2m_h} \end{pmatrix} \tag{6}$$

## 2 arXiv:1106.6060, Swap the index only

**SCORE PROMPT**: PROBLEM: You will be instructed to simplify the quadratic term $\hat{H}^{int,Hartree}$ through relabeling the index. The logic is that the expected value $(\langle c_{\alpha_1,s_1}^\dagger(k_1) c_{\alpha_1,s_1}(k_2) \rangle)$ in the first Hartree term

$(\langle c^\dagger_{\alpha_1,s_1}(k_1)c_{\alpha_1,s_1}(k_2)\rangle c^\dagger_{\alpha_2,s_2}(k_3)c_{\alpha_2,s_2}(k_4))$ has the same form as the quadratic operators in the second Hartree term $(\langle c^\dagger_{\alpha_2,s_2}(k_3)c_{\alpha_2,s_2}(k_4)\rangle c^\dagger_{\alpha_1,s_1}(k_1)c_{\alpha_1,s_1}(k_2))$, and vice versa. The same applies to the Fock term. Namely, a replacement of $k_1 \leftrightarrow k_3$ and $k_2 \leftrightarrow k_4$ is applied to ONLY the second Hartree or Fock term. You should not swap any index that is not in the summation, which includes spin index. This means, if you relabel the index by swapping the index in the "expected value" and "quadratic operators" in the second Hartree or Fock term, you can make the second Hartree or Fock term look identical to the first Hartree or Fock term, as long as $V(q) = V(-q)$, which is naturally satisfied in Coulomb interaction. You should follow the EXAMPLE below to simplify it through relabeling the index. You should recall that $\hat{H}^{int,Hartree}$ is $\frac{U_d}{N}\sum_{k_1,k_2,k_3,k_4}\sum_G \delta(k_1-k_2+k_3-k_4,G)\Big[\langle c^\dagger_{d,\uparrow}(k_1)c_{d,\uparrow}(k_2)\rangle c^\dagger_{d,\downarrow}(k_3)c_{d,\downarrow}(k_4) + \langle c^\dagger_{d,\downarrow}(k_3)c_{d,\downarrow}(k_4)\rangle c^\dagger_{d,\uparrow}(k_1)c_{d,\uparrow}(k_2)\Big]$ $+\frac{U_p}{2N}\sum_{k_1,k_2,k_3,k_4}\sum_G\delta(k_1-k_2+k_3-k_4,G)\Big\{\langle c^\dagger_{p_x,\uparrow}(k_1)c_{p_x,\uparrow}(k_2)\rangle c^\dagger_{p_x,\downarrow}(k_3)c_{p_x,\downarrow}(k_4) + \langle c^\dagger_{p_x,\downarrow}(k_3)c_{p_x,\downarrow}(k_4)\rangle c^\dagger_{p_x,\uparrow}(k_1)c_{p_x,\uparrow}(k_2) + \langle c^\dagger_{p_y,\uparrow}(k_1)c_{p_y,\uparrow}(k_2)\rangle c^\dagger_{p_y,\downarrow}(k_3)c_{p_y,\downarrow}(k_4) + \langle c^\dagger_{p_y,\downarrow}(k_3)c_{p_y,\downarrow}(k_4)\rangle c^\dagger_{p_y,\uparrow}(k_1)c_{p_y,\uparrow}(k_2)\Big\} + 2V_{pd}\sum_{s,s'}\frac{1}{N}\sum_{k_1,k_2,k_3,k_4}\sum_G\delta(k_1-k_2+k_3-k_4,G)\Big[\langle c^\dagger_{d,s}(k_1)c_{d,s}(k_2)\rangle c^\dagger_{p_x,s'}(k_3)c_{p_x,s'}(k_4)\cos\left(\frac{k_3-k_4}{2}\cdot\hat{x}\right) + \langle c^\dagger_{p_x,s'}(k_3)c_{p_x,s'}(k_4)\rangle c^\dagger_{d,s}(k_1)c_{d,s}(k_2)\cos\left(\frac{k_3-k_4}{2}\cdot\hat{x}\right) + \langle c^\dagger_{d,s}(k_1)c_{d,s}(k_2)\rangle c^\dagger_{p_y,s'}(k_3)c_{p_y,s'}(k_4)\cos\left(\frac{k_3-k_4}{2}\cdot\hat{y}\right) + \langle c^\dagger_{p_y,s'}(k_3)c_{p_y,s'}(k_4)\rangle c^\dagger_{d,s}(k_1)c_{d,s}(k_2)\cos\left(\frac{k_3-k_4}{2}\cdot\hat{y}\right)\Big] + 2V_{pd}\sum_{s,s'}\frac{1}{N}\sum_{k_1,k_2,k_3,k_4}\sum_G\delta(k_1-k_2+k_3-k_4,G)\Big[\langle c^\dagger_{d,s}(k_1)c_{d,s}(k_2)\rangle c^\dagger_{p_x,s'}(k_3)c_{p_x,s'}(k_4)\cos\left(\frac{k_3-k_4}{2}\cdot\hat{x}\right) + \langle c^\dagger_{p_x,s'}(k_3)c_{p_x,s'}(k_4)\rangle c^\dagger_{d,s}(k_1)c_{d,s}(k_2)\cos\left(\frac{k_3-k_4}{2}\cdot\hat{x}\right) + \langle c^\dagger_{d,s}(k_1)c_{d,s}(k_2)\rangle c^\dagger_{p_y,s'}(k_3)c_{p_y,s'}(k_4)\cos\left(\frac{k_3-k_4}{2}\cdot\hat{y}\right) + \langle c^\dagger_{p_y,s'}(k_3)c_{p_y,s'}(k_4)\rangle c^\dagger_{d,s}(k_1)c_{d,s}(k_2)\cos\left(\frac{k_3-k_4}{2}\cdot\hat{y}\right)\Big] + \frac{V_{pp}}{N}\sum_{s,s'}\sum_{\sigma_x,\sigma_y}\sum_{k_1,k_2,k_3,k_4}\sum_G\delta(k_2-k_1+k_4-k_3,G)e^{-i(k_1-k_2)\cdot\sigma_x\hat{x}/2-i(k_3-k_4)\cdot\sigma_y\hat{y}/2}\times\Big[\langle c^\dagger_{p_x,s}(k_1)c_{p_x,s}(k_2)\rangle c^\dagger_{p_y,s'}(k_3)c_{p_y,s'}(k_4) + \langle c^\dagger_{p_y,s'}(k_3)c_{p_y,s'}(k_4)\rangle c^\dagger_{p_x,s}(k_1)c_{p_x,s}(k_2)\Big]$ Return the simplified $\hat{H}^{int,Hartree}$. ===

EXAMPLE: Given a Hamiltonian $\hat{H} = \sum_{k_1,k_2,k_3,k_4,\sigma_1,\sigma_2,\sigma_3,\sigma_4} V(k_1-k_4)(\langle c^\dagger_{d,\sigma_1}(k_1)c_{d,\sigma_4}(k_4)\rangle c^\dagger_{p,\sigma_2}(k_2)c_{p,\sigma_3}(k_3) + \langle c^\dagger_{p,\sigma_2}(k_2)c_{d,\sigma_3}(k_3)\rangle c^\dagger_{d,\sigma_1}(k_1)c_{\sigma_4}(k_4))\delta_{k_1+k_2,k_3+k_4}$, where $V(q)=V(-q)$. In the second term, we relabel the index to swap the index in expected value and the index in quadratic operators, namely, $\sigma_1 \leftrightarrow \sigma_2$, $\sigma_3 \leftrightarrow \sigma_4$, $k_1 \leftrightarrow k_2$, $k_3 \leftrightarrow k_4$. Important: $d$ and $p$ cannot be swapped because they are not indices in the summation. After the replacement, the second term becomes $\sum_{k_1,k_2,k_3,k_4,\sigma_1,\sigma_2,\sigma_3,\sigma_4} V(k_2-k_3)\langle c^\dagger_{p,\sigma_1}(k_1)c_{p,\sigma_4}(k_4)\rangle c^\dagger_{d,\sigma_2}(k_2)c_{d,\sigma_3}(k_3)\delta_{k_4+k_3,k_2+k_1}$. Note that the Kronecker dirac function $\delta_{k_4+k_3,k_2+k_1}$ implies $k_1+k_2=k_3+k_4$, i.e., $k_2-k_3=k_4-k_1$. Thus, the second term simplifies to $\sum_{k_1,k_2,k_3,k_4,\sigma_1,\sigma_2,\sigma_3,\sigma_4} V(k_4-k_1)\langle c^\dagger_{p,\sigma_1}(k_1)c_{p,\sigma_4}(k_4)\rangle c^\dagger_{d,\sigma_2}(k_2)c_{d,\sigma_3}(k_3)\delta_{k_4+k_3,k_2+k_1}$. Because $V(q)=V(-q)$, meaning $V(k_4-k_1)=V(k_1-k_4)$, the second term further simplifies to $\sum_{k_1,k_2,k_3,k_4,\sigma_1,\sigma_2,\sigma_3,\sigma_4} V(k_1-k_4)\langle c^\dagger_{p,\sigma_1}(k_1)c_{p,\sigma_4}(k_4)\rangle c^\dagger_{d,\sigma_2}(k_2)c_{d,\sigma_3}(k_3)\delta_{k_4+k_3,k_2+k_1}$. Finally, we have the simplified Hamiltonian as $\hat{H} = \sum_{k_1,k_2,k_3,k_4,\sigma_1,\sigma_2,\sigma_3,\sigma_4} V(k_1-k_4)(\langle c^\dagger_{d,\sigma_1}(k_1)c_{d,\sigma_4}(k_4)\rangle c^\dagger_{p,\sigma_2}(k_2)c_{p,\sigma_3}(k_3) + \langle c^\dagger_{p,\sigma_1}(k_1)c_{p,\sigma_4}(k_4)\rangle c^\dagger_{d,\sigma_2}(k_2)c_{d,\sigma_3}(k_3))\delta_{k_4+k_3,k_2+k_1}$.

SOLUTION: Following the example, we can simplify $\hat{H}^{int,Hartree}$ by relabeling the indices in the second Hartree term of each interaction. The relabeling swaps the indices in the expectation value and the quadratic operators, namely, $k_1 \leftrightarrow k_3$, $k_2 \leftrightarrow k_4$. After the replacement, the simplified $\hat{H}^{int,Hartree}$ is: $\hat{H}^{int,Hartree} = \frac{U_d}{N}\sum_{k_1,k_2,k_3,k_4}\sum_G\delta(k_1-k_2+k_3-k_4,G)\Big[\langle c^\dagger_{d,\uparrow}(k_1)c_{d,\uparrow}(k_2)\rangle c^\dagger_{d,\downarrow}(k_3)c_{d,\downarrow}(k_4) + \langle c^\dagger_{d,\uparrow}(k_1)c_{d,\uparrow}(k_2)\rangle c^\dagger_{d,\downarrow}(k_3)c_{d,\downarrow}(k_4)\Big]$ $+\frac{U_p}{2N}\sum_{k_1,k_2,k_3,k_4}\sum_G\delta(k_1-k_2+k_3-k_4,G)\Big\{\langle c^\dagger_{p_x,\uparrow}(k_1)c_{p_x,\uparrow}(k_2)\rangle c^\dagger_{p_x,\downarrow}(k_3)c_{p_x,\downarrow}(k_4) + \langle c^\dagger_{p_x,\uparrow}(k_1)c_{p_x,\uparrow}(k_2)\rangle c^\dagger_{p_x,\downarrow}(k_3)c_{p_x,\downarrow}(k_4) + \langle c^\dagger_{p_y,\uparrow}(k_1)c_{p_y,\uparrow}(k_2)\rangle c^\dagger_{p_y,\downarrow}(k_3)c_{p_y,\downarrow}(k_4) + \langle c^\dagger_{p_y,\uparrow}(k_1)c_{p_y,\uparrow}(k_2)\rangle c^\dagger_{p_y,\downarrow}(k_3)c_{p_y,\downarrow}(k_4)\Big\} + 2V_{pd}\sum_{s,s'}\frac{1}{N}\sum_{k_1,k_2,k_3,k_4}\sum_G\delta(k_1-k_2+k_3-k_4,G)\Big[\langle c^\dagger_{d,s}(k_1)c_{d,s}(k_2)\rangle c^\dagger_{p_x,s'}(k_3)c_{p_x,s'}(k_4)\cos\left(\frac{k_3-k_4}{2}\cdot\hat{x}\right) + \langle c^\dagger_{d,s}(k_1)c_{d,s}(k_2)\rangle c^\dagger_{p_x,s'}(k_3)c_{p_x,s'}(k_4)\cos\left(\frac{k_3-k_4}{2}\cdot\hat{x}\right) + \langle c^\dagger_{d,s}(k_1)c_{d,s}(k_2)\rangle c^\dagger_{p_y,s'}(k_3)c_{p_y,s'}(k_4)\cos\left(\frac{k_3-k_4}{2}\cdot\hat{y}\right) + \langle c^\dagger_{d,s}(k_1)c_{d,s}(k_2)\rangle c^\dagger_{p_y,s'}(k_3)c_{p_y,s'}(k_4)\cos\left(\frac{k_3-k_4}{2}\cdot\hat{y}\right)\Big]$ $+2V_{pd}\sum_{s,s'}\frac{1}{N}\sum_{k_1,k_2,k_3,k_4}\sum_G\delta(k_1-k_2+k_3-k_4,G)\Big[\langle c^\dagger_{d,s}(k_1)c_{d,s}(k_2)\rangle c^\dagger_{p_x,s'}(k_3)c_{p_x,s'}(k_4)\cos\left(\frac{k_3-k_4}{2}\cdot\hat{x}\right) + \langle c^\dagger_{d,s}(k_1)c_{d,s}(k_2)\rangle c^\dagger_{p_x,s'}(k_3)c_{p_x,s'}(k_4)\cos\left(\frac{k_3-k_4}{2}\cdot\hat{x}\right) + \langle c^\dagger_{d,s}(k_1)c_{d,s}(k_2)\rangle c^\dagger_{p_y,s'}(k_3)c_{p_y,s'}(k_4)\cos\left(\frac{k_3-k_4}{2}\cdot\hat{y}\right) + \langle c^\dagger_{d,s}(k_1)c_{d,s}(k_2)\rangle c^\dagger_{p_y,s'}(k_3)c_{p_y,s'}(k_4)\cos\left(\frac{k_3-k_4}{2}\cdot\hat{y}\right)\Big] + \frac{V_{pp}}{N}\sum_{s,s'}\sum_{\sigma_x,\sigma_y}\sum_{k_1,k_2,k_3,k_4}\sum_G\delta(k_2-k_1+k_4-k_3,G)e^{-i(k_1-k_2)\cdot\sigma_x\hat{x}/2-i(k_3-k_4)\cdot\sigma_y\hat{y}/2}\times\Big[\langle c^\dagger_{p_x,s}(k_1)c_{p_x,s}(k_2)\rangle c^\dagger_{p_y,s'}(k_3)c_{p_y,s'}(k_4) + \langle c^\dagger_{p_x,s}(k_1)c_{p_x,s}(k_2)\rangle c^\dagger_{p_y,s'}(k_3)c_{p_y,s'}(k_4)\Big]$ This is the simplified $\hat{H}^{int,Hartree}$ after relabeling the indices.

SCORE:

**LM Score (Binary)**: 0

**LM Reason**: "The SOLUTION does not correctly apply the index swapping to the second Hartree term of each interaction. The indices $k_1 \leftrightarrow k_3$ and $k_2 \leftrightarrow k_4$ should be swapped in the second Hartree term, but the solution does not reflect this change. The solution is identical to the original problem statement, indicating that the index swapping has not been applied."

**GT Score (0/1/2)**: 1

**GT Reason**: In Paper: not directly in plain format, it's in the matrix format. up and down shouldn't swap in the term

with U˙d.

**Target Solution**: $\frac{U_d}{N}\sum_{k_1,k_2,k_3,k_4}\sum_G \delta(k_1-k_2+k_3-k_4,G)\Big[\langle c^\dagger_{d,\uparrow}(k_1)c_{d,\uparrow}(k_2)\rangle c^\dagger_{d,\downarrow}(k_3)c_{d,\downarrow}(k_4)+\langle c^\dagger_{d,\downarrow}(k_1)c_{d,\downarrow}(k_2)\rangle c^\dagger_{d,\uparrow}(k_3)c_{d,\uparrow}(k_4)\Big]+\frac{U_p}{2N}\sum_{k_1,k_2,k_3,k_4}\sum_G \delta(k_1-k_2+k_3-k_4,G)\Big\{\langle c^\dagger_{p_x,\uparrow}(k_1)c_{p_x,\uparrow}(k_2)\rangle c^\dagger_{p_x,\downarrow}(k_3)c_{p_x,\downarrow}(k_4)+\langle c^\dagger_{p_x,\downarrow}(k_1)c_{p_x,\downarrow}(k_2)\rangle c^\dagger_{p_x,\uparrow}(k_3)c_{p_x,\uparrow}(k_4)+\langle c^\dagger_{p_y,\uparrow}(k_1)c_{p_y,\uparrow}(k_2)\rangle c^\dagger_{p_y,\downarrow}(k_3)c_{p_y,\downarrow}(k_4)+\langle c^\dagger_{p_y,\downarrow}(k_1)c_{p_y,\downarrow}(k_2)\rangle c^\dagger_{p_y,\uparrow}(k_3)c_{p_y,\uparrow}(k_4)\Big\}+2V_{pd}\sum_{s,s'}\frac{1}{N}\sum_{k_1,k_2,k_3,k_4}\sum_G \delta(k_1-k_2+k_3-k_4,G)\Big[\langle c^\dagger_{d,s}(k_1)c_{d,s}(k_2)\rangle c^\dagger_{p_x,s'}(k_3)c_{p_x,s'}(k_4)\cos\left(\frac{k_3-k_4}{2}\cdot\hat{x}\right)+\langle c^\dagger_{p_x,s}(k_1)c_{p_x,s}(k_2)\rangle c^\dagger_{d,s'}(k_3)c_{d,s'}(k_4)\cos\left(\frac{k_1-k_2}{2}\cdot\hat{x}\right)+\langle c^\dagger_{d,s}(k_1)c_{d,s}(k_2)\rangle c^\dagger_{p_y,s'}(k_3)c_{p_y,s'}(k_4)\cos\left(\frac{k_3-k_4}{2}\cdot\hat{y}\right)+\langle c^\dagger_{p_y,s}(k_1)c_{p_y,s}(k_2)\rangle c^\dagger_{d,s'}(k_3)c_{d,s'}(k_4)\cos\left(\frac{k_1-k_2}{2}\cdot\hat{y}\right)\Big]+\frac{V_{pp}}{N}\sum_{s,s'}\sum_{\sigma_x,\sigma_y}\sum_{k_1,k_2,k_3,k_4}\sum_G \delta(k_2-k_1+k_4-k_3,G)e^{-i(k_1-k_2)\cdot\sigma_x\hat{x}/2-i(k_3-k_4)\cdot\sigma_y\hat{y}/2}\times\Big[\langle c^\dagger_{p_x,s}(k_1)c_{p_x,s}(k_2)\rangle c^\dagger_{p_y,s'}(k_3)c_{p_y,s'}(k_4)+\langle c^\dagger_{p_y,s}(k_1)c_{p_y,s}(k_2)\rangle c^\dagger_{p_x,s'}(k_3)c_{p_x,s'}(k_4)\Big]$

## 3 arXiv:2108.02159, Extract quadratic term

**SCORE PROMPT**: PROBLEM: You will be instructed to extract the quadratic terms in the $\Sigma^{HF}$. The quadratic terms mean terms that are proportional to $\rho_{\alpha,\boldsymbol{b};\beta,\boldsymbol{b}'}$, which excludes terms that are solely expectations or products of expectations. You should only preserve the quadratic terms in $\Sigma^{HF}$, denoted as $\Sigma^{HF}_{\alpha,\boldsymbol{b};\beta,\boldsymbol{b}'}$. You should recall that $\Sigma^{int,HF}=\frac{1}{2NA}\sum_{\sigma_1,\sigma_2,b_1,b_2,b_3,b_4,k_1,k_2,k_3,k_4}V(q)\delta_{k_1+b_1+k_2+b_2,k_3+b_3+k_4+b_4}[\langle c^\dagger_{\sigma_1,b_1}(k_1)c_{\sigma_1,b_4}(k_4)\rangle c^\dagger_{\sigma_2,b_2}(k_2)c_{\sigma_2,b_3}(k_3)+\langle c^\dagger_{\sigma_2,b_2}(k_2)c_{\sigma_2,b_3}(k_3)\rangle c^\dagger_{\sigma_1,b_1}(k_1)c_{\sigma_1,b_4}(k_4)-\langle c^\dagger_{\sigma_1,b_1}(k_1)c_{\sigma_1,b_4}(k_4)\rangle\langle c^\dagger_{\sigma_2,b_2}(k_2)c_{\sigma_2,b_3}(k_3)\rangle-\langle c^\dagger_{\sigma_1,b_1}(k_1)c_{\sigma_2,b_3}(k_3)\rangle c^\dagger_{\sigma_2,b_2}(k_2)c_{\sigma_1,b_4}(k_4)-\langle c^\dagger_{\sigma_2,b_2}(k_2)c_{\sigma_1,b_4}(k_4)\rangle c^\dagger_{\sigma_1,b_1}(k_1)c_{\sigma_2,b_3}(k_3)+\langle c^\dagger_{\sigma_1,b_1}(k_1)c_{\sigma_2,b_3}(k_3)\rangle\langle c^\dagger_{\sigma_2,b_2}(k_2)c_{\sigma_1,b_4}(k_4)\rangle]$. Return $\Sigma^{HF}_{\alpha,\boldsymbol{b};\beta,\boldsymbol{b}'}$. Use the following conventions for the symbols (You should also obey the conventions in all my previous prompts if you encounter undefined symbols. If you find it is never defined or has conflicts in the conventions, you should stop and let me know): In $\Sigma^{HF}_{\alpha,\boldsymbol{b};\beta,\boldsymbol{b}'}$, Greek letters label spin, $A$ is the finite sample area corresponding to a discrete Brillouin-zone mesh, and $\rho_{\alpha,\boldsymbol{b};\beta,\boldsymbol{b}'}$ is the self-consistently determined momentum-space density matrix.

SOLUTION: The quadratic terms in $\Sigma^{HF}$ are those that are proportional to $\rho_{\alpha,\boldsymbol{b};\beta,\boldsymbol{b}'}$. From the given expression for $\Sigma^{int,HF}$, we can identify these terms as: $\Sigma^{HF}_{\alpha,\boldsymbol{b};\beta,\boldsymbol{b}'}=\frac{1}{2NA}\sum_{\sigma_1,\sigma_2,b_1,b_2,b_3,b_4,k_1,k_2,k_3,k_4}V(q)\delta_{k_1+b_1+k_2+b_2,k_3+b_3+k_4+b_4}[\langle c^\dagger_{\sigma_1,b_1}(k_1)c_{\sigma_1,b_4}(k_4)\rangle c^\dagger_{\sigma_2,b_2}(k_2)c_{\sigma_2,b_3}(k_3)+\langle c^\dagger_{\sigma_2,b_2}(k_2)c_{\sigma_2,b_3}(k_3)\rangle c^\dagger_{\sigma_1,b_1}(k_1)c_{\sigma_1,b_4}(k_4)-\langle c^\dagger_{\sigma_1,b_1}(k_1)c_{\sigma_2,b_3}(k_3)\rangle c^\dagger_{\sigma_2,b_2}(k_2)c_{\sigma_1,b_4}(k_4)-\langle c^\dagger_{\sigma_2,b_2}(k_2)c_{\sigma_1,b_4}(k_4)\rangle c^\dagger_{\sigma_1,b_1}(k_1)c_{\sigma_2,b_3}(k_3)]$ This expression represents the quadratic terms in the Hartree-Fock self-energy, $\Sigma^{HF}_{\alpha,\boldsymbol{b};\beta,\boldsymbol{b}'}$, after the interaction term has been expanded using the Hartree-Fock approximation.

SCORE:

**LM Score (Binary)**: 0

**LM Reason**: "The SOLUTION is incorrect. The quadratic terms in the Hartree-Fock self-energy should not include terms that are solely expectations or products of expectations. The solution includes such terms, which is not in accordance with the problem statement."

**GT Score (0/1/2)**: 2

**GT Reason**: N/A

**Target Solution**: $\hat{H}^{int,HF,2}=\frac{1}{2NA}\sum_{\sigma_1,\sigma_2,b_1,b_2,b_3,b_4,k_1,k_2,k_3,k_4}V(q)\delta_{k_1+b_1+k_2+b_2,k_3+b_3+k_4+b_4}[\langle c^\dagger_{\sigma_1,b_1}(k_1)c_{\sigma_1,b_4}(k_4)\rangle c^\dagger_{\sigma_2,b_2}(k_2)c_{\sigma_2,b_3}(k_3)$ $\langle c^\dagger_{\sigma_2,b_2}(k_2)c_{\sigma_2,b_3}(k_3)\rangle c^\dagger_{\sigma_1,b_1}(k_1)c_{\sigma_1,b_4}(k_4)-\langle c^\dagger_{\sigma_1,b_1}(k_1)c_{\sigma_2,b_3}(k_3)\rangle c^\dagger_{\sigma_2,b_2}(k_2)c_{\sigma_1,b_4}(k_4)-\langle c^\dagger_{\sigma_2,b_2}(k_2)c_{\sigma_1,b_4}(k_4)\rangle c^\dagger_{\sigma_1,b_1}(k_1)c_{\sigma_2,b_3}(k_3)]$

## 4 arXiv:2111.01152, Construct Kinetic Hamiltonian (continuum version, single-particle)

**SCORE PROMPT**: PROBLEM: You will be instructed to describe the kinetic term of Hamiltonian in a system with two layers in the real space in the single-particle form. The degrees of freedom of the system are: valley index (+K and -K valley), layer index (top and bottom layer).. Express the Kinetic Hamiltonian $H_\tau$ using variables which are only on the diagonal terms, and arrange the basis in the order of (+K,bottom), (+K,top), (-K,bottom), (-K,top). Use the following conventions for the symbols: $\tau=\pm1$ represents $\pm K$ valleys, $\boldsymbol{\kappa}=\frac{4\pi}{3a_M}(1,0)$ is at a corner of the moiré Brillouin zone. The $2\times2$ Hamiltonian hybridizes the bottom layer ($\mathfrak{b}$) and top layer ($\mathfrak{t}$), where the off diagonal terms describe the interlayer tunneling $\Delta_{\mathrm{T},\tau}$, and the diagonal terms describe the momentum-shifted kinetic energy with the effective mass $(m_{\mathfrak{b}},m_{\mathfrak{t}})=(0.65,0.35)m_e$ ($m_e$ is the rest electron mass), plus the intralayer potential $\Delta_{\mathfrak{b}/\mathfrak{t}}$, and a band offset $V_{z\mathfrak{t}}$.

SOLUTION: The kinetic term of the Hamiltonian in a system with two layers in the real space in the single-particle form can be written as:

$$H_\tau=\begin{pmatrix}\frac{(\hbar k-\tau\hbar\boldsymbol{\kappa})^2}{2m_{\mathfrak{b}}}+\Delta_{\mathfrak{b}} & 0\\ 0 & \frac{(\hbar k-\tau\hbar\boldsymbol{\kappa})^2}{2m_{\mathfrak{t}}}+\Delta_{\mathfrak{t}}+V_{z\mathfrak{t}}\end{pmatrix} \quad (7)$$

where $\tau$ represents the valley index (+K and -K valley), $\boldsymbol{\kappa}$ is at a corner of the moiré Brillouin zone, $m_{\mathfrak{b}}$ and $m_{\mathfrak{t}}$ are the effective masses of the bottom and top layers respectively, $\Delta_{\mathfrak{b}}$ and $\Delta_{\mathfrak{t}}$ are the intralayer potentials, and $V_{z\mathfrak{t}}$ is the band offset. The basis is arranged in the order of (+K,bottom), (+K,top), (-K,bottom), (-K,top). The Hamiltonian is diagonal, meaning there is no interlayer tunneling.

SCORE:

**LM Score (Binary)**: 0

**LM Reason**: "The SOLUTION is incorrect. The Hamiltonian matrix provided does not match the required 4x4 matrix for the four degrees of freedom: (+K,bottom), (+K,top), (-K,bottom), (-K,top). The solution only provides a 2x2 matrix."

**GT Score (0/1/2)**: 1

**GT Reason**: bottom layer does not have a shift of Kappa, but this may be also due to the unclear instruction (so 1 point drop for `prompt_quality`)

**Target Solution**: $H_{Kinetic}(r) = \begin{pmatrix} E_{+K,b} & 0 & 0 & 0 \\ 0 & E_{+K,t} & 0 & 0 \\ 0 & 0 & E_{-K,b} & 0 \\ 0 & 0 & 0 & E_{-K,t} \end{pmatrix}$

**System Prompt:**
You are a condensed matter physicist. You need to score the SOLUTION to a described PROBLEM. Your score must either be 0 or 1.
The correctness of the SOLUTION is crucial. Use the following rubric to score the SOLUTION:
Score 1: The SOLUTION is fully correct.
Score 0: The SOLUTION is fully or partially wrong. The SOLUTION may be partially wrong because of minor errors such as incorrect indices.
Your reply must consist of a JSON-parsable dictionary with two keys:
Score: A single integer that is either 0 or 1.
Reason: Your justification for the score. This should be an empty string if the score is 1, or the errors in the solution, if the score is 0.
Use the following examples to learn how to assign scores:
===
EXAMPLE #0:
PROBLEM: You will be instructed to describe the potential term of Hamiltonian $H_P$ in the real space in the single-particle form. The potential Hamiltonian has the same degrees of freedom as the kinetic Hamiltonian. The diagonal terms are $\Delta_b(\boldsymbol{r})$ and $\Delta_t(\boldsymbol{r})$. The off-diagonal terms are the coupling between layer index $l$ and valley index $\tau$, $\Delta_T(\boldsymbol{r})$ and $\Delta_T^\dagger(\boldsymbol{r})$, which should be kept hermitian. All others terms are zero. Express the potential Hamiltonian $H_P$ using $\Delta_b(\boldsymbol{r})$ and $\Delta_t(\boldsymbol{r})$ and $\Delta_T(\boldsymbol{r})$ and $\Delta_T^\dagger(\boldsymbol{r})$. Use the following conventions for the symbols (You should also obey the conventions in all my previous prompts if you encounter undefined symbols. If you find it is never defined or has conflicts in the conventions, you should stop and let me know): The intralayer and interlayer moiré potentials are $\Delta_{b/t} = 2V\sum_{i=1,3,5}\cos(\boldsymbol{G}_i\cdot\boldsymbol{r}\pm\phi)$ and $\Delta_T = w(1+e^{-i\boldsymbol{G}_2\cdot\boldsymbol{r}}+e^{-i\boldsymbol{G}_3\cdot\boldsymbol{r}})$, respectively. $\boldsymbol{G}_i = \frac{4\pi}{\sqrt{3}a_M}(\cos\frac{i-1}{3}\pi, \sin\frac{i-1}{3}\pi)$ are moiré reciprocal lattice vectors with $a_M$ being the moiré lattice constant. $\boldsymbol{\kappa}_+ = 2\boldsymbol{G}_1/3 - \boldsymbol{G}_2/3$ and $\boldsymbol{\kappa}_- = \boldsymbol{G}_1/3 + \boldsymbol{G}_2/3$ are the mBZ corners. $m^*$ is the effective mass and is taken as $0.6m_e$, where $m_e$ is the free electron mass. Layer-differentiating potential proportional to $\Delta_D$ is included in $H_K$ to take into account the out-of-plane electric field. For $K'$ valley, the continuum model Hamiltonian can be deduced by acting time reversal operator on $H_K$.
SOLUTION: The potential Hamiltonian $H_P$ in the real space in the single-particle form, given the conventions and the instructions, can be written as:

$$H_P = \begin{pmatrix} \Delta_b(\boldsymbol{r}) & 0 & 0 & \Delta_T(\boldsymbol{r}) \\ 0 & \Delta_t(\boldsymbol{r}) & \Delta_T^\dagger(\boldsymbol{r}) & 0 \\ 0 & \Delta_T(\boldsymbol{r}) & \Delta_b(\boldsymbol{r}) & 0 \\ \Delta_T^\dagger(\boldsymbol{r}) & 0 & 0 & \Delta_t(\boldsymbol{r}) \end{pmatrix}$$

Here, $\Delta_b(\boldsymbol{r})$ and $\Delta_t(\boldsymbol{r})$ are the diagonal terms representing the intralayer moiré potentials for the bottom and top layers, respectively. $\Delta_T(\boldsymbol{r})$ and $\Delta_T^\dagger(\boldsymbol{r})$ are the off-diagonal terms representing the interlayer moiré potentials, ensuring the hermiticity of the Hamiltonian. All other terms are zero, as per the instructions.
SCORE: {"Score": 0, "Reason": "The SOLUTION does not arrange the matrix elements in the required order."}
===
EXAMPLE #1:
PROBLEM: You will be instructed to describe the kinetic term of Hamiltonian in TBG in the real space in the second-quantized form. The degrees of freedom of the system are: spin and sublattice The kinetic term is a tight-binding model composed of the following hopping process: site i and site j with the amplitude $h_{\alpha\beta}(R_i - R_j)$ The summation should be taken over all spin and sublattice and all real space positions. Return the Kinetic Hamiltonian $H_0$. Use the following conventions for the symbols: $d_{\alpha,i,\sigma}$ is the annihilation operator of an electron with spin $\sigma$=↑,↓ on sublattice $\alpha$ of unit cell i, and $h_{\alpha\beta}(R_i - R_j)$ is the corresponding tight-binding matrix element between sublattices $\alpha$ and $\beta$ located in unit cells centered at $R_i$ and $R_j$ respectively.
SOLUTION: The kinetic term of the Hamiltonian in the second-quantized form can be written as: $H_0 = \sum_{i,j}\sum_{\alpha,\beta}\sum_\sigma h_{\alpha\beta}(R_i - R_j) d^\dagger_{\alpha,i,\sigma} d_{\beta,j,\sigma}$ Here, the first sum is over all unit cells i and j, the second sum is over all sublattices $\alpha$ and $\beta$, and the third sum is over all spin states $\sigma$. The operator $d^\dagger_{\alpha,i,\sigma}$ creates an electron with spin $\sigma$ on sublattice $\alpha$ of unit cell i, and $d_{\beta,j,\sigma}$ annihilates an electron with spin $\sigma$ on sublattice $\beta$ of unit cell j. The matrix element $h_{\alpha\beta}(R_i - R_j)$ represents the hopping amplitude between these sites.
SCORE: {"Score": 1, "Reason": ""}
===
Now score the following problem and solution:

[1] Pan, H., Xie, M., Wu, F. & Das Sarma, S. Topological phases in ab-stacked mote$_2$/wse$_2$: $F_2$ topological insulators, chern insulators, and topological charge density waves. *Physical Review Letters* **129**, 056804 (2022). 2111.01152.

[2] arxiv dataset. URL `https://www.kaggle.com/datasets/Cornell-University/arxiv`.

[3] Jung, J., Zhang, F. & MacDonald, A. H. Lattice theory of pseudospin ferromagnetism in bilayer graphene: Competing interaction-induced quantum Hall states. *Physical Review B* **83**, 115408 (2011). 1010.1819.

[4] Fischer, M. H. & Kim, E.-A. Mean-Field Analysis of Intra-Unit-Cell Order in the Emery Model of the CuO$_2$ Plane. *Physical Review B* **84**, 144502 (2011). 1106.6060.

[5] Jung, J. & MacDonald, A. H. Gapped broken symmetry states in ABC trilayer graphene. *Physical Review B* **88**, 075408 (2013). 1208.0116.

[6] Johnston, S., Mukherjee, A., Elfimov, I., Berciu, M. & Sawatzky, G. A. Charge disproportionation without charge transfer in the rare-earth nickelates as a possible mechanism for the metal-insulator transition. *Physical Review Letters* **112**, 106404 (2014). 1310.2674.

[7] Naka, M., Seo, H. & Motome, Y. Theory of Valence Transition in BiNiO$_3$. *Physical Review Letters* **116**, 056402 (2016). 1508.00296.

[8] Xie, M. & MacDonald, A. H. On the nature of the correlated insulator states in twisted bilayer graphene. *Physical Review Letters* **124**, 097601 (2020). 1812.04213.

[9] Pan, H., Wu, F. & Das Sarma, S. Band topology, Hubbard model, Heisenberg model, and Dzyaloshinskii-Moriya interaction in twisted bilayer ${\mathrm{WSe}}_{2}$. *Physical Review Research* **2**, 033087 (2020). 2004.04168.

[10] Pan, H., Wu, F. & Das Sarma, S. Quantum phase diagram of a Moiré-Hubbard model. *Physical Review B* **102**, 201104 (2020). 2008.08998.

[11] Pan, H. & Das Sarma, S. Interaction-Driven Filling-Induced Metal-Insulator Transitions in 2D Moiré Lattices. *Physical Review Letters* **127**, 096802 (2021). 2012.04554.

[12] Hu, N. C. & MacDonald, A. H. Competing magnetic states in transition metal dichalcogenide moir\'e materials. *Physical Review B* **104**, 214403 (2021). 2108.02159.

[13] Pan, H. & Sarma, S. D. Interaction range and temperature dependence of symmetry breaking in strongly correlated two-dimensional moir\'e transition metal dichalcogenide bilayers. *Physical Review B* **105**, 041109 (2022). 2110.11330.

[14] Zeng, Y., Xue, F. & MacDonald, A. H. In-plane magnetic field induced density wave states near quantum spin Hall phase transitions. *Physical Review B* **105**, 125102 (2022). 2112.07523.

[15] Adhikari, K., Seo, K., Beach, K. S. D. & Uchoa, B. Strongly Interacting Phases in Twisted Bilayer Graphene at the Magic Angle (2023). 2308.03843.

[16] Liu, X., Wang, C., Zhang, X.-W., Cao, T. & Xiao, D. Gate-tunable antiferromagnetic Chern insulator in twisted bilayer transition metal dichalcogenides (2023). 2308.07488.

[17] Codebase. URL `https://github.com/KimGroup/HartreeFock_GPT`.

[18] Brown, T. *et al.* Language models are few-shot learners. In *Advances in Neural Information Processing Systems*, vol. 33, 1877–1901 (2020).

[19] Lu, Y., Yang, X., Li, X., Wang, X. E. & Wang, W. Y. Llmscore: Unveiling the power of large language models in text-to-image synthesis evaluation. *arXiv preprint arXiv:2305.11116* (2023).

[20] Chevalier, A. *et al.* Language models as science tutors. *arXiv preprint arXiv:2402.11111* (2024).

[21] Lin, S., Hilton, J. & Evans, O. Teaching models to express their uncertainty in words. *arXiv preprint arXiv:2205.14334* (2022).
